# Supplementary material for: DiffVQA: Video Quality Assessment Using Diffusion Feature Extractor
Source: arXiv:2505.03261 source file (2025-05-06)
Supplement: Supplementary file 1 [file supp_tex.tex]

%%%%%%%%% BODY TEXT
\section{Illustration of \name{}}
As illustrated in \figref{fig:diffusion_features}, we adapt the pre-trained Stable Diffusion model~\cite{rombach2022high} with a Controller module~\cite{zhang2023adding}, ensuring that the diffusion model is capable of reconstructing images identical to the input during training.

After adaptation, the diffusion model is employed to extract features from video frames. For each input image, the text input is set to null, and the image is encoded into a latent feature \( z_{0} \). Noise is then added to \( z_{0} \), initiating the reverse denoising process over \( T \) steps. Using spaced-DDPM sampling~\cite{nichol2021improved}, the process begins at \( t = T \) and iteratively proceeds to \( t = 0 \) (the final step).

The outputs of the diffusion feature extractor consist of multi-scale features from the denoising network at \( t = 0 \) and the reconstructed latent feature \( \hat{z}_0 \), as depicted in \figref{fig:diffusion_features}. In subsequent sections, we refer to these features as \( \text{F}_{\text{MS}} \) and \( \text{F}_{\text{Latent}} \), respectively.

Our design is inspired by the findings presented in \tabref{tab:dff_features} and \tabref{tab:sd_extractor}, which highlight that adapting the diffusion model with a controller to reconstruct identical inputs makes the extracted diffusion features more suitable for VQA compared to directly using the pre-trained Stable Diffusion model. Additionally, leveraging both \(\text{F}_{\text{MS}}\) and \(\text{F}_{\text{Latent}}\) provides superior feature representations for VQA, outperforming other feature selection strategies.

\section{More Experiments}

\subsection{Evaluation on Maxwell dataset}
We evaluate \name{} on the Maxwell dataset~\cite{wu2023exploring} to assess its capability in analyzing multi-dimensional video quality attributes characteristic of in-the-wild content. The Maxwell dataset provides a comprehensive evaluation framework by assessing video quality through a combination of technical and aesthetic attributes. 

On the technical side, the attributes address various factors impacting video clarity and stability. Low sharpness (T-1) refers to videos with unclear textures, while out-of-focus issues (T-2) describe scenarios where the primary target, such as a person in a portrait video, appears blurred due to being out of focus. Noise (T-3) captures random variations in pixel brightness or color, and motion blur (T-4) arises from the movements of the camera or subjects during recording. Flicker (T-5) highlights non-smooth transitions between adjacent frames, while poor exposure (T-6) pertains to regions that are unrecognizable due to excessively low or high brightness. Compression artifacts (T-7) denote distortions, such as blocky or moiré patterns, introduced by compression algorithms~\cite{jpeg,h264}, and low fluency (T-8) indicates missing frames in a sequence of motion.

On the aesthetic front, the dataset considers content appeal (A-1), which evaluates the overall engagement and attractiveness of the video content. Composition (A-2) assesses the organization and balance of objects and scenes within the frame. Color (A-3) measures the vibrancy and pleasantness of the color scheme, while lighting (A-4) evaluates the use of contrastive and visually appealing illumination. Lastly, trajectory (A-5) examines the temporal consistency of the camera's movement, ensuring it aligns harmoniously with the scene being captured.

As summarized in~\tabref{tab:maxwell-all}, \name{} demonstrated promising performance, achieving the highest scores in Technical and Aesthetic categories, as well as the Overall Quality Score, outperforming other state-of-the-art methods.

\begin{figure}[t!]
    \centering
    \hspace{-0.5cm}\includegraphics[width=1.05\linewidth]{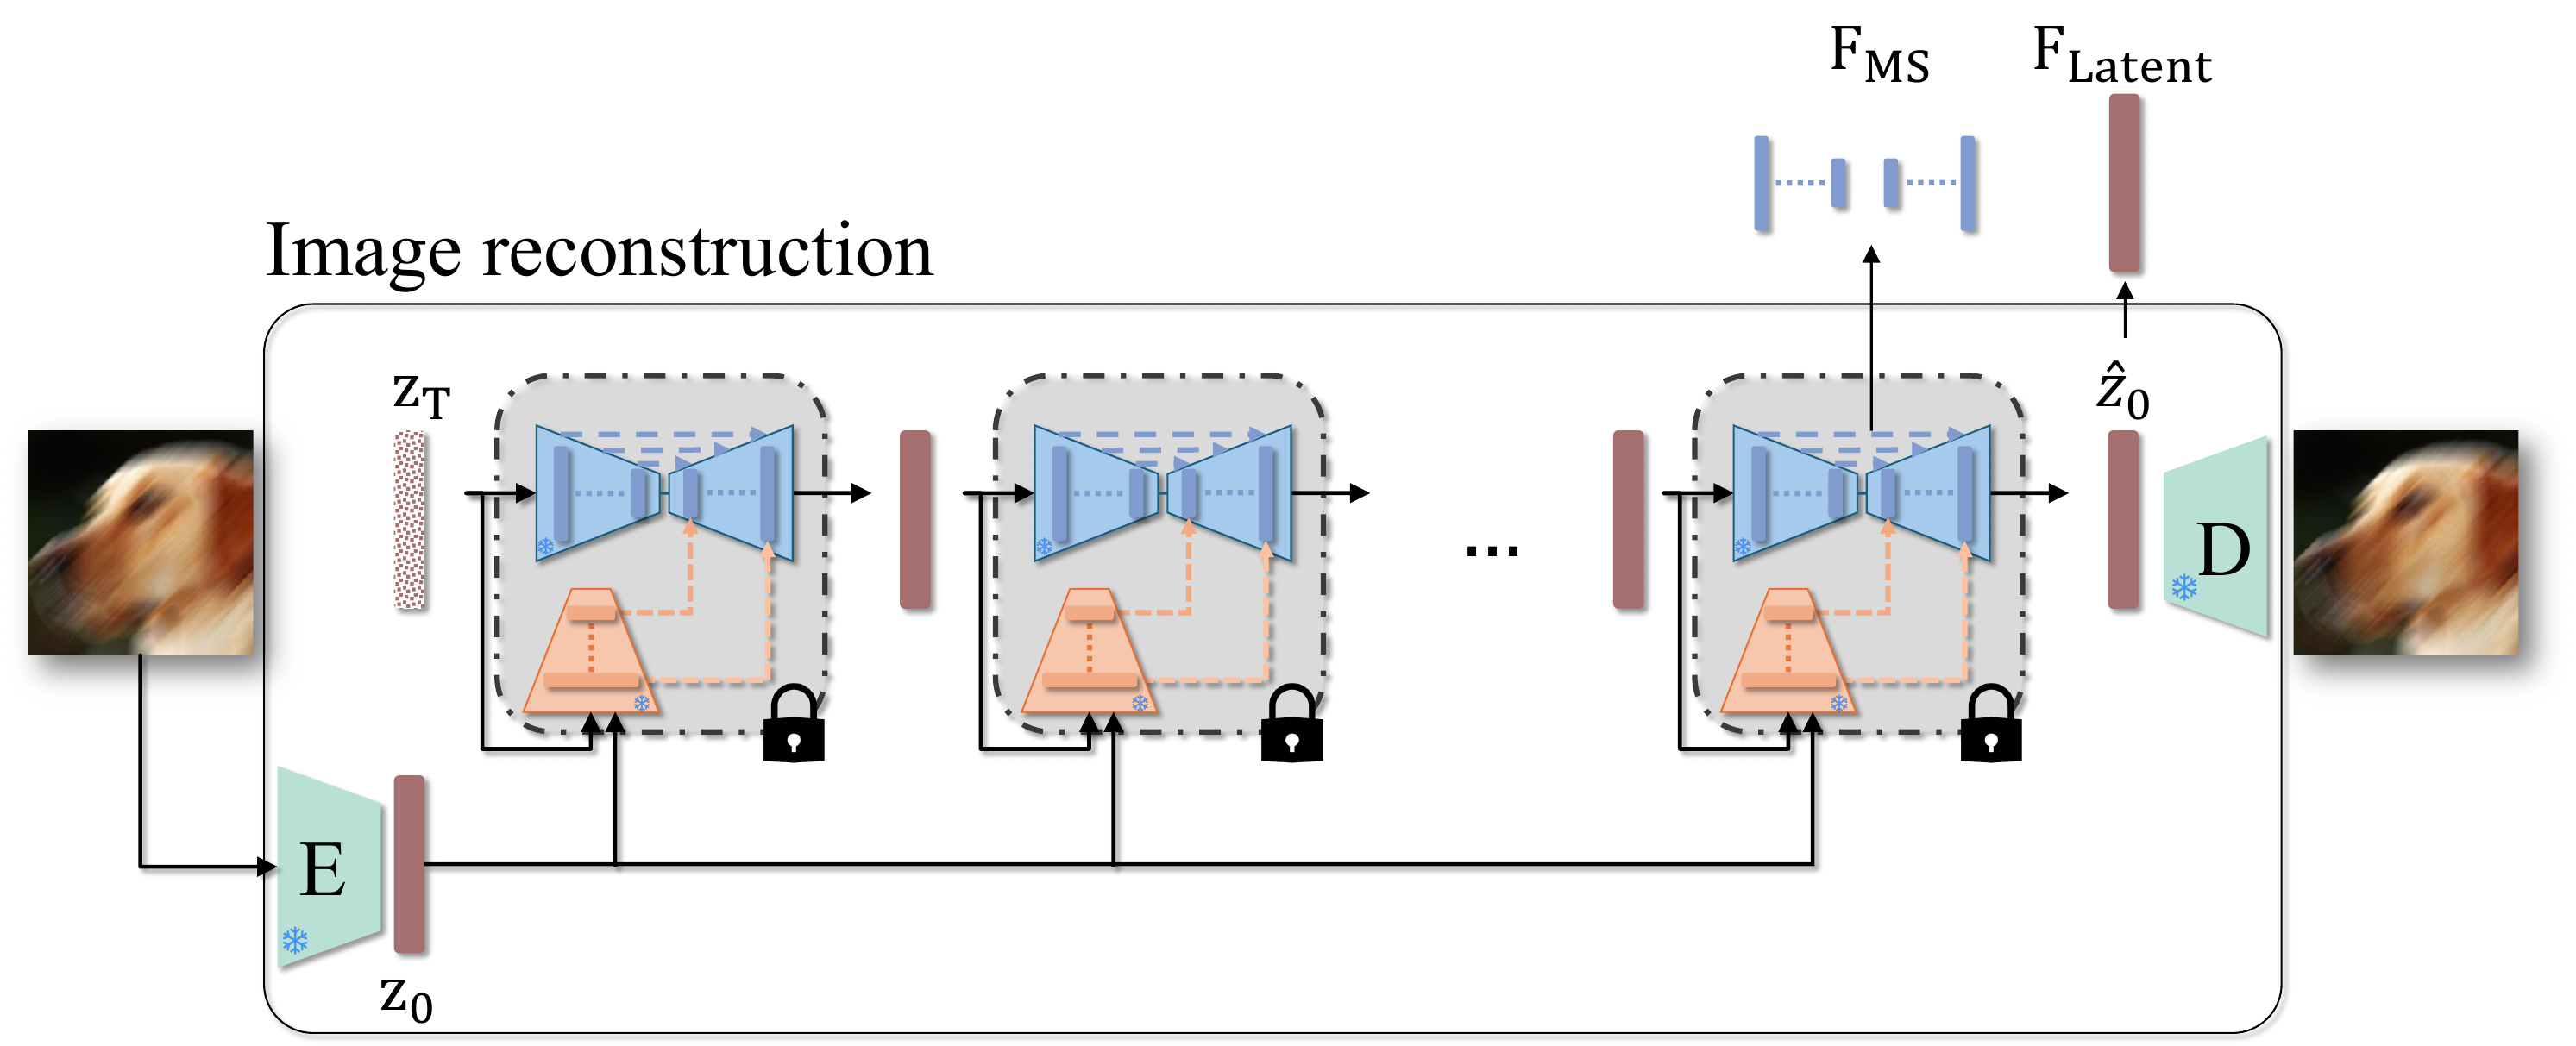}
\caption{\textbf{Details of the Diffusion Feature Extractor} (detailed version of main paper's Figure 3 (c)).}
    \label{fig:diffusion_features}
\end{figure}

\begin{table*}
\footnotesize
\centering
\resizebox{\linewidth}{!}{\begin{tabular}{l|c|c|c|c|c|c|c|c|c|c|c|c|c|c|c|c}
\hline
   Dimensions (\textit{in codes})  & A-1 & A-2 & A-3 & A-4 & A-5 & A-all & T-1 & T-2 & T-3 & T-4 & T-5 & T-6 & T-7 & T-8 & T-all & O    \\ \hline
  Methods           & PLCC     & PLCC   & PLCC   & PLCC   & PLCC   & PLCC   & PLCC   & PLCC   & PLCC   & PLCC   & PLCC   & PLCC   & PLCC   & PLCC   & PLCC   & PLCC  \\ \hline 

NIQE \cite{mittal2012making} & 0.317 & 0.281 & 0.329 & 0.321 & 0.211 & 0.338 & 0.189 & 0.255 & 0.174 & 0.217 & 0.136 & 0.199 & 0.156 & 0.178 & 0.255 & 0.301 \\
TPQI~\cite{liao2022exploring} & 0.246 & 0.293 & 0.210 & 0.225 & 0.360 & 0.319 & 0.223 & 0.293 & 0.239 & 0.374 & 0.463 & 0.225 & 0.244 & 0.410 & 0.363 & 0.361 \\
SAQI~\cite{wu2023bvqi} & 0.388 & 0.410 & 0.453 & 0.504 & 0.393 & 0.515 & 0.560 & 0.500 & 0.524 & 0.509 & 0.344 & 0.482 & 0.497 & 0.311 & 0.554 & 0.559\\

TLVQM \cite{korhonen2019two}  &0.477 & 0.523 & 0.437 & 0.471 & 0.601 & 0.590 & 0.537 & 0.571 & 0.538 & 0.606 & 0.664 & 0.503 & 0.539 & 0.530 & 0.653 & 0.652  \\

VIDEVAL \cite{tu2021ugc} & 0.469 & 0.533 & 0.501 & 0.513 & 0.533 & 0.564 &  0.578 & 0.534 & 0.548 &0.557 & 0.664 &  0.467 & 0.543 & 0.393 & 0.595 & 0.601        \\ 
RAPIQUE \cite{tu2021rapique}&0.490 & 0.538 & 0.520 & 0.559 & 0.560 & 0.651 & 0.610 & 0.618 & 0.588 & 0.621 & 0.563 & 0.568 & 0.566 & 0.406 & 0.695 & 0.708  \\ 
 VSFA \cite{li2018has}    & 0.512 & 0.556 & 0.611 & 0.634 & 0.515 & 0.624 & 0.719 & 0.625 & 0.642 & 0.612 & 0.555 & 0.645 &  0.643 & 0.406 & 0.672 & 0.678 \\
BVQA \cite{li2021unified} & 0.553 & 0.607 & 0.659 & 0.668 & 0.678 & 0.671 & 0.746 & 0.686 & 0.694 & 0.682 & 0.781 &0.653 & 0.677 & 0.659 &0.759 & 0.739 \\ 

FAST-VQA \cite{wu2022fast} & 0.614 & 0.630 & 0.696 & 0.709 & 0.646 & 0.721 & 0.800 & 0.724 & 0.755 & 0.731 & 0.751 & 0.695 & 0.736 & 0.654 & 0.803 & 0.782 \\ 

MaxVQA~\cite{wu2023towards} & \underline{0.681} & \underline{0.701} & \underline{0.757} & \underline{0.749} & \underline{0.712} & \underline{0.775} & \underline{0.825} & \underline{0.748} & \underline{0.776} & \underline{0.761} & \underline{0.782} & \underline{0.748} & \underline{0.763} & \underline{0.684} & \underline{0.827} & \underline{0.813} \\

\hline
\textbf{\name{}} & \textbf{0.694} & \textbf{0.710} & \textbf{0.769} & \textbf{0.772} & \textbf{0.733} & \textbf{0.794} & \textbf{0.838} & \textbf{0.766} & \textbf{0.790} & \textbf{0.767} & \textbf{0.789} & \textbf{0.762} & \textbf{0.778} & \textbf{0.690} & \textbf{0.843} & \textbf{0.840} \\
\hline
\end{tabular}}
\caption{\textbf{Benchmarking of \name{} against existing methods on the Maxwell dataset~\cite{wu2023towards} across multiple dimensions.}}
\label{tab:maxwell-all}
\end{table*}

\begin{table}[t!]
    \centering
    \footnotesize
    \setlength\tabcolsep{6pt}
    
    \begin{tabular}{lcc}
        \hline
        Variant & SRCC$\uparrow$ & PLCC$\uparrow$ \\ 
        \hline
        (i) Only \(\text{F}_{\text{Latent}}\) & 0.820 & 0.799 \\ 
        (ii) Only \(\text{F}_{\text{MS}}\) & 0.891 & 0.879 \\ 
        (iii) \jw{Encoder-\(\text{F}_{\text{MS}} + \text{F}_{\text{Latent}}\) } & 0.872 & 0.863 \\ 
        (iv) Decoder-\(\text{F}_{\text{MS}} + \text{F}_{\text{Latent}}\) & 0.885 & 0.871 \\ 
        (v) Controller Multi-Scale Features & 0.604 & 0.627 \\ 
        (vi) ALL (\jw{\(\text{F}_{\text{MS}} + \text{F}_{\text{Latent}}\)}) & \textbf{0.912} & \textbf{0.915} \\ 
        \hline
    \end{tabular}
    \caption{\textbf{Comparison of VQA performance using different features as inputs to the Diffusion Feature Fusion module.} The results demonstrate that the selected features in \name{} (\jw{\(\text{F}_{\text{MS}} + \text{F}_{\text{Latent}}\)}) achieve the best performance.}
        \label{tab:dff_features}

\end{table}

\begin{table}[t!]
\centering
\scalebox{0.9}{
\begin{tabular}{lcc}
\toprule
SD w. Different Noise Level  & SRCC & PLCC \\ 
\midrule
SD ($t=1000$) & 0.723 & 0.717 \\
SD ($t=100$)  & 0.791 & 0.796 \\
SD ($t=10$)   & 0.835 & 0.827 \\
SD ($t=1$)    & 0.854 & 0.852 \\
% \hline
\midrule
\name{} & \textbf{0.912} & \textbf{0.915} \\
\bottomrule
\end{tabular}}
\caption{\textbf{\jw{Performance comparison of SRCC and PLCC between the naïve feature extractor by using the pre-trained Stable Diffusion Model without adaptation at different noise levels (\(t = 1000, 100, 10, 1\)) and \name{}.}} Results demonstrate that increasing noise steps degrades VQA performance due to reduced feature relevance. \name{} achieves the highest performance by leveraging adapted diffusion features.}
 \label{tab:sd_extractor}

\end{table}

\begin{table}[t!]
\centering
\scalebox{0.9}{
\begin{tabular}{lcc}
\toprule
\( \jw{z_T} \) Initialization Method & SRCC $\uparrow$ & PLCC $\uparrow$ \\
\midrule
From random noise                      & 0.904                    & 0.889                    \\
From \( z_0 \) with added noise        & \textbf{0.912}           & \textbf{0.915}           \\
\bottomrule
\end{tabular}}
\caption{\textbf{Impact of different \( z_T \) initializations on VQA performance.} Comparison between \( z_T \) derived from \( z_0 \) with added noise for \( T = 1000 \) steps and \( z_T \) initialized from random noise. Results demonstrate that using \( z_T \) derived from \( z_0 \) achieves better VQA performance.}
\label{tab:zt_initialization}

\end{table}

\begin{figure*}[htbp]
    \centering
    % First row of subfigures
    \begin{subfigure}[b]{0.16\textwidth}
        \centering
        \includegraphics[width=\textwidth]{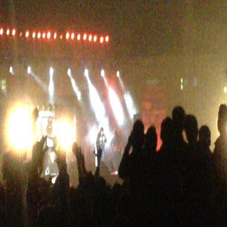}
        \includegraphics[width=\textwidth]{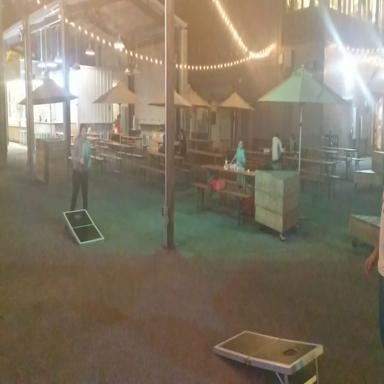}
        \caption{Input}
    \end{subfigure}
    \begin{subfigure}[b]{0.16\textwidth}
        \centering
        \includegraphics[width=\textwidth]{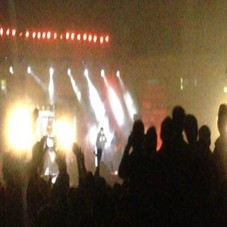}
        \includegraphics[width=\textwidth]{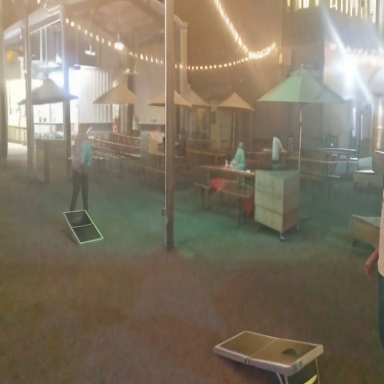}
        \caption{\jw{SD (\(t=1\))}}
    \end{subfigure}
    \begin{subfigure}[b]{0.16\textwidth}
        \centering
        \includegraphics[width=\textwidth]{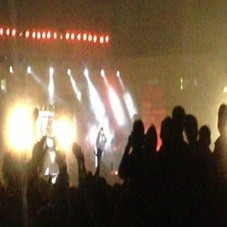}
        \includegraphics[width=\textwidth]{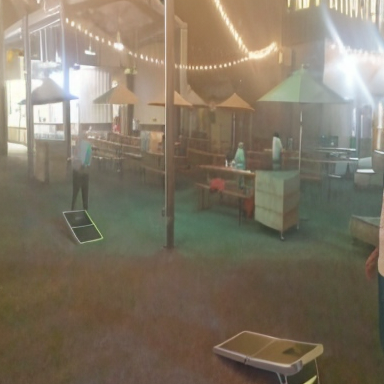}
        \caption{SD (\(t=10\))}
    \end{subfigure}
    \begin{subfigure}[b]{0.16\textwidth}
        \centering
        \includegraphics[width=\textwidth]{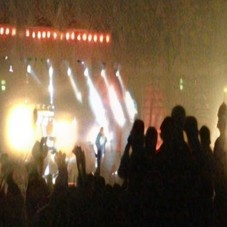}
        \includegraphics[width=\textwidth]{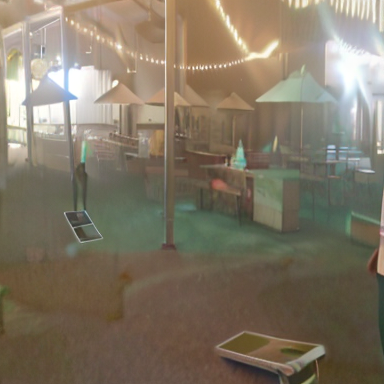}
        \caption{SD (\(t=100\))}
    \end{subfigure}
    \begin{subfigure}[b]{0.16\textwidth}
        \centering
        \includegraphics[width=\textwidth]{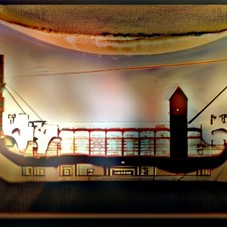}
        \includegraphics[width=\textwidth]{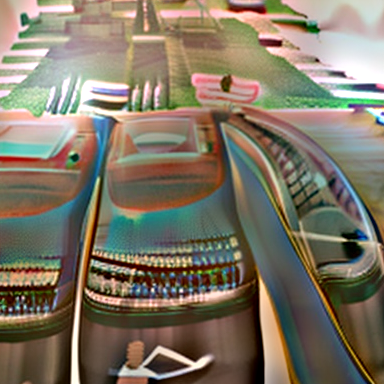}
        \caption{SD (\(t=1000\))}
    \end{subfigure}
    \begin{subfigure}[b]{0.16\textwidth}
        \centering
        \includegraphics[width=\textwidth]{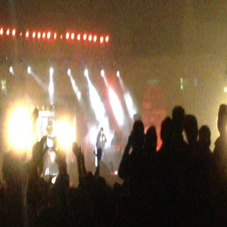}
        \includegraphics[width=\textwidth]{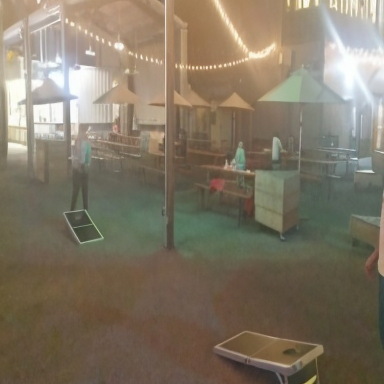}
        \caption{\name{}}
    \end{subfigure}
    % Caption for the entire figure
    \caption{\textbf{Visualization of reconstructed frames  \jw{using the pre-trained Stable Diffusion without adaptation at various noise levels (\(t=1, 10, 100, 1000\)) and \name{}}.} When \(t=1\) or \(t=10\), the reconstructed frames retain good quality; however, starting from \(t=100\), distortions begin to degrade the reconstruction fidelity, as seen in the first row of (d), particularly in the upper-right corner. By \(t=1000\), the reconstructed frames lose significant semantic and distortion information, highlighting the diminishing fidelity at higher noise levels.}
    \label{fig:noise_reconstruction}
\end{figure*}

\subsection{Ablation Study}
\label{sec:ablation}
We conduct more experiments to validate the effectiveness of the \name{} model, all of which are performed using the LIVE-VQC dataset \cite{hosu2017konstanz}.

\noindent\textbf{Feature Selection in DFF.}
We validate the effectiveness of using different features from the diffusion feature extractor as inputs to the Diffusion Feature Fusion (DFF) module by creating several variants of our approach. These variants include: 
(i) using only \(\text{F}_{\text{Latent}}\), 
(ii) using only \(\text{F}_{\text{MS}}\), 
(iii) using only the encoder features from \(\text{F}_{\text{MS}}\) combined with \(\text{F}_{\text{Latent}}\), 
(iv) using only the decoder features from \(\text{F}_{\text{MS}}\) combined with \(\text{F}_{\text{Latent}}\), where the decoder features from \(\text{F}_{\text{MS}}\) consist of the denoising U-Net's decoder features combined with the Controller's multi-scale features, 
(v) using only the multi-scale features from the Controller, and 
(vi) the selected features in \name{} (\jw{ \(\text{F}_{\text{MS}} + \text{F}_{\text{Latent}}\)}). 

The results, presented in \tabref{tab:dff_features}, demonstrate that the selected features in \name{} achieve the best VQA performance, confirming the efficacy of our feature selection approach. Among the other feature selection approaches, we observe that using the complete \(\text{F}_{\text{MS}}\) yields the best performance compared to using only \(\text{F}_{\text{Latent}}\). This is because \(\text{F}_{\text{MS}}\) captures both rich low-level and high-level information. Within \(\text{F}_{\text{MS}}\), using only the decoder features performs better than using only the encoder features. We attribute this to the decoder features incorporating the Controller's additional information, which provides complementary insights beyond the encoder's features. However, using only the Controller's features for VQA results in the most limited performance. This is likely because the Controller primarily provides auxiliary control signals aimed at reconstructing the input frames, which are not the dominant factors in VQA tasks. Nevertheless, combining the Controller's features into \(\text{F}_{\text{MS}}\) improves VQA performance, as the Controller supplements \(\text{F}_{\text{MS}}\) with additional information that compensates for its limitations.

\noindent\textbf{Necessity of Adaption.}
We conduct an additional experiment to validate the importance of adapting the diffusion model by reconstructing images identical to the input. Specifically, we use the naïve feature extractor based on the pre-trained Stable Diffusion model (SD) without any adaptation or Controller module to extract features for VQA. 
For this experiment, the input frame is encoded into the latent feature \( z_0 \) using the pre-trained autoencoder of SD. Different levels of noise are added to \( z_0 \) at \( t=1, 10, 100, 1000 \) (where \( t=1000 \) represents the total step $T$ in this paper), resulting in \( z_1, z_{10}, z_{100}, z_{1000} \). These noisy latent features are then passed through the reverse diffusion process to reconstruct \( \hat{z}_0 \). The features at \( t=0 \) (final step), including \( \text{F}_{\text{MS}} \) and \( \text{F}_{\text{Latent}} \), are extracted as the outputs of the diffusion feature extractor, consistent with those used in \name{}.

The results, presented in \tabref{tab:sd_extractor}, demonstrate that the performance of VQA is degraded when features are extracted from an unadapted SD model without a Controller module. This is primarily because \( \text{F}_{\text{MS}} \), derived from the original \( z_0 \) through the denoising U-Net, is not inherently tailored for VQA tasks. In contrast, adapting SD with the Controller module, which enables the reconstruction of identical input frames, ensures that \( \text{F}_{\text{MS}} \) becomes more suitable for VQA applications. Furthermore, we observe that adding more noise steps to \( z_0 \) leads to worse VQA performance. As shown in \figref{fig:noise_reconstruction}, with increasing noise levels, the reconstructed images deviate from the original input due to the absence of the Controller's guidance. This discrepancy results in extracted features that fail to accurately represent the image, thereby diminishing VQA performance.

\noindent\textbf{Different Initialization of \jw{\( z_T \)}.}
In our \name{} framework, the \( z_T \) used is derived by adding noise to \( z_0 \). We conduct experiments to evaluate the impact of using \( z_T \) initialized from random noise instead. The results, presented in \tabref{tab:zt_initialization}, indicate that initializing \( z_T \) with random noise leads to a decline in VQA performance. This finding underscores that deriving \( z_T \) by adding noise to \( z_0 \) enables the denoising U-Net to generate more effective features, ultimately enhancing the performance of VQA.

\section{Datasets}
We evaluate the proposed model on six widely recognized UGC VQA datasets: KoNViD-1k~\cite{hosu2017konstanz}, LIVE-VQC~\cite{hosu2017konstanz}, YouTube-UGC~\cite{wang2019youtube}, LSVQ~\cite{ying2021patch}, KVQ~\cite{lu2024kvq}, and Maxwell~\cite{wu2023exploring}. Examples of video frames from each dataset are shown in \figref{fig:dataset-examples}. The KoNViD-1k dataset contains 1,200 videos sampled from a wide variety of real-world scenes, providing diverse visual content. The LIVE-VQC dataset includes 585 videos captured in authentic settings, focusing on realistic and varied video quality challenges. The YouTube-UGC dataset, comprising 1,147 videos, is notably diverse, spanning 15 video categories such as animation, gaming, HDR, live music, and sports. The LSVQ dataset includes 39,076 videos, making it the largest UGC VQA dataset to date and a vital benchmark for VQA research. The KVQ dataset represents the first large-scale kaleidoscope short-form video database, consisting of 4,200 user-uploaded or processed videos from short-form UGC platforms. The Maxwell dataset contains 4,543 videos covering 16 dimensions, including 13 specific quality factors and 3 abstract quality ratings. It is split into a training set of 3,634 videos and a reserved test set of 909 videos, enabling comprehensive evaluation of multi-dimensional video quality attributes, particularly for dynamic and in-the-wild content.

\begin{figure*}[t]
    \centering
    \begin{subfigure}[b]{0.32\textwidth}
        \centering
        \includegraphics[width=\linewidth]{figures/all_images/dataset_sample/konvid_sample.png}
        \caption{KoNViD-1k}
        \label{fig:konvid-1k}
    \end{subfigure}
    \hfill
    \begin{subfigure}[b]{0.32\textwidth}
        \centering
        \includegraphics[width=\linewidth]{figures/all_images/dataset_sample/livevqc_sample.png}
        \caption{LIVE-VQC}
        \label{fig:live-vqc}
    \end{subfigure}
    \hfill
    \begin{subfigure}[b]{0.32\textwidth}
        \centering
        \includegraphics[width=\linewidth]{figures/all_images/dataset_sample/ytugc_sample.png}
        \caption{YouTube-UGC}
        \label{fig:youtube-ugc}
    \end{subfigure}
    \vspace{1em}
    \begin{subfigure}[b]{0.32\textwidth}
        \centering
        \includegraphics[width=\linewidth]{figures/all_images/dataset_sample/lsvq_sample.png}
        \caption{LSVQ}
        \label{fig:lsvq}
    \end{subfigure}
    \hfill
    \begin{subfigure}[b]{0.32\textwidth}
        \centering
        \includegraphics[width=\linewidth]{figures/all_images/dataset_sample/kvq_sample.png}
        \caption{KVQ}
        \label{fig:kvq}
    \end{subfigure}
    \hfill
    \begin{subfigure}[b]{0.32\textwidth}
        \centering
        \includegraphics[width=\linewidth]{figures/all_images/dataset_sample/maxwell_sample.png}
        \caption{Maxwell}
        \label{fig:maxwell}
    \end{subfigure}
    \caption{\textbf{Examples of video frames from the six evaluated datasets.} Each row contains three columns showing examples from different datasets: (a) KoNViD-1k~\cite{hosu2017konstanz}, (b) LIVE-VQC~\cite{hosu2017konstanz}, (c) YouTube-UGC~\cite{wang2019youtube}, (d) LSVQ~\cite{ying2021patch}, (e) KVQ~\cite{lu2024kvq}, and (f) Maxwell~\cite{wu2023exploring}.}
    \label{fig:dataset-examples}
\end{figure*}

\section{Implementation Details}

\begin{figure*}[t]
    \centering
    % Sharp
    \begin{subfigure}[b]{0.3\textwidth}
        \centering
        \includegraphics[width=\textwidth]{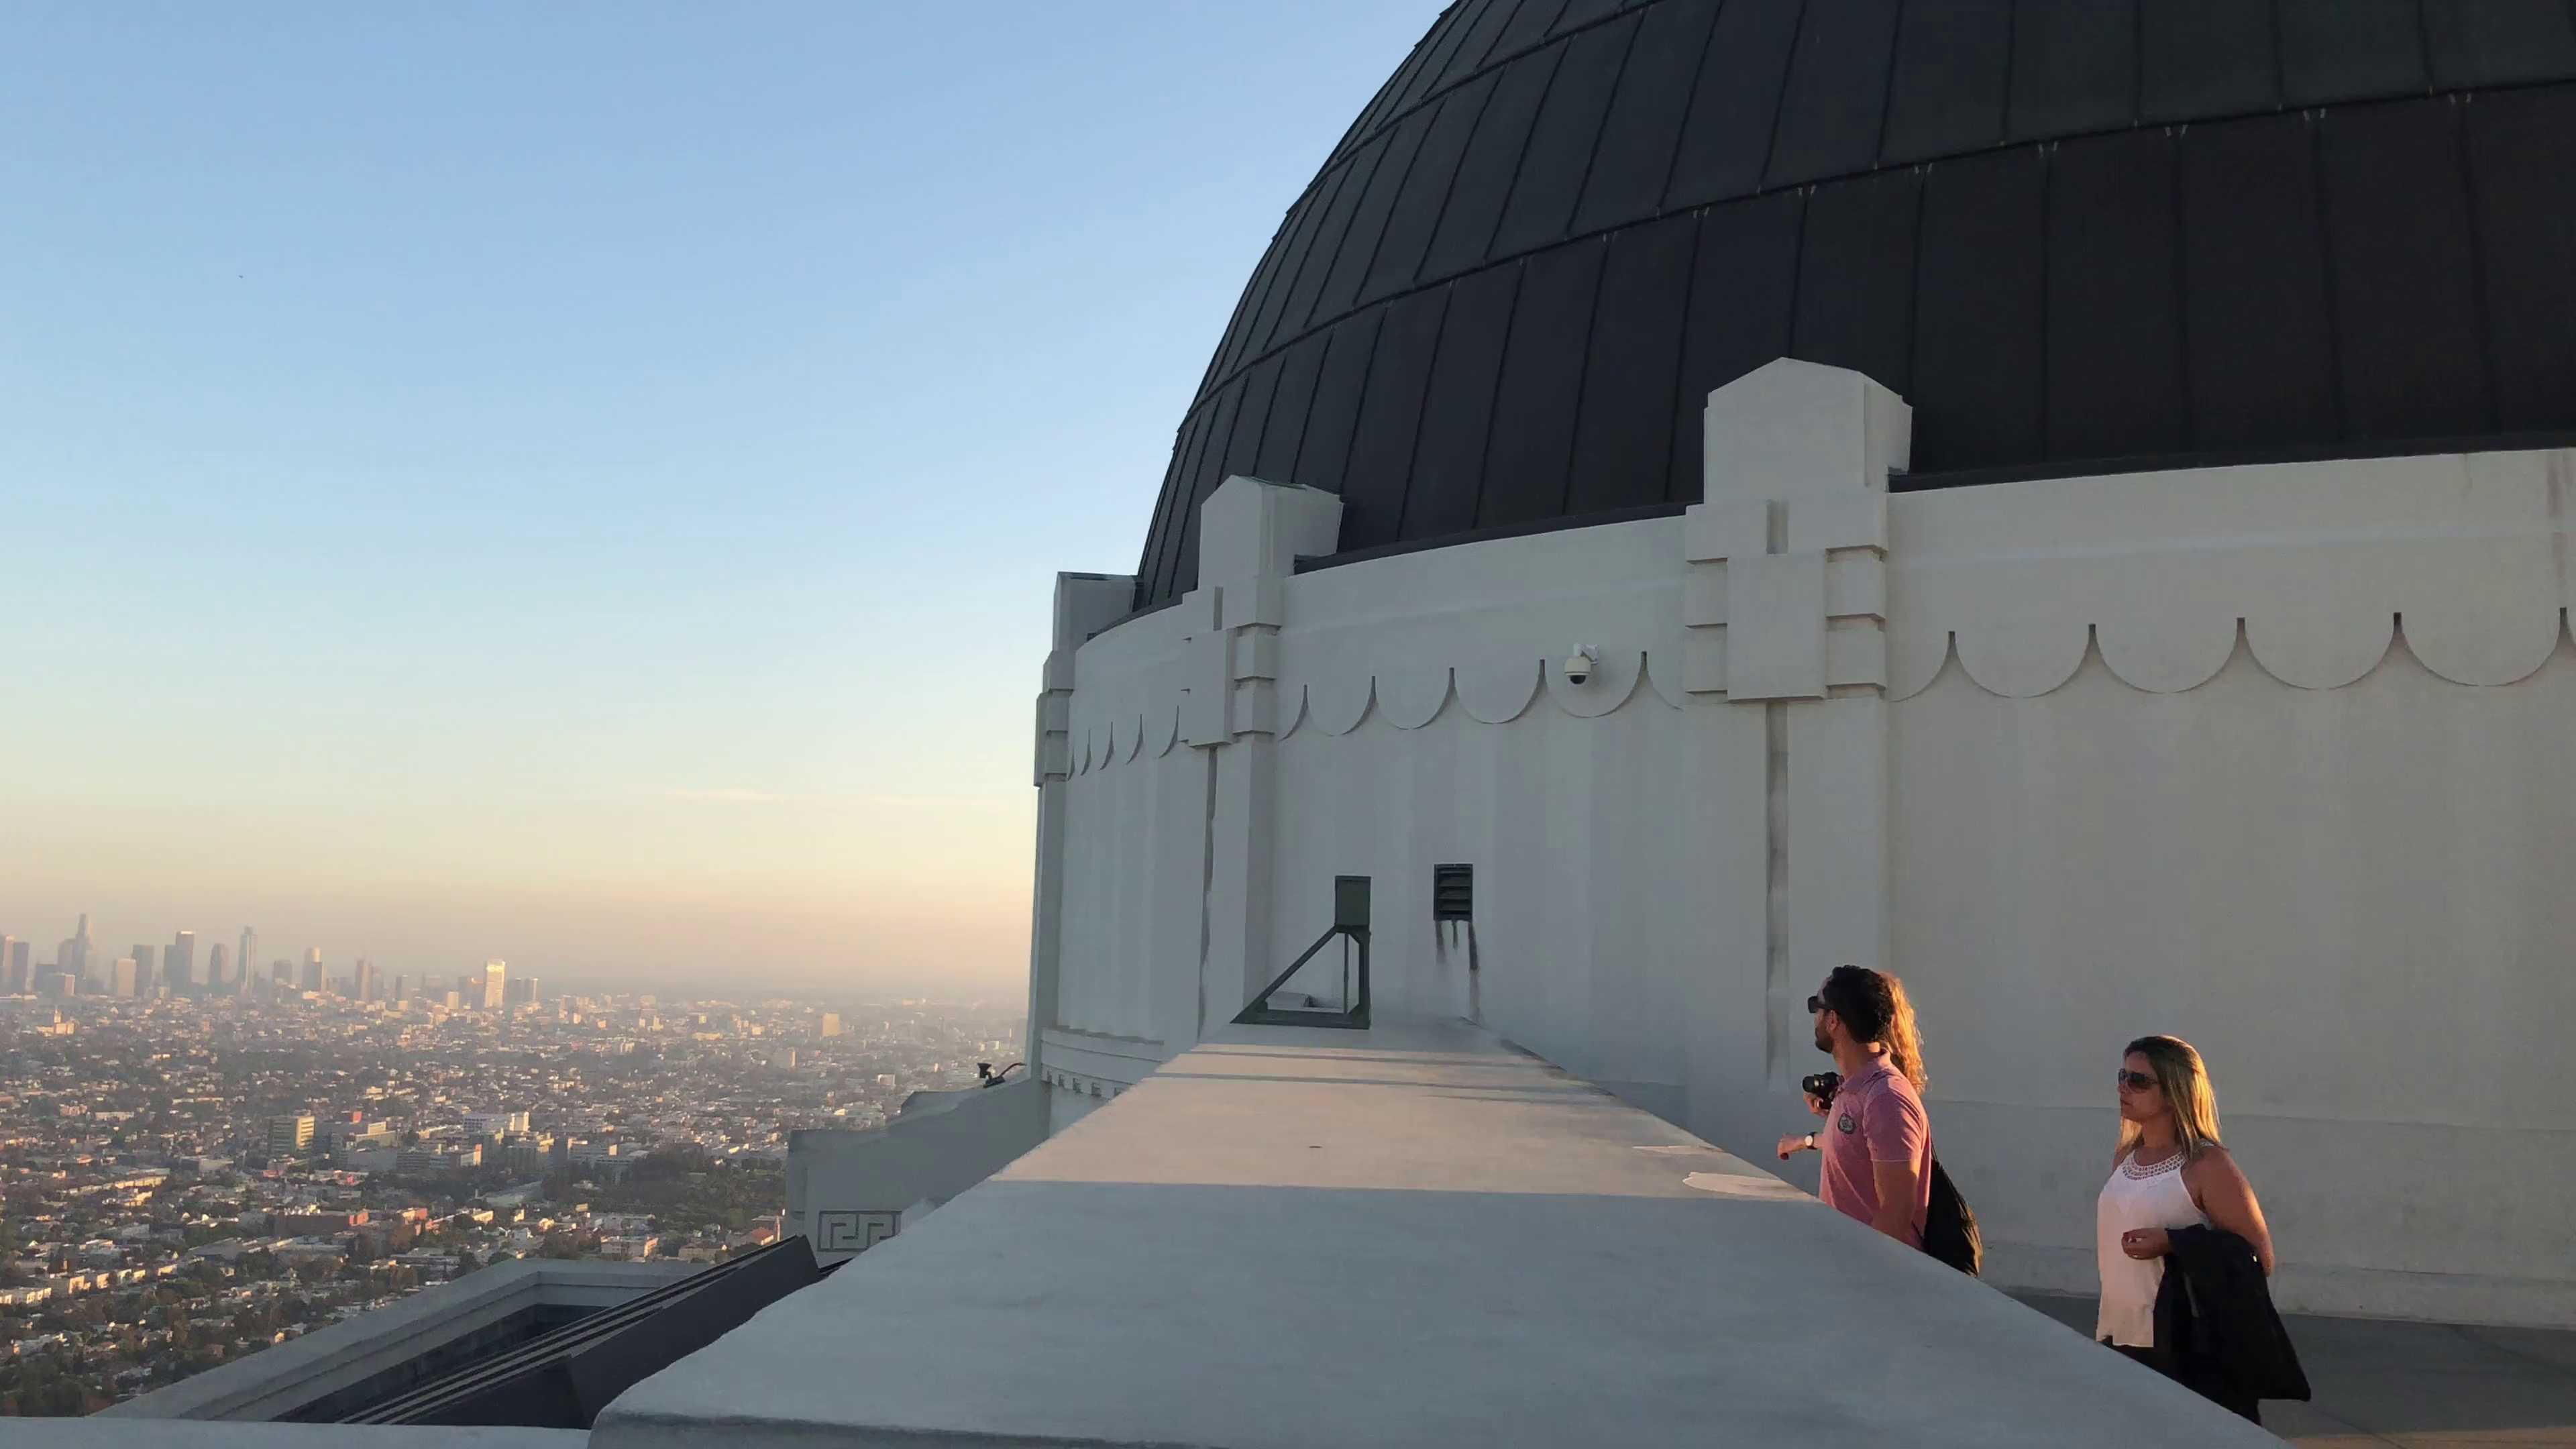}
        \caption{Sharp}
    \end{subfigure}
    % Gaussian Noise
    \begin{subfigure}[b]{0.3\textwidth}
        \centering
        \includegraphics[width=\textwidth]{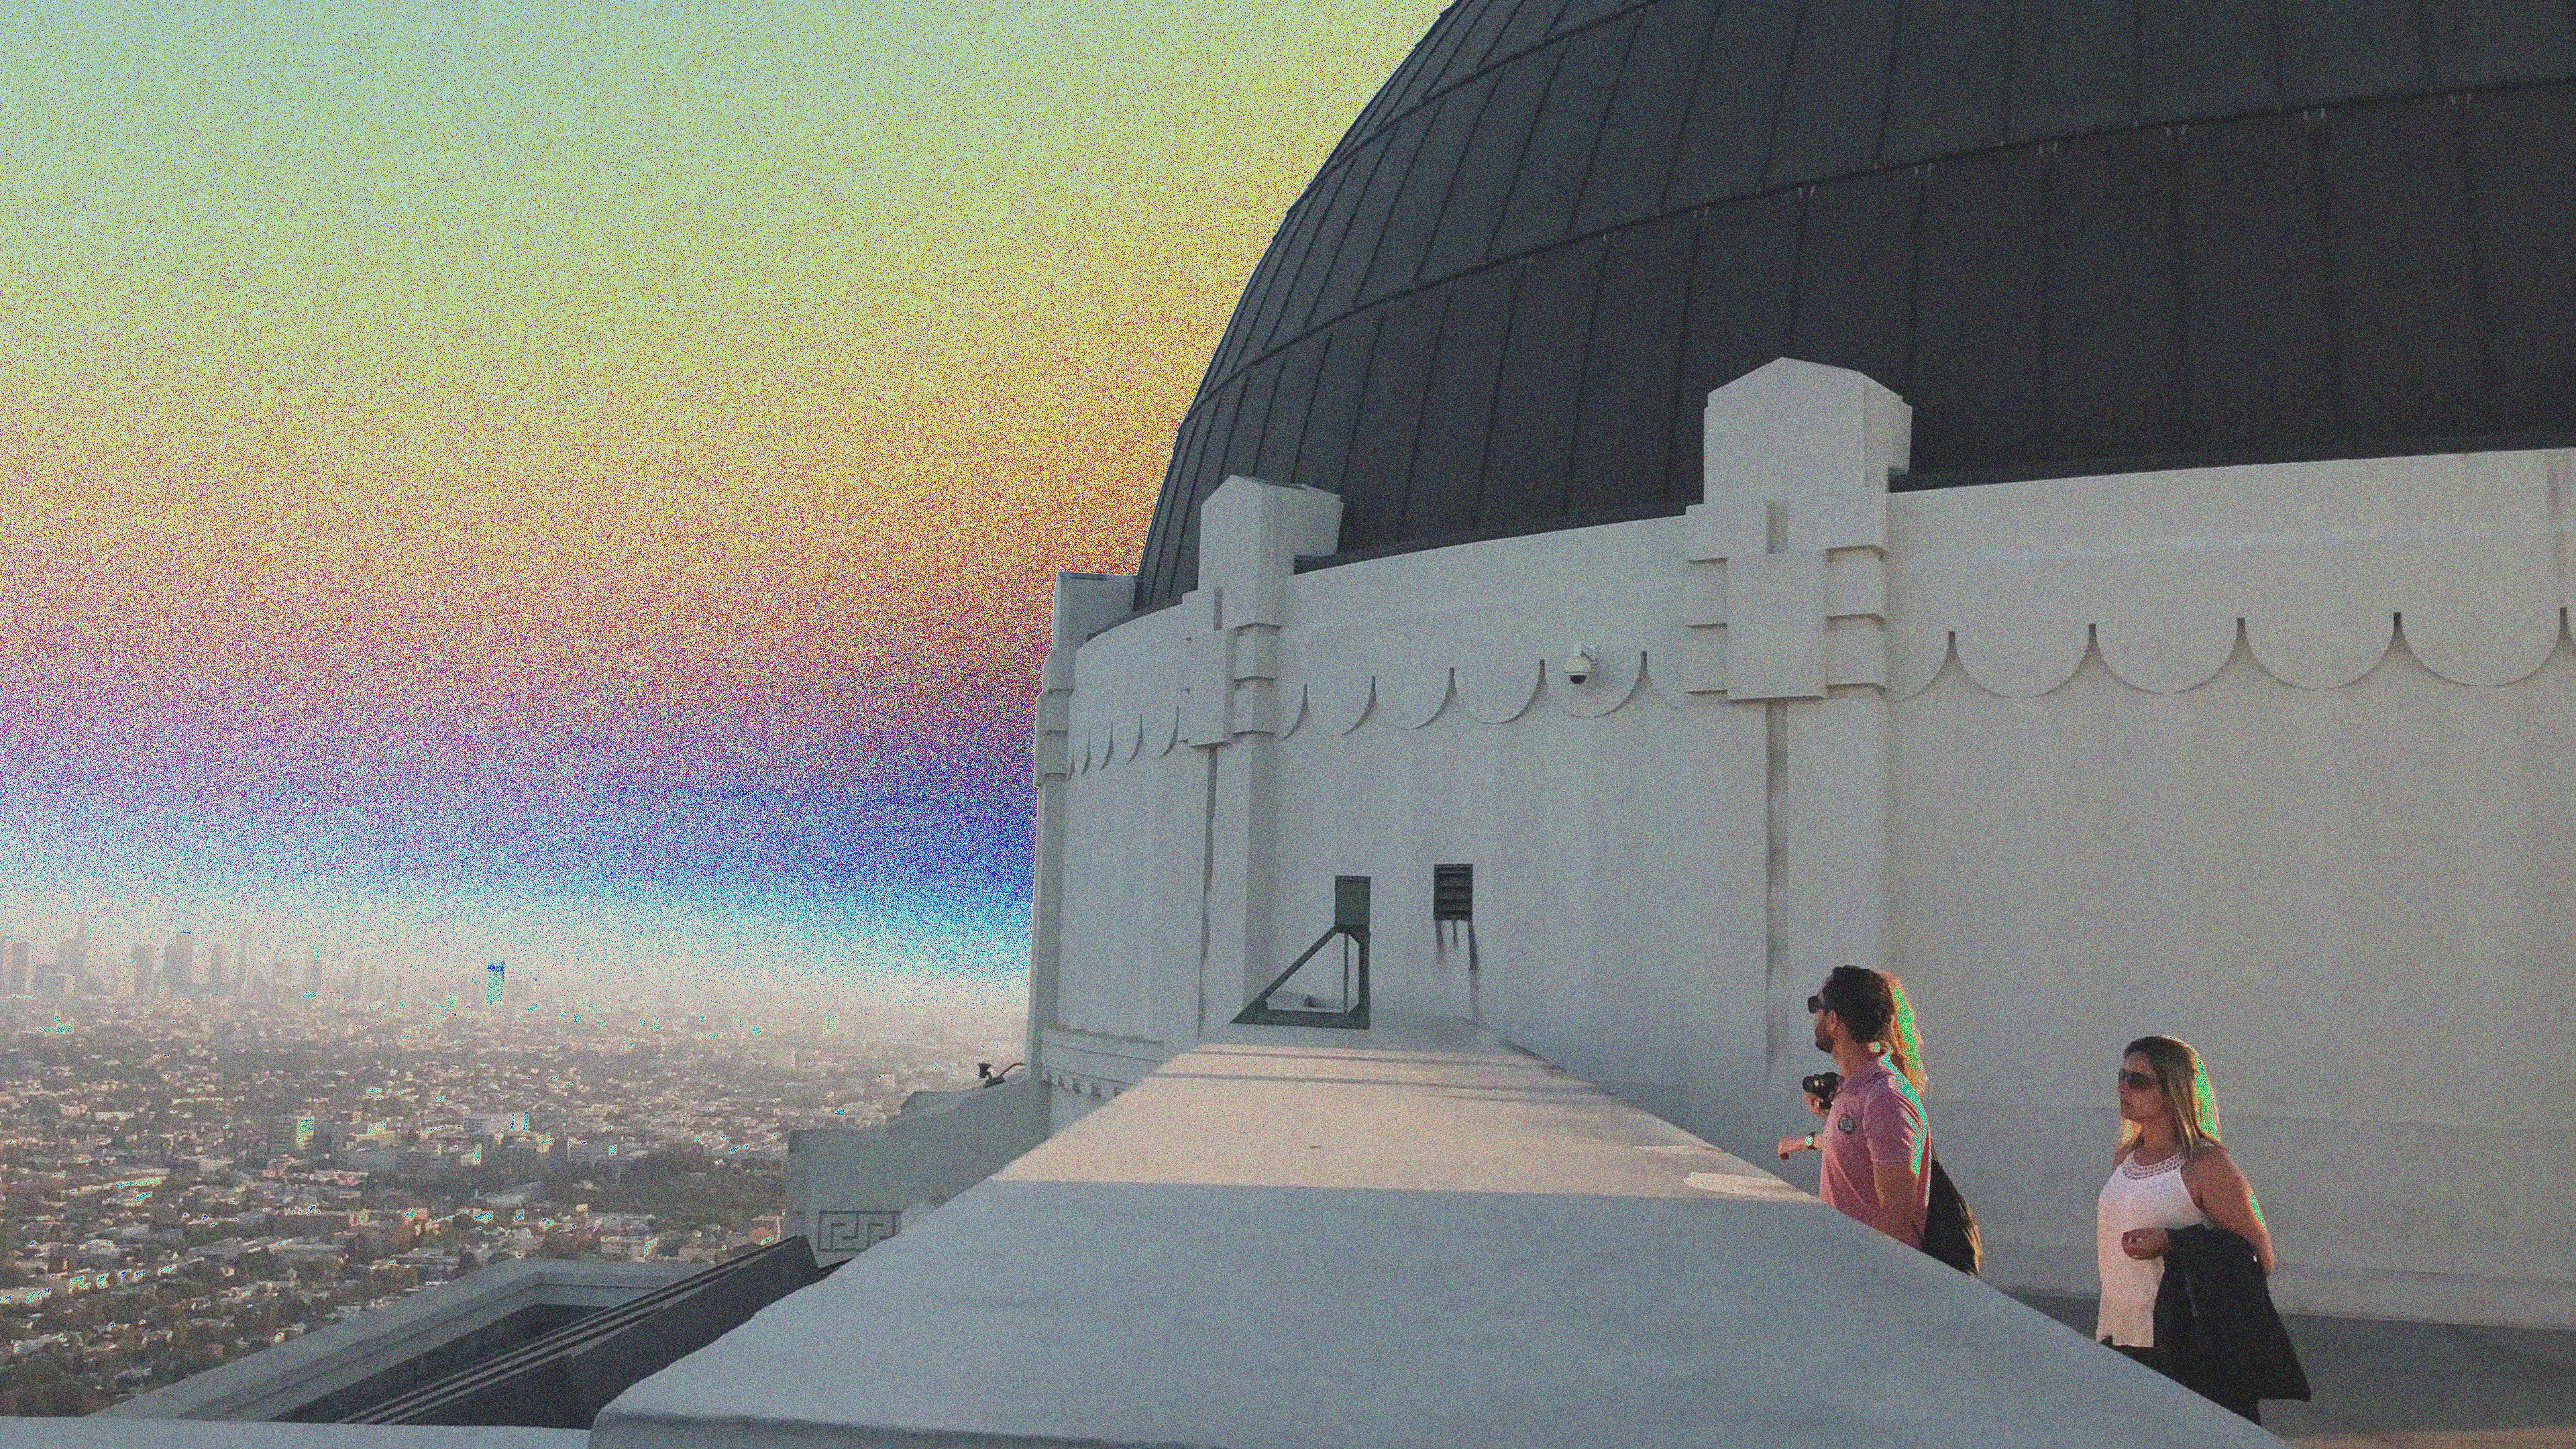}
        \caption{Gaussian Noise}
    \end{subfigure}
    % ISO Noise
    \begin{subfigure}[b]{0.3\textwidth}
        \centering
        \includegraphics[width=\textwidth]{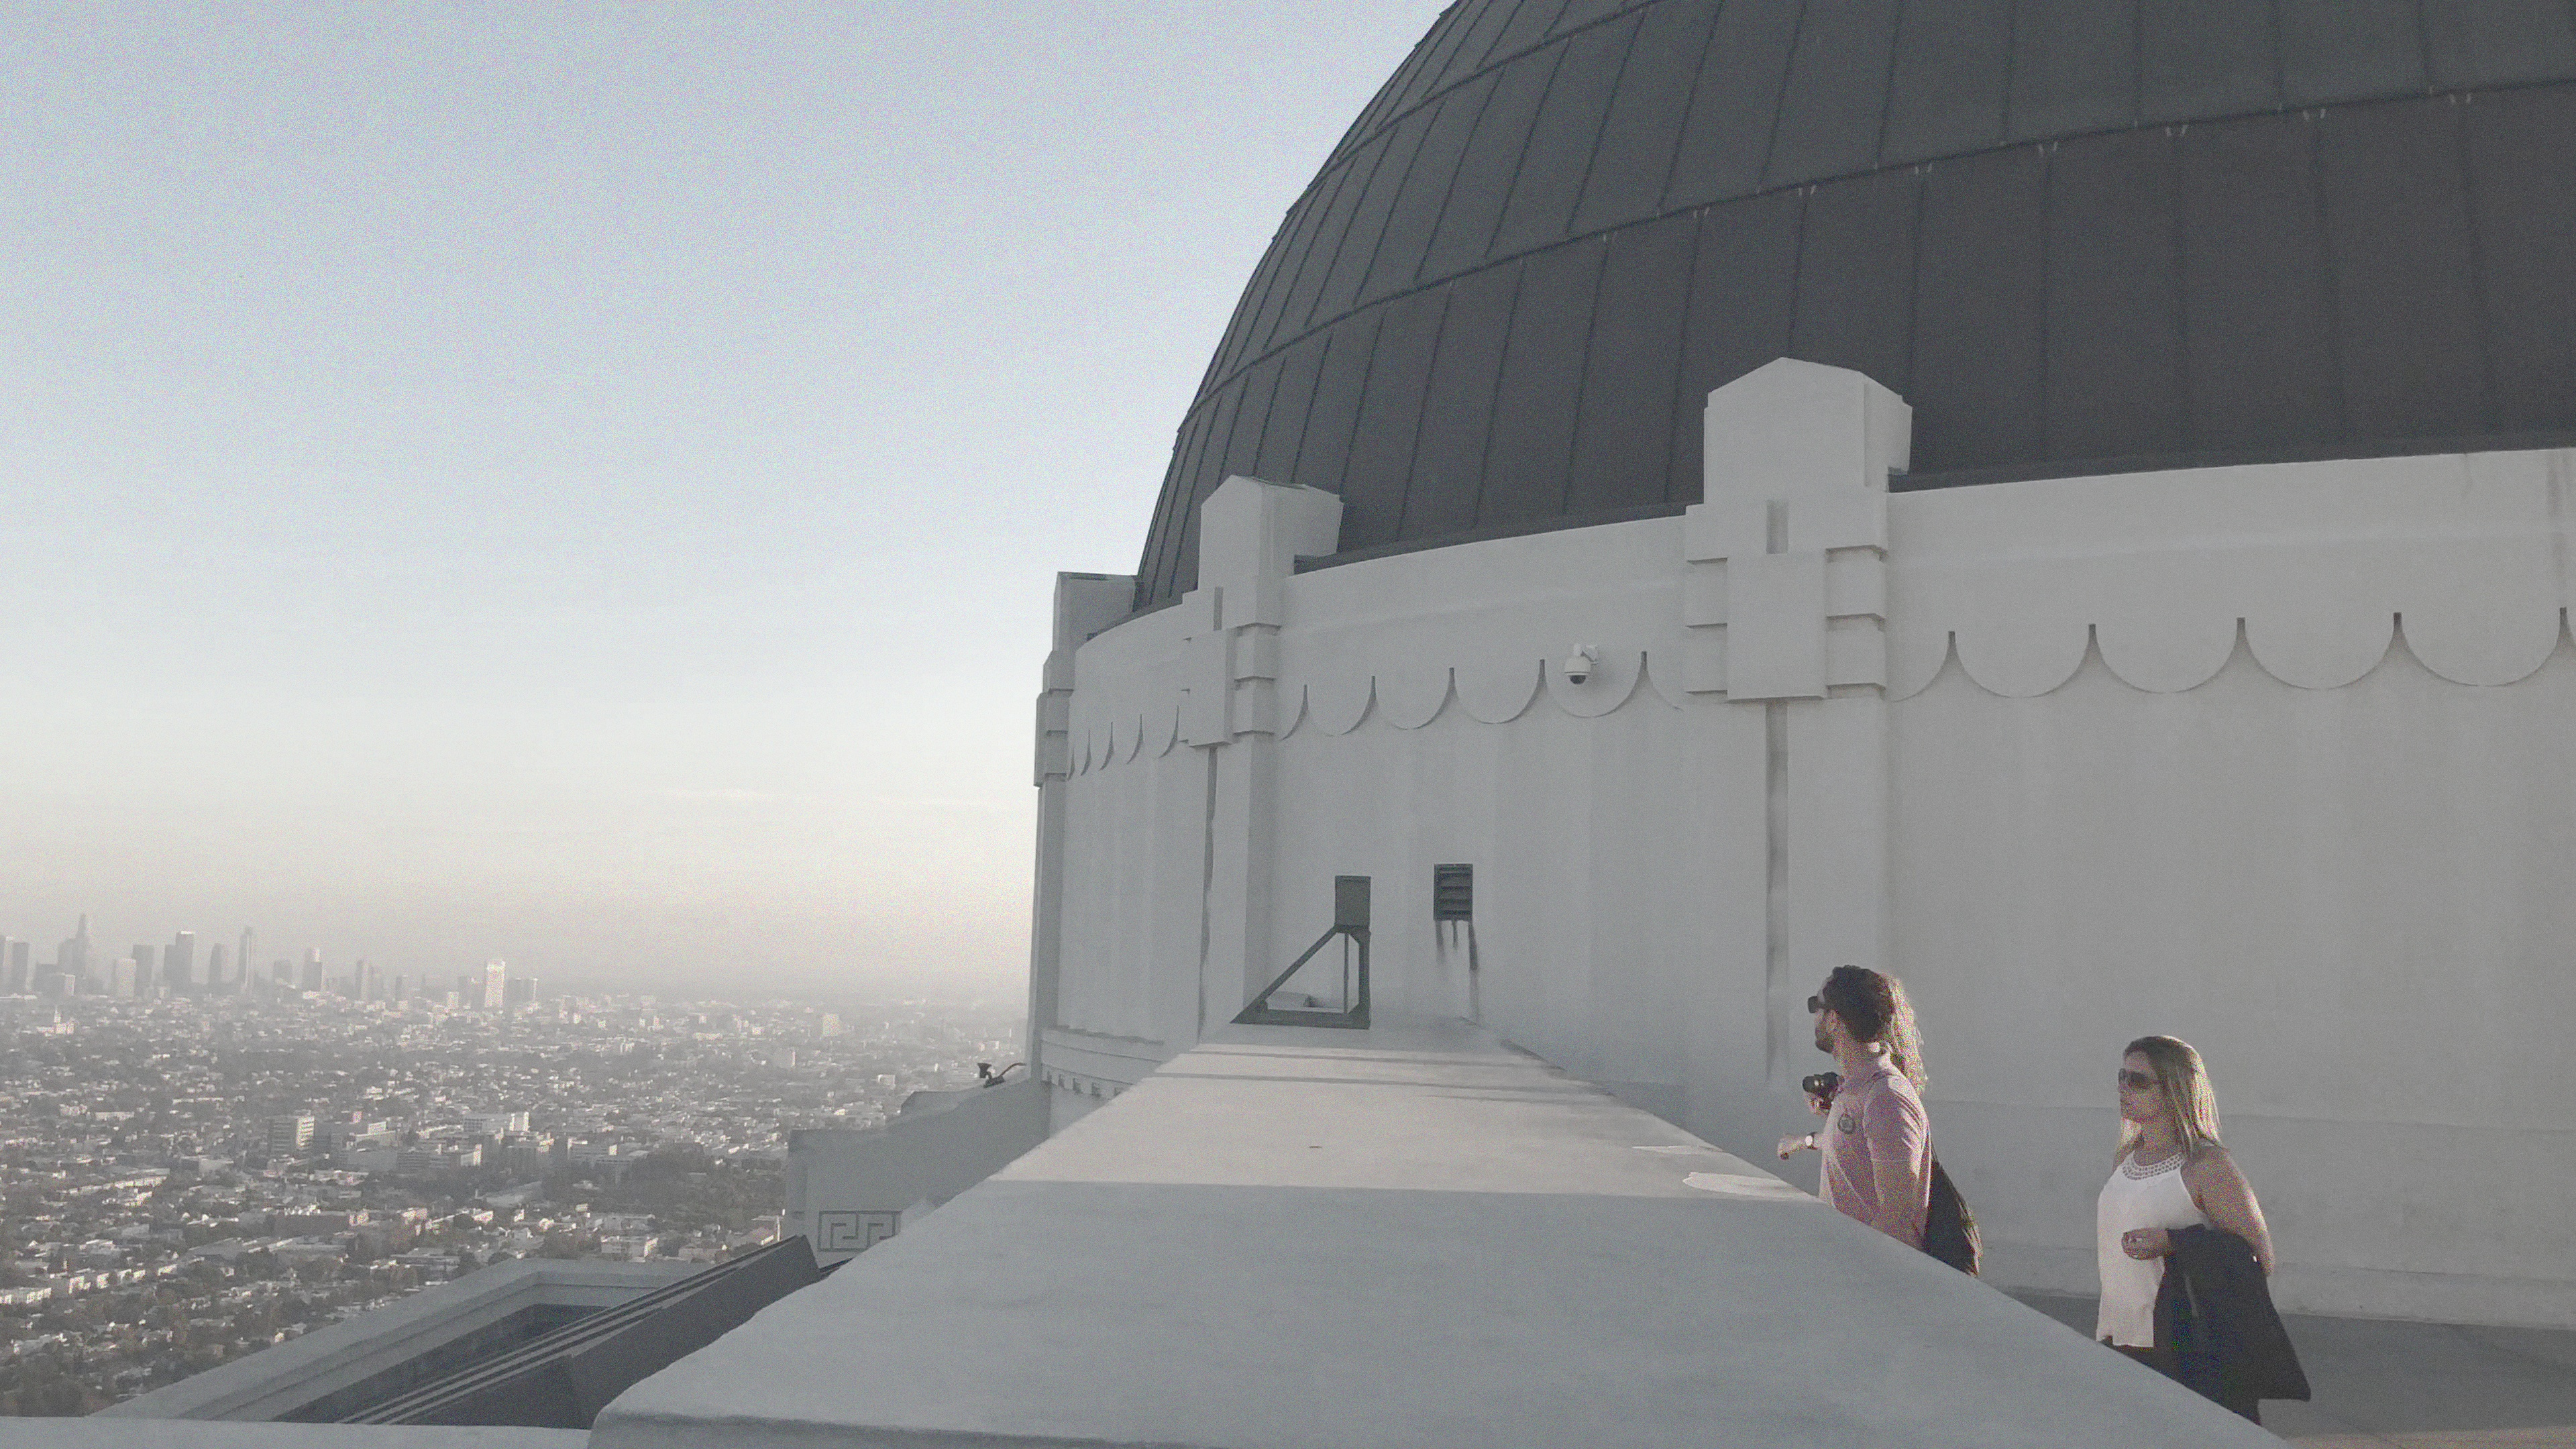}
        \caption{ISO Noise}
    \end{subfigure}
    \\    
    % Motion Blur
    \begin{subfigure}[b]{0.3\textwidth}
        \centering
        \includegraphics[width=\textwidth]{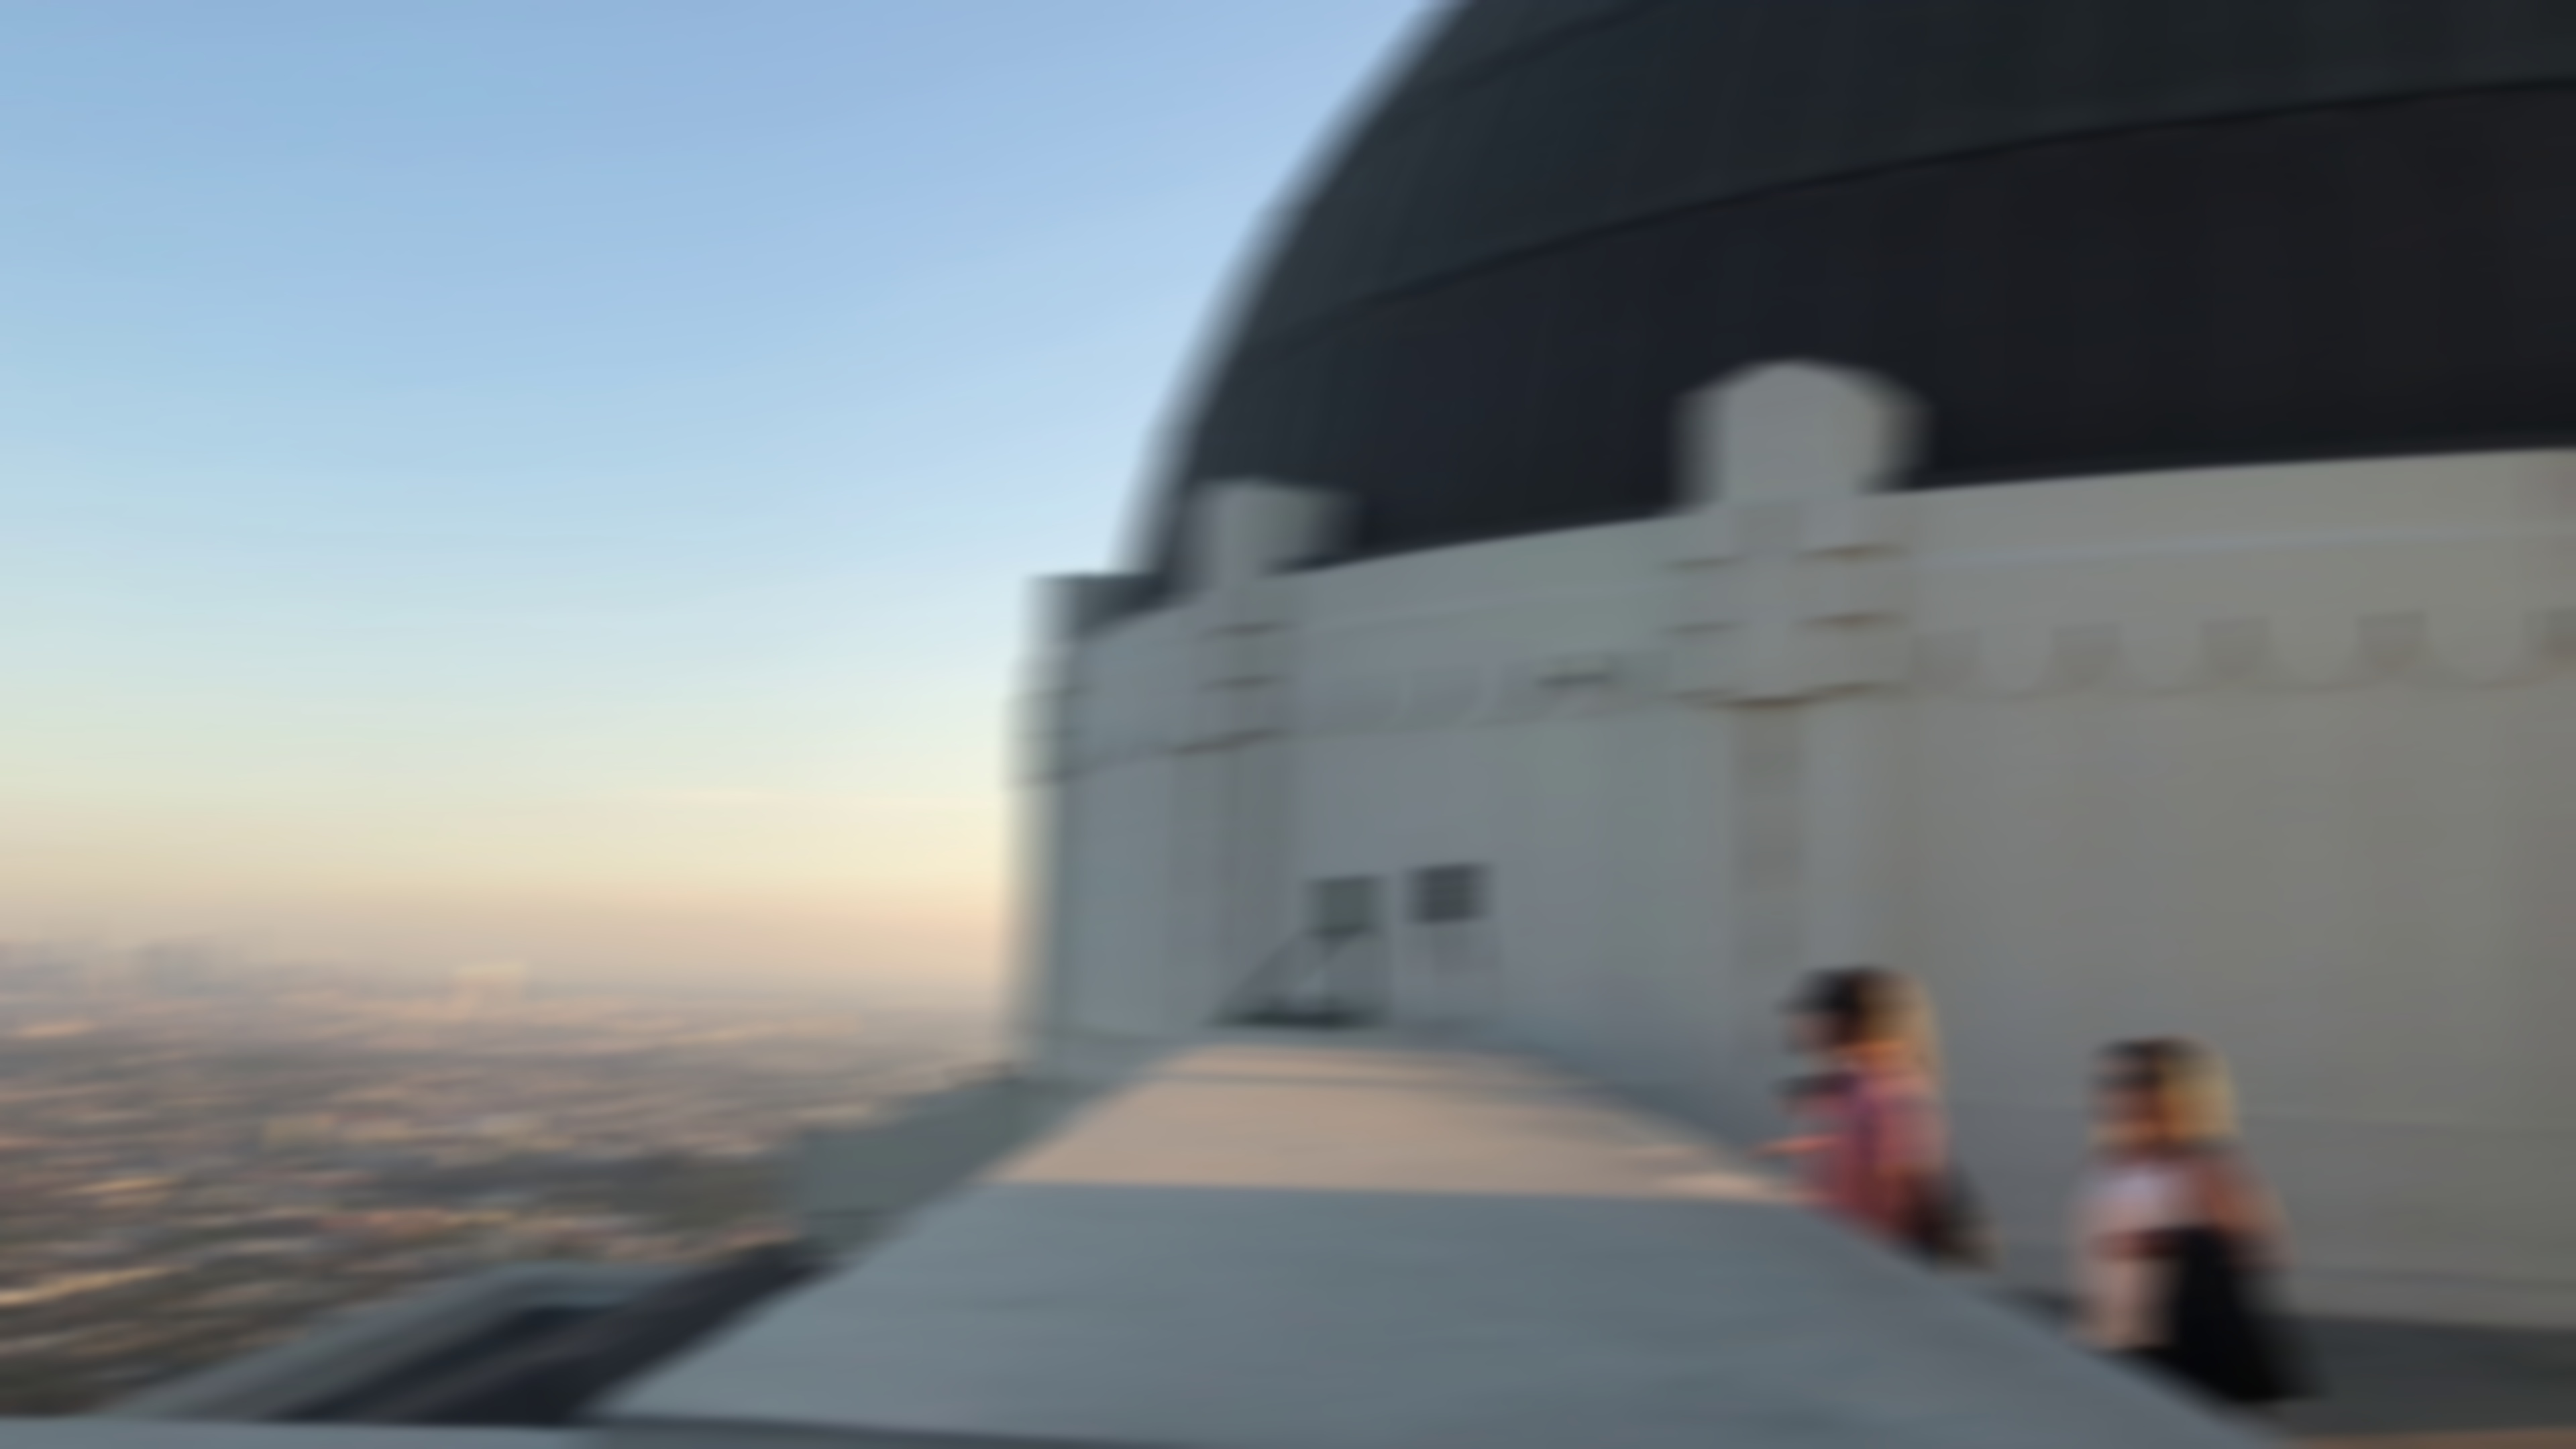}
        \caption{Motion Blur}
    \end{subfigure}
    % Compression
    \begin{subfigure}[b]{0.3\textwidth}
        \centering
        \includegraphics[width=\textwidth]{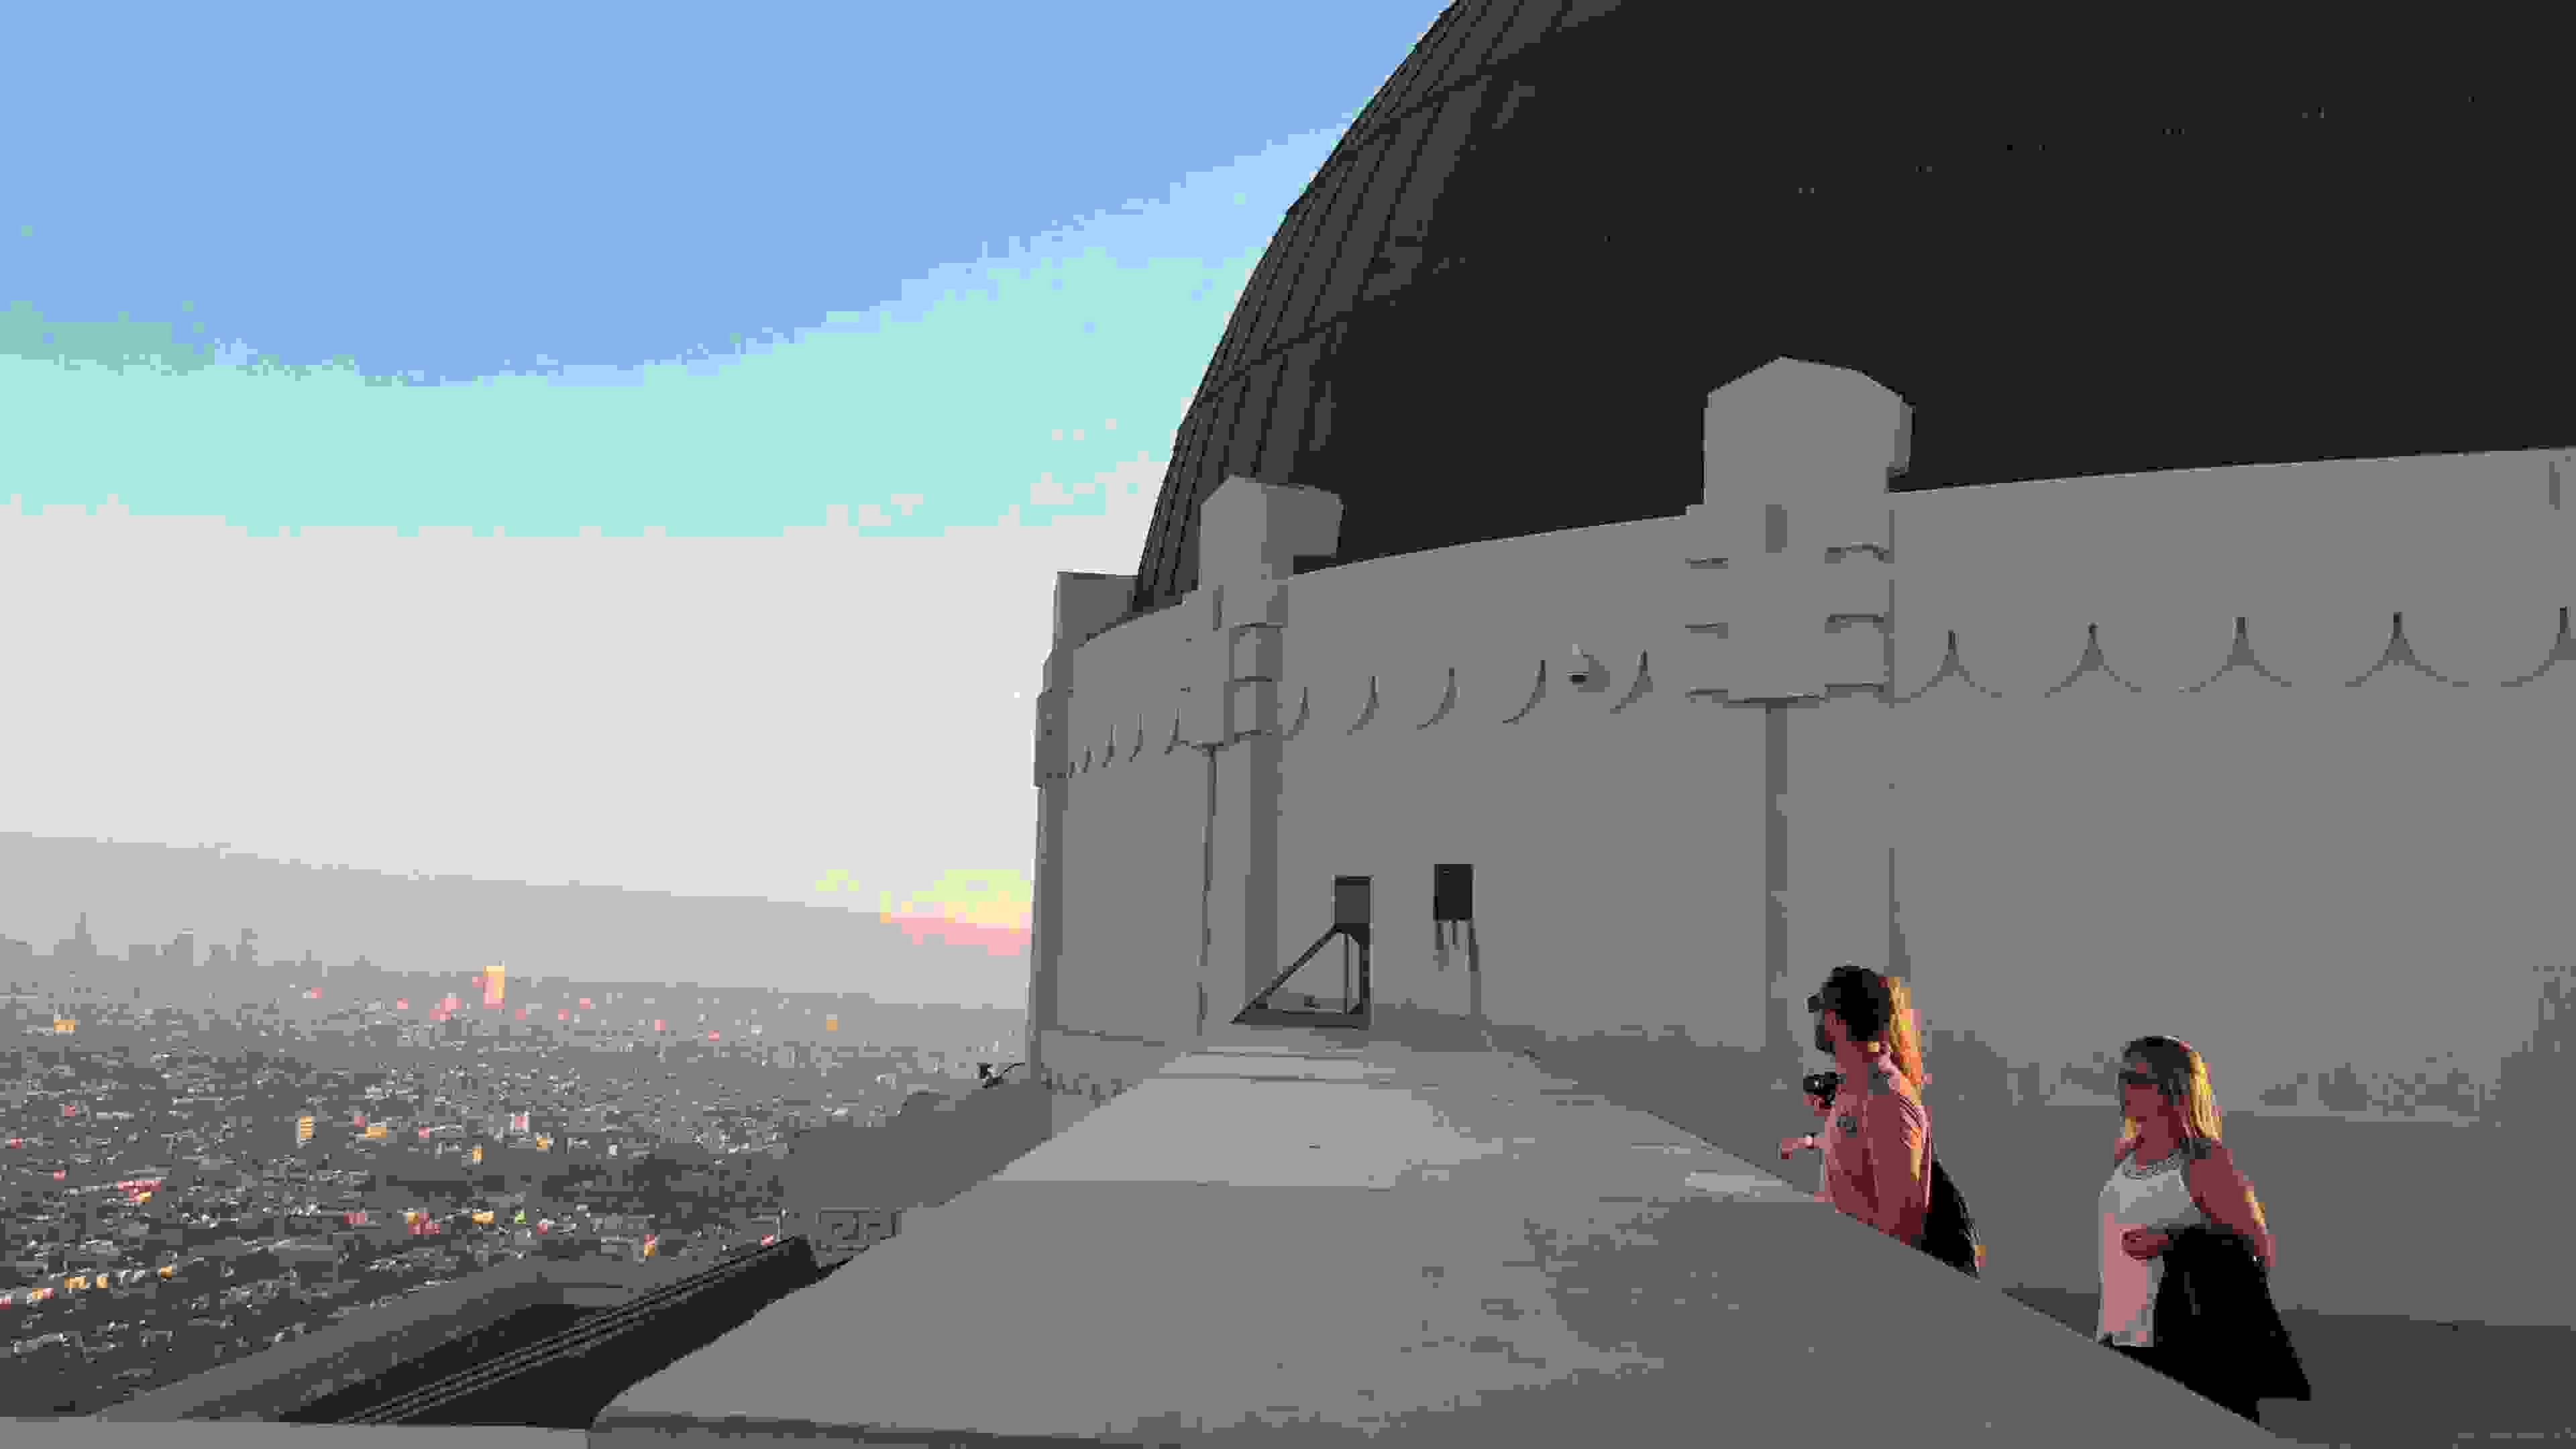}
        \caption{Compression}
    \end{subfigure}
    % Zoom Blur
    \begin{subfigure}[b]{0.3\textwidth}
        \centering
        \includegraphics[width=\textwidth]{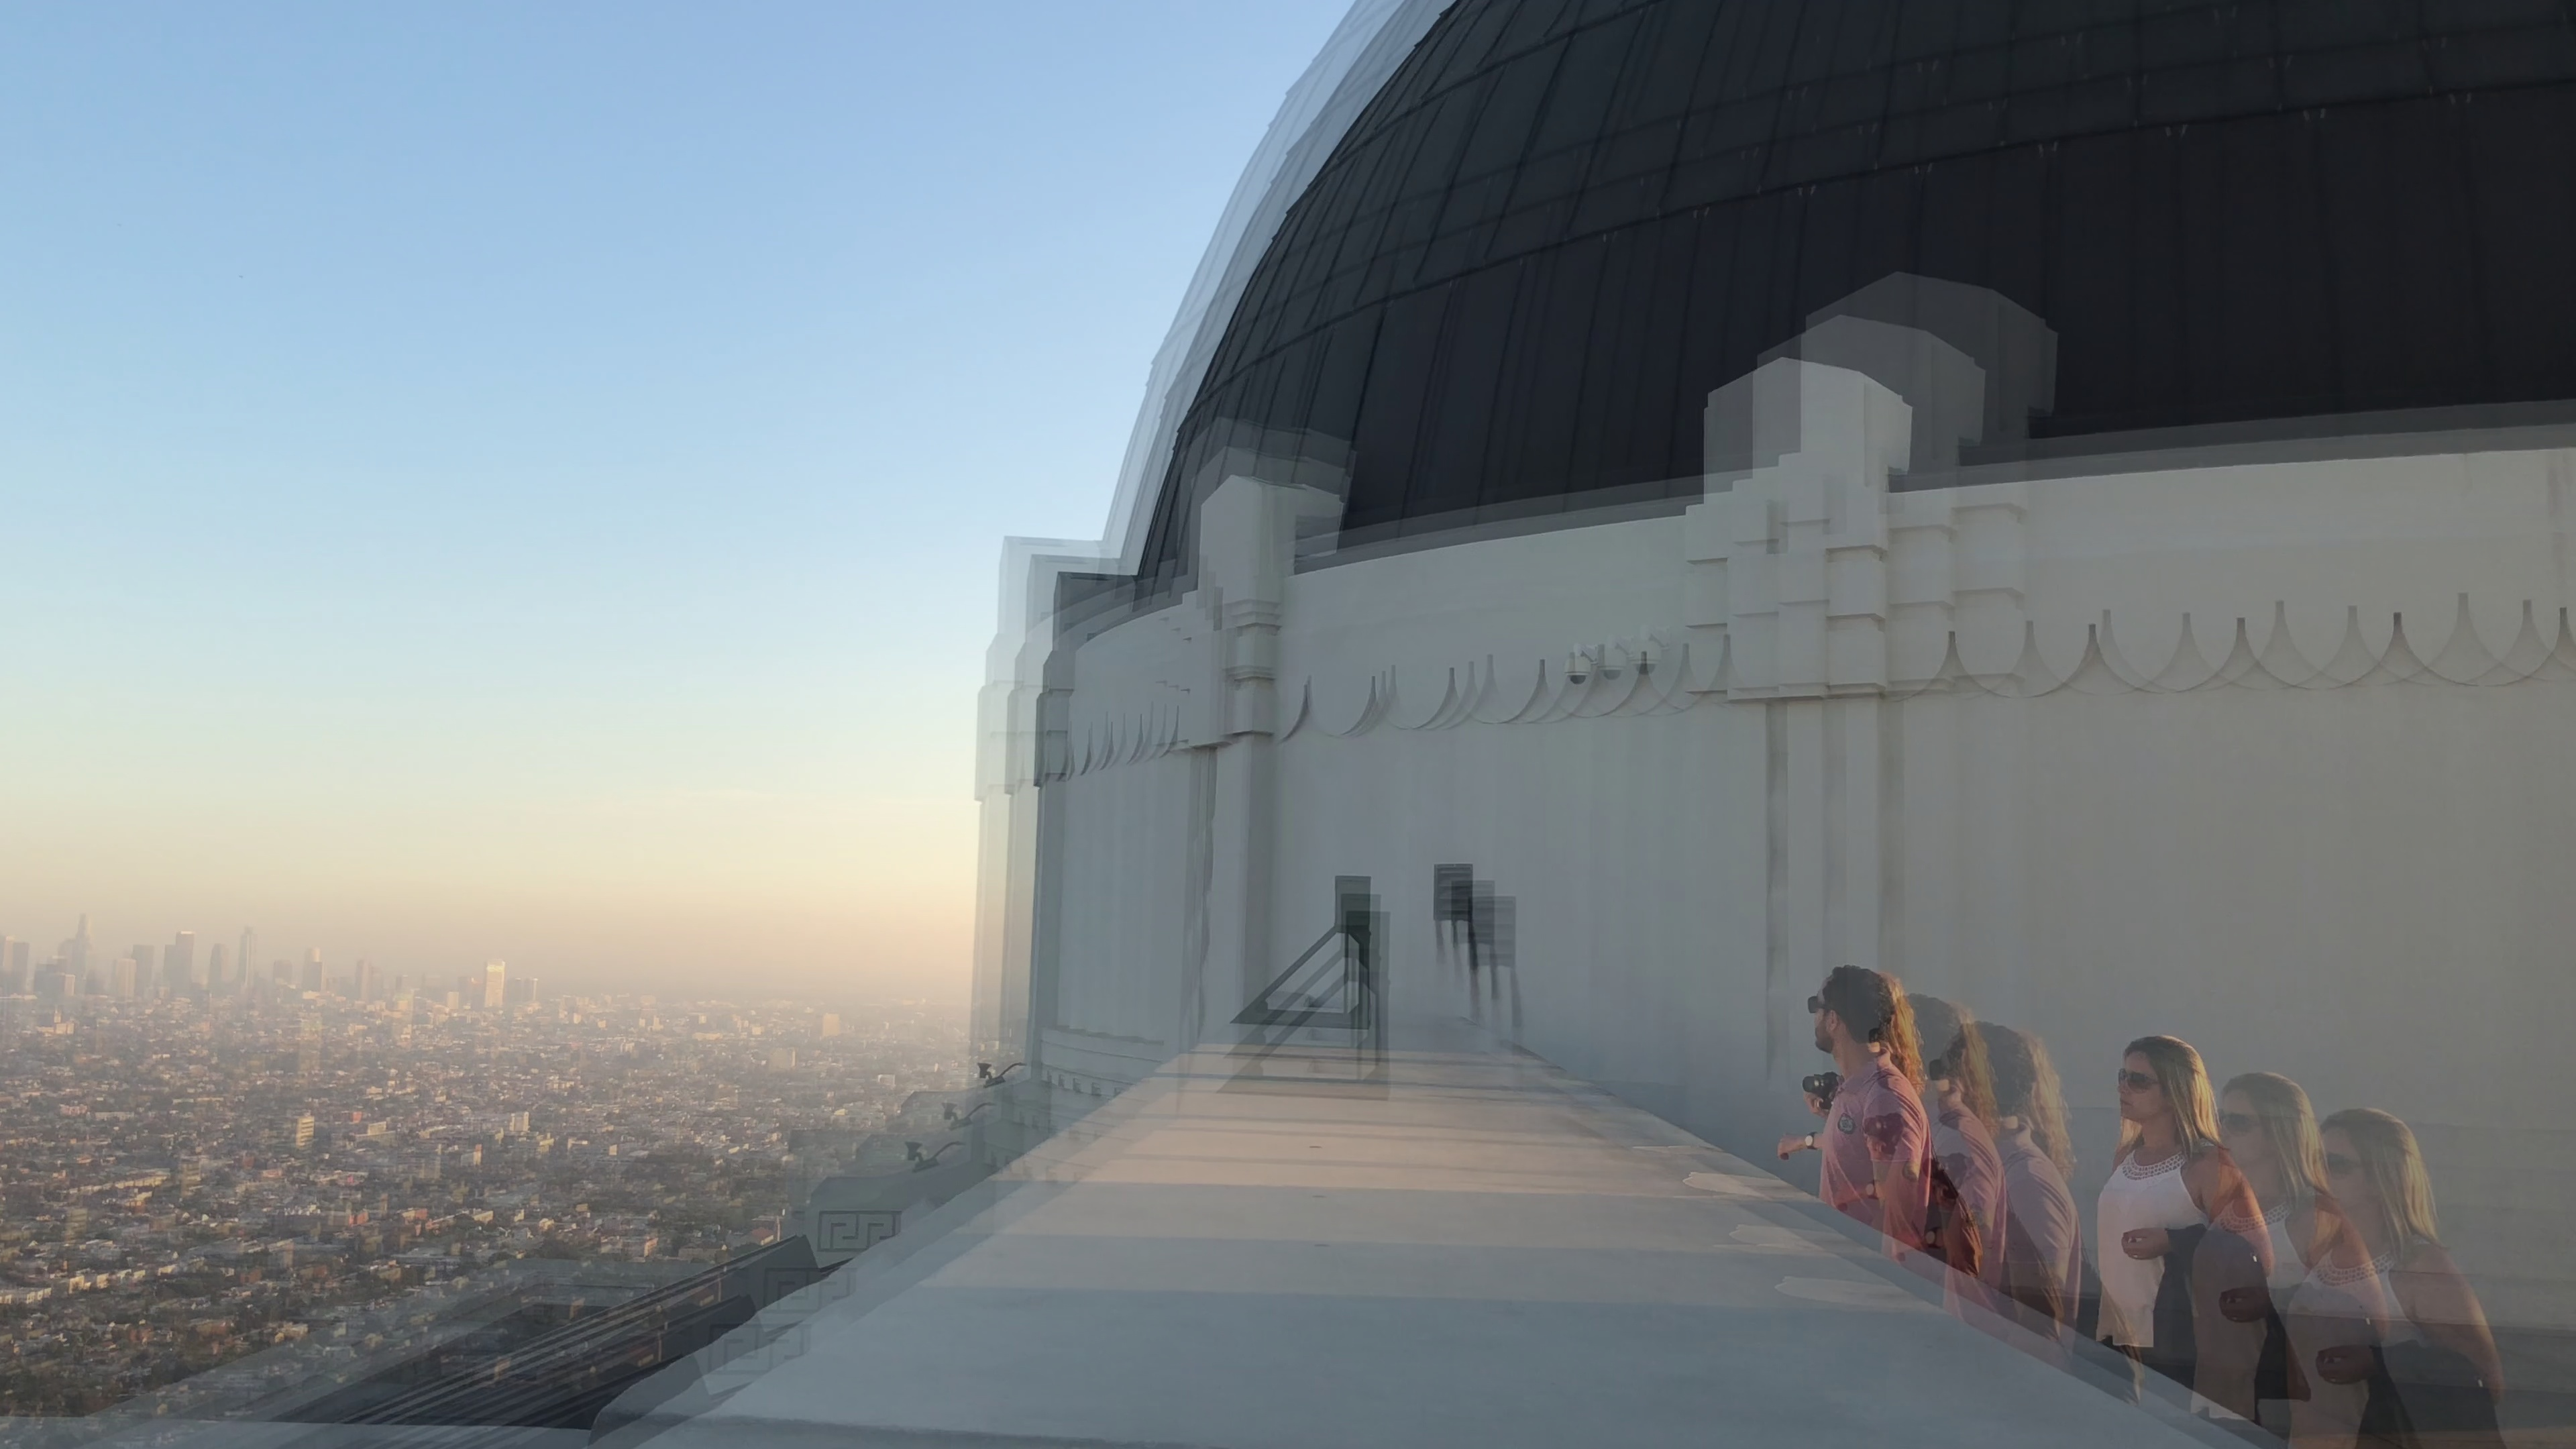}
        \caption{Zoom Blur}
    \end{subfigure}

    \caption{\textbf{Examples of video frames with different distortion types.}}
    \label{fig:distortion_examples}
\end{figure*}

\begin{figure*}[t]
    \centering
    % Video 1
    \begin{subfigure}[b]{0.3\textwidth}
        \centering
        \includegraphics[width=\textwidth]{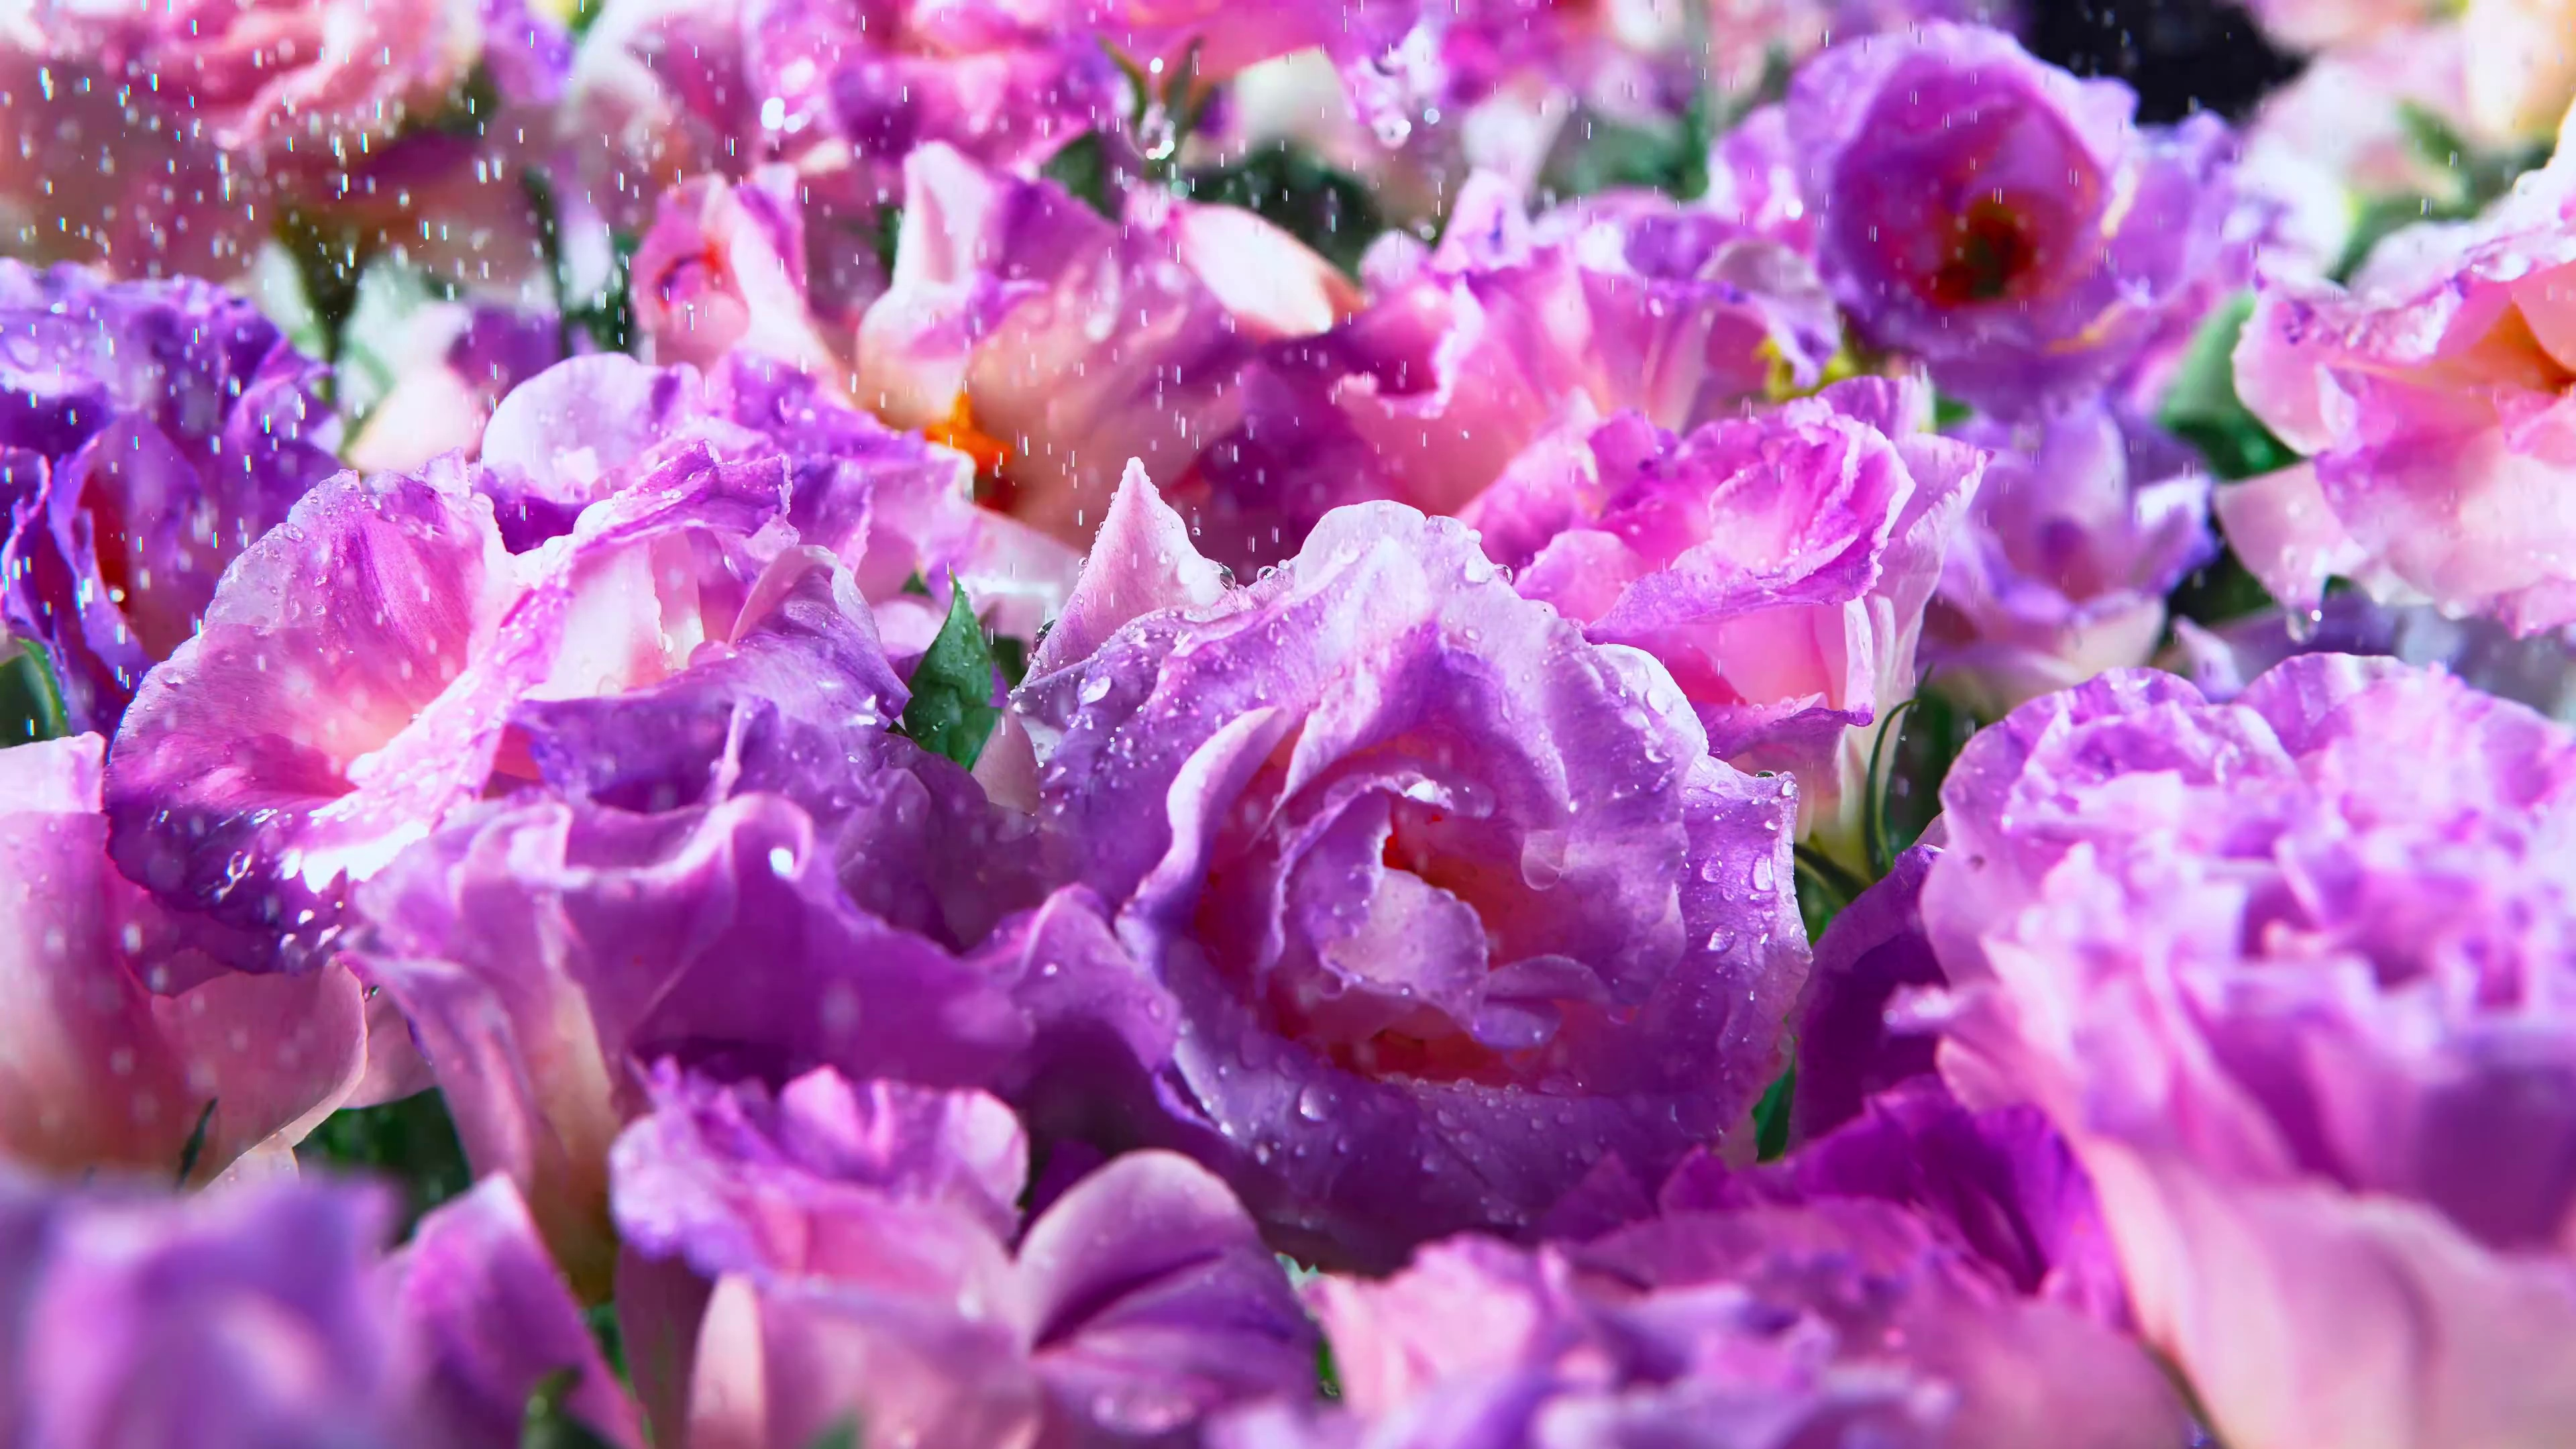}
        \caption{Video 1}
    \end{subfigure}
    % Video 2
    \begin{subfigure}[b]{0.3\textwidth}
        \centering
        \includegraphics[width=\textwidth]{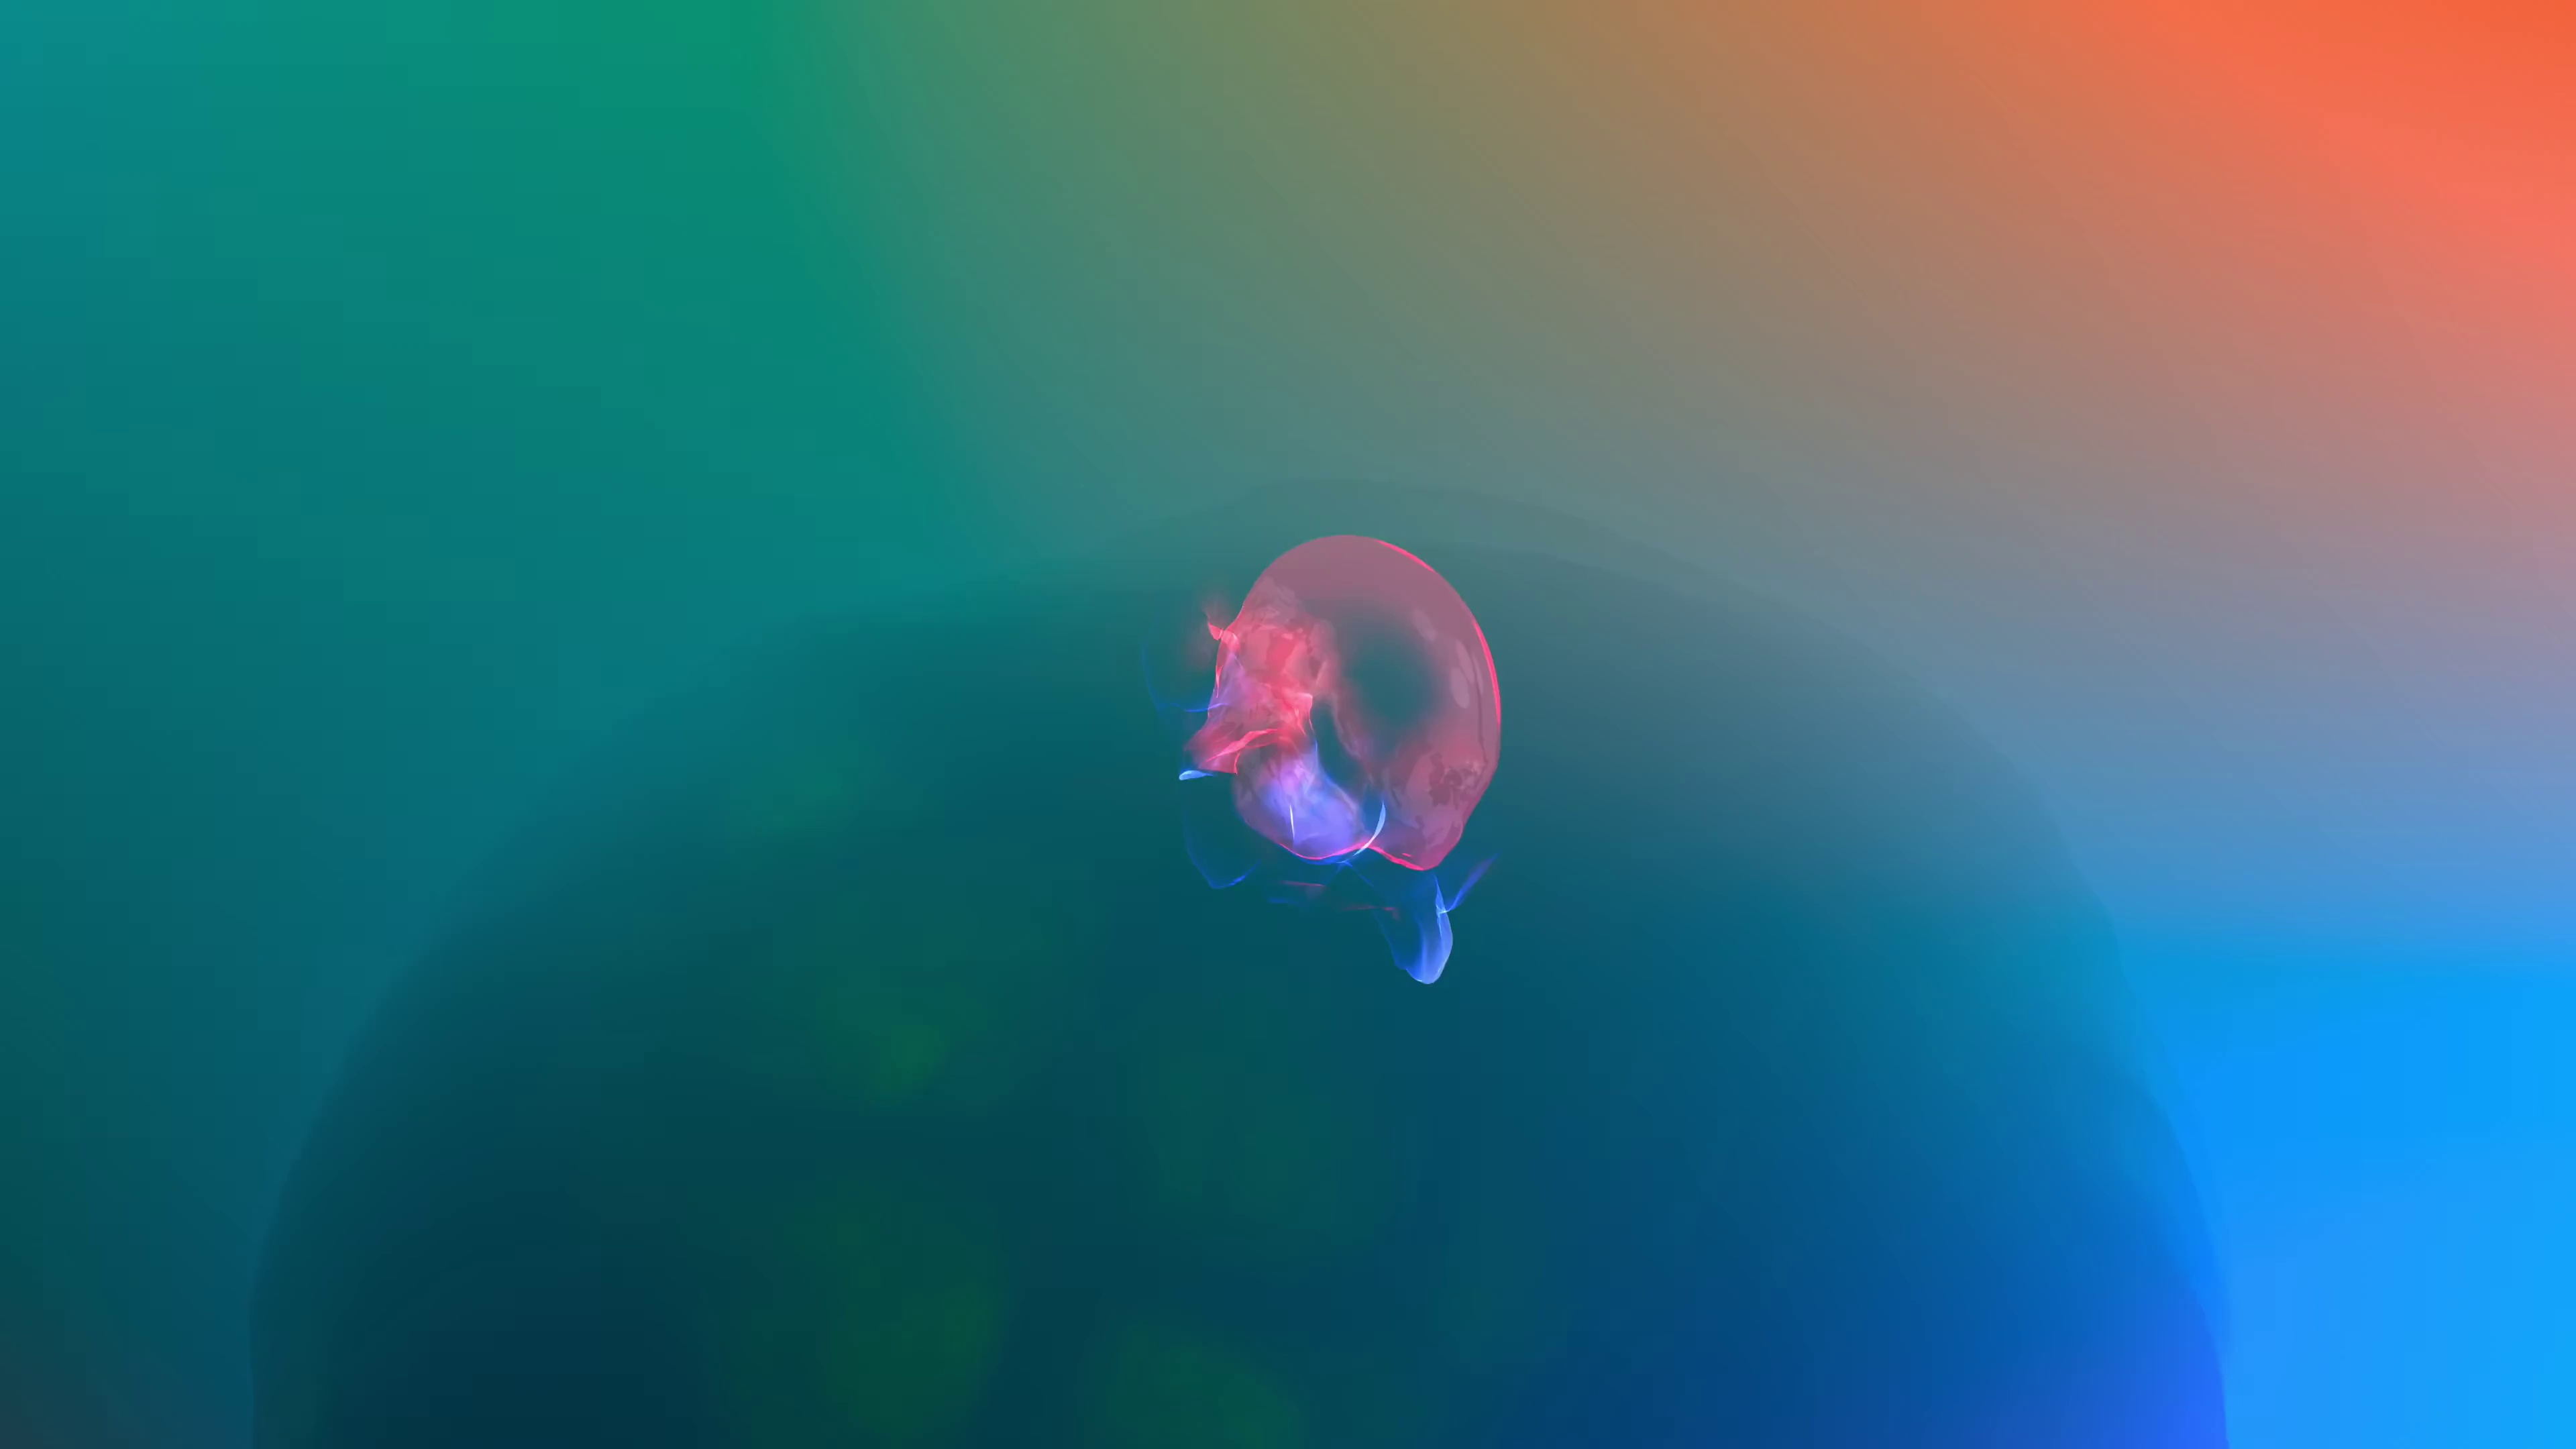}
        \caption{Video 2}
    \end{subfigure}
    % Video 3
    \begin{subfigure}[b]{0.3\textwidth}
        \centering
        \includegraphics[width=\textwidth]{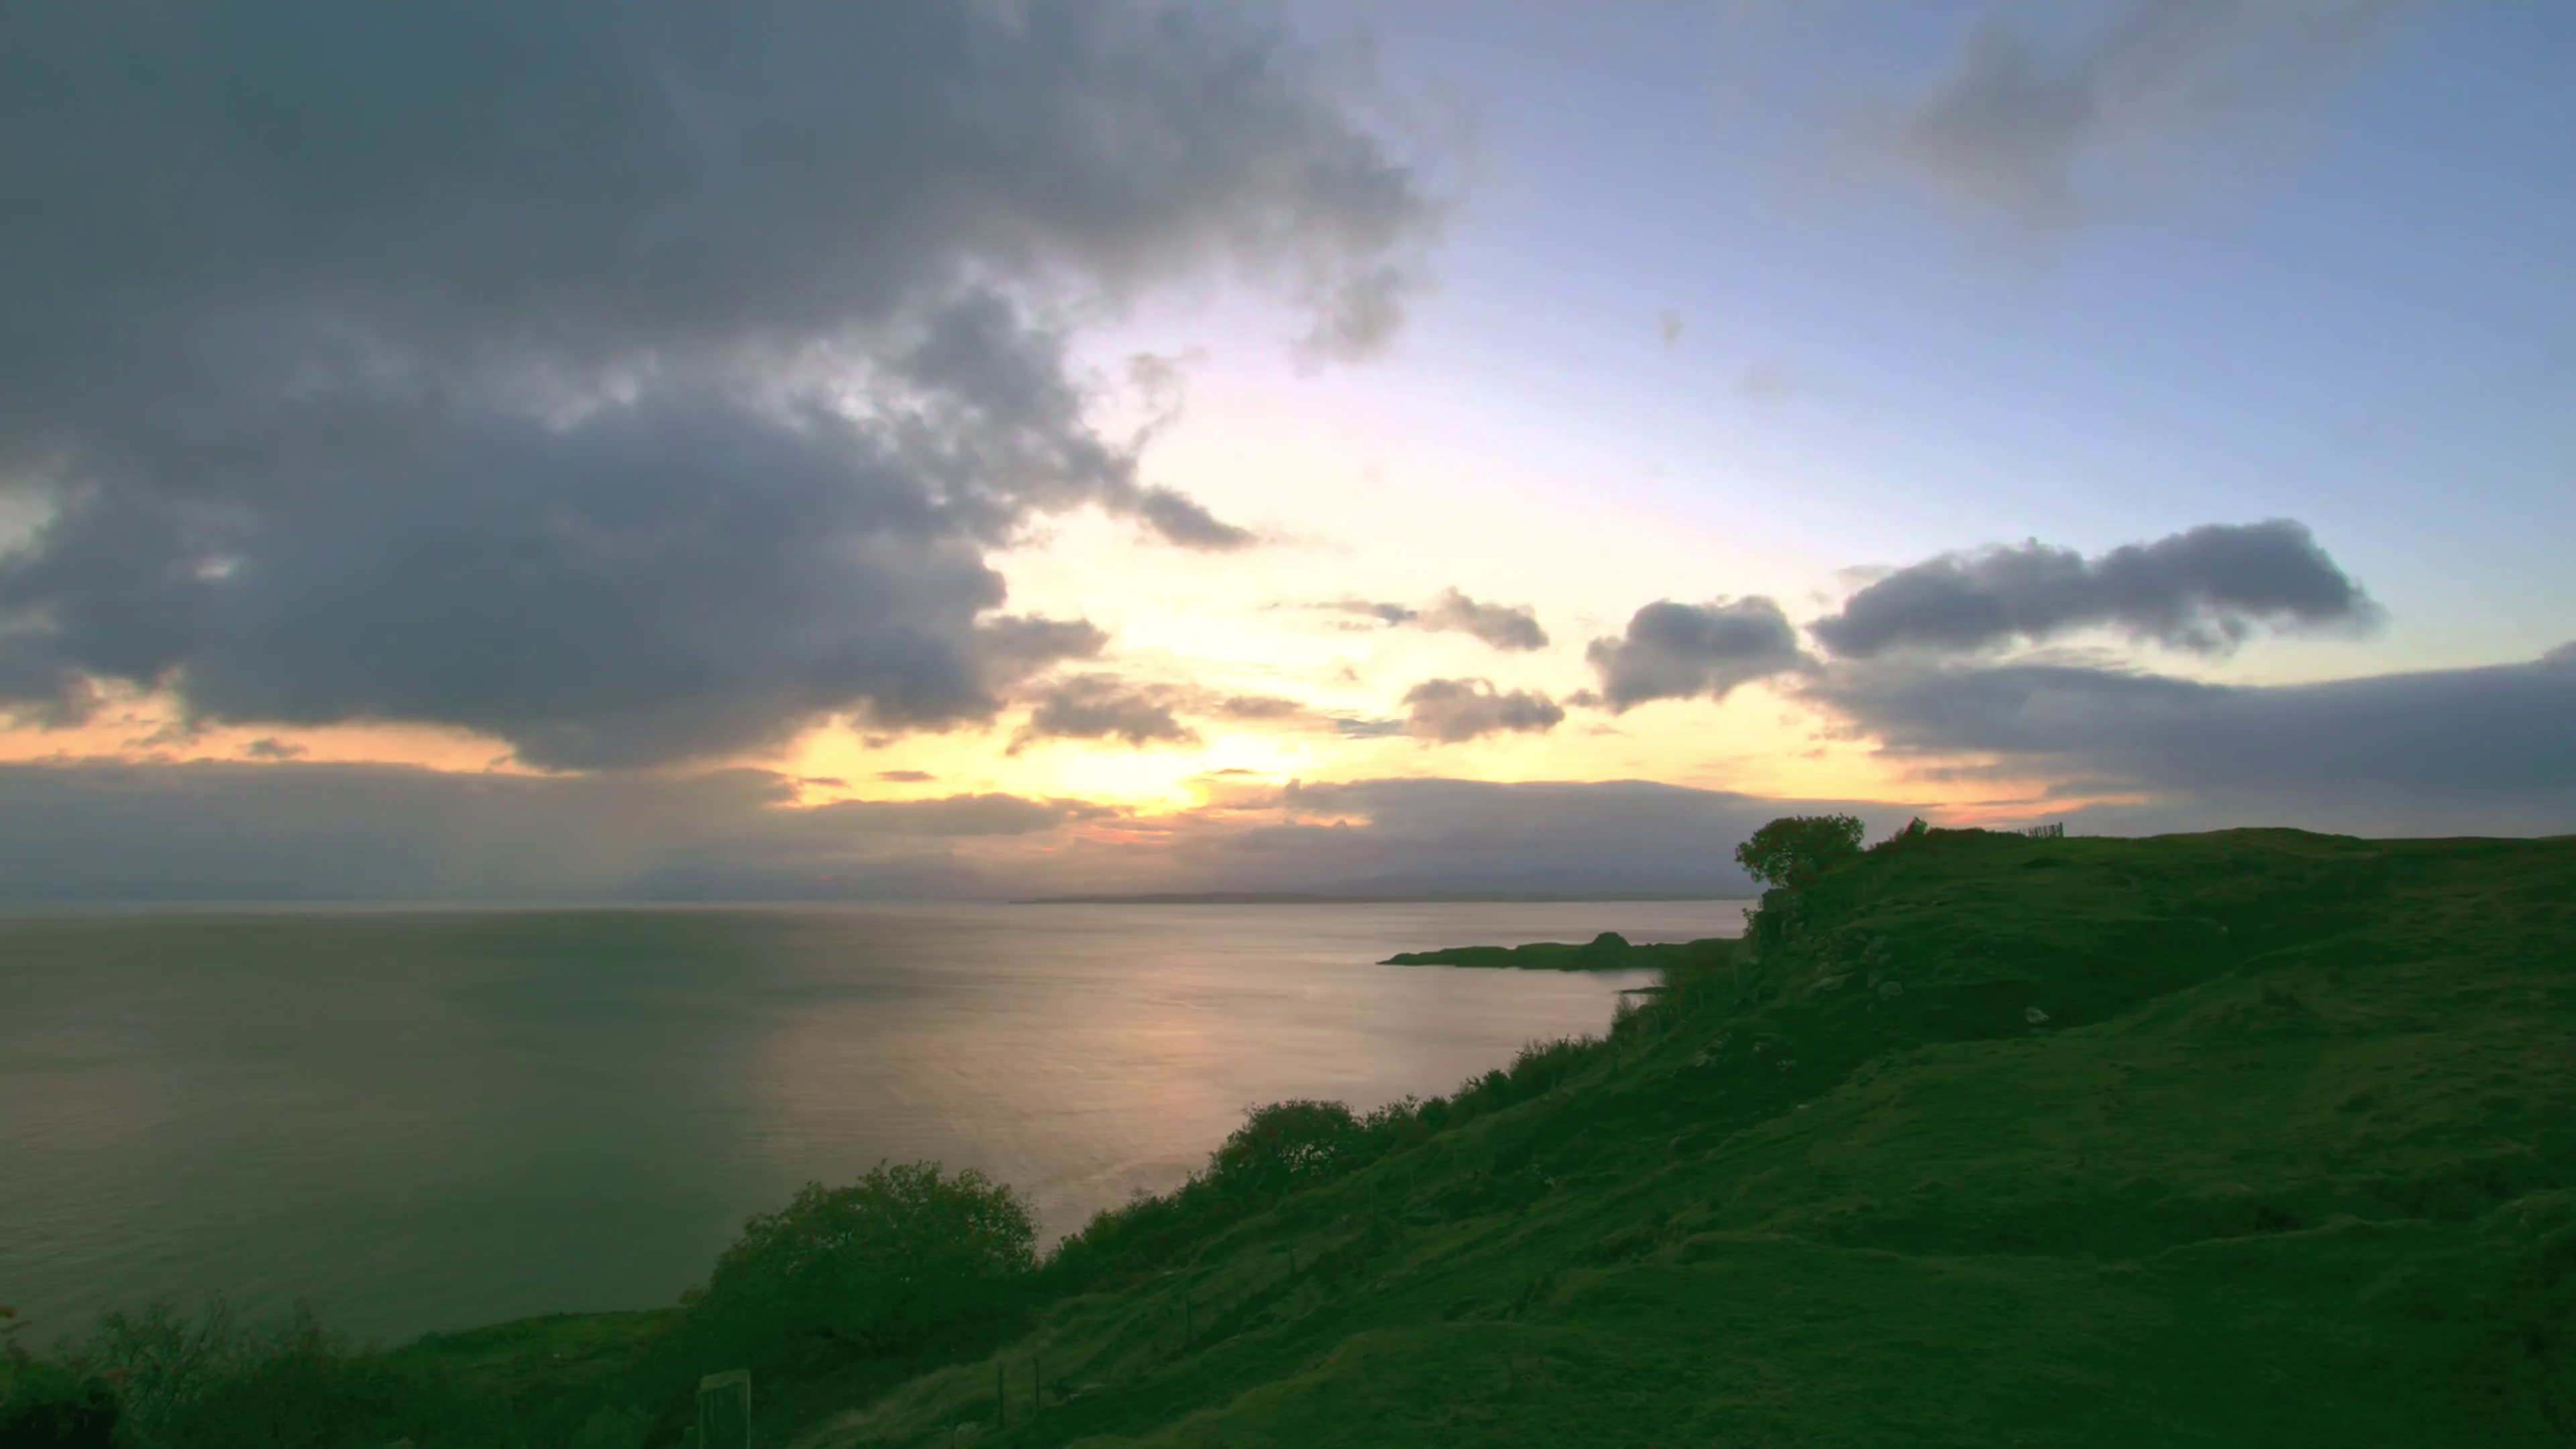}
        \caption{Video 3}
    \end{subfigure}
    
    \vspace{0.5cm}
    
    % Video 4
    \begin{subfigure}[b]{0.3\textwidth}
        \centering
        \includegraphics[width=\textwidth]{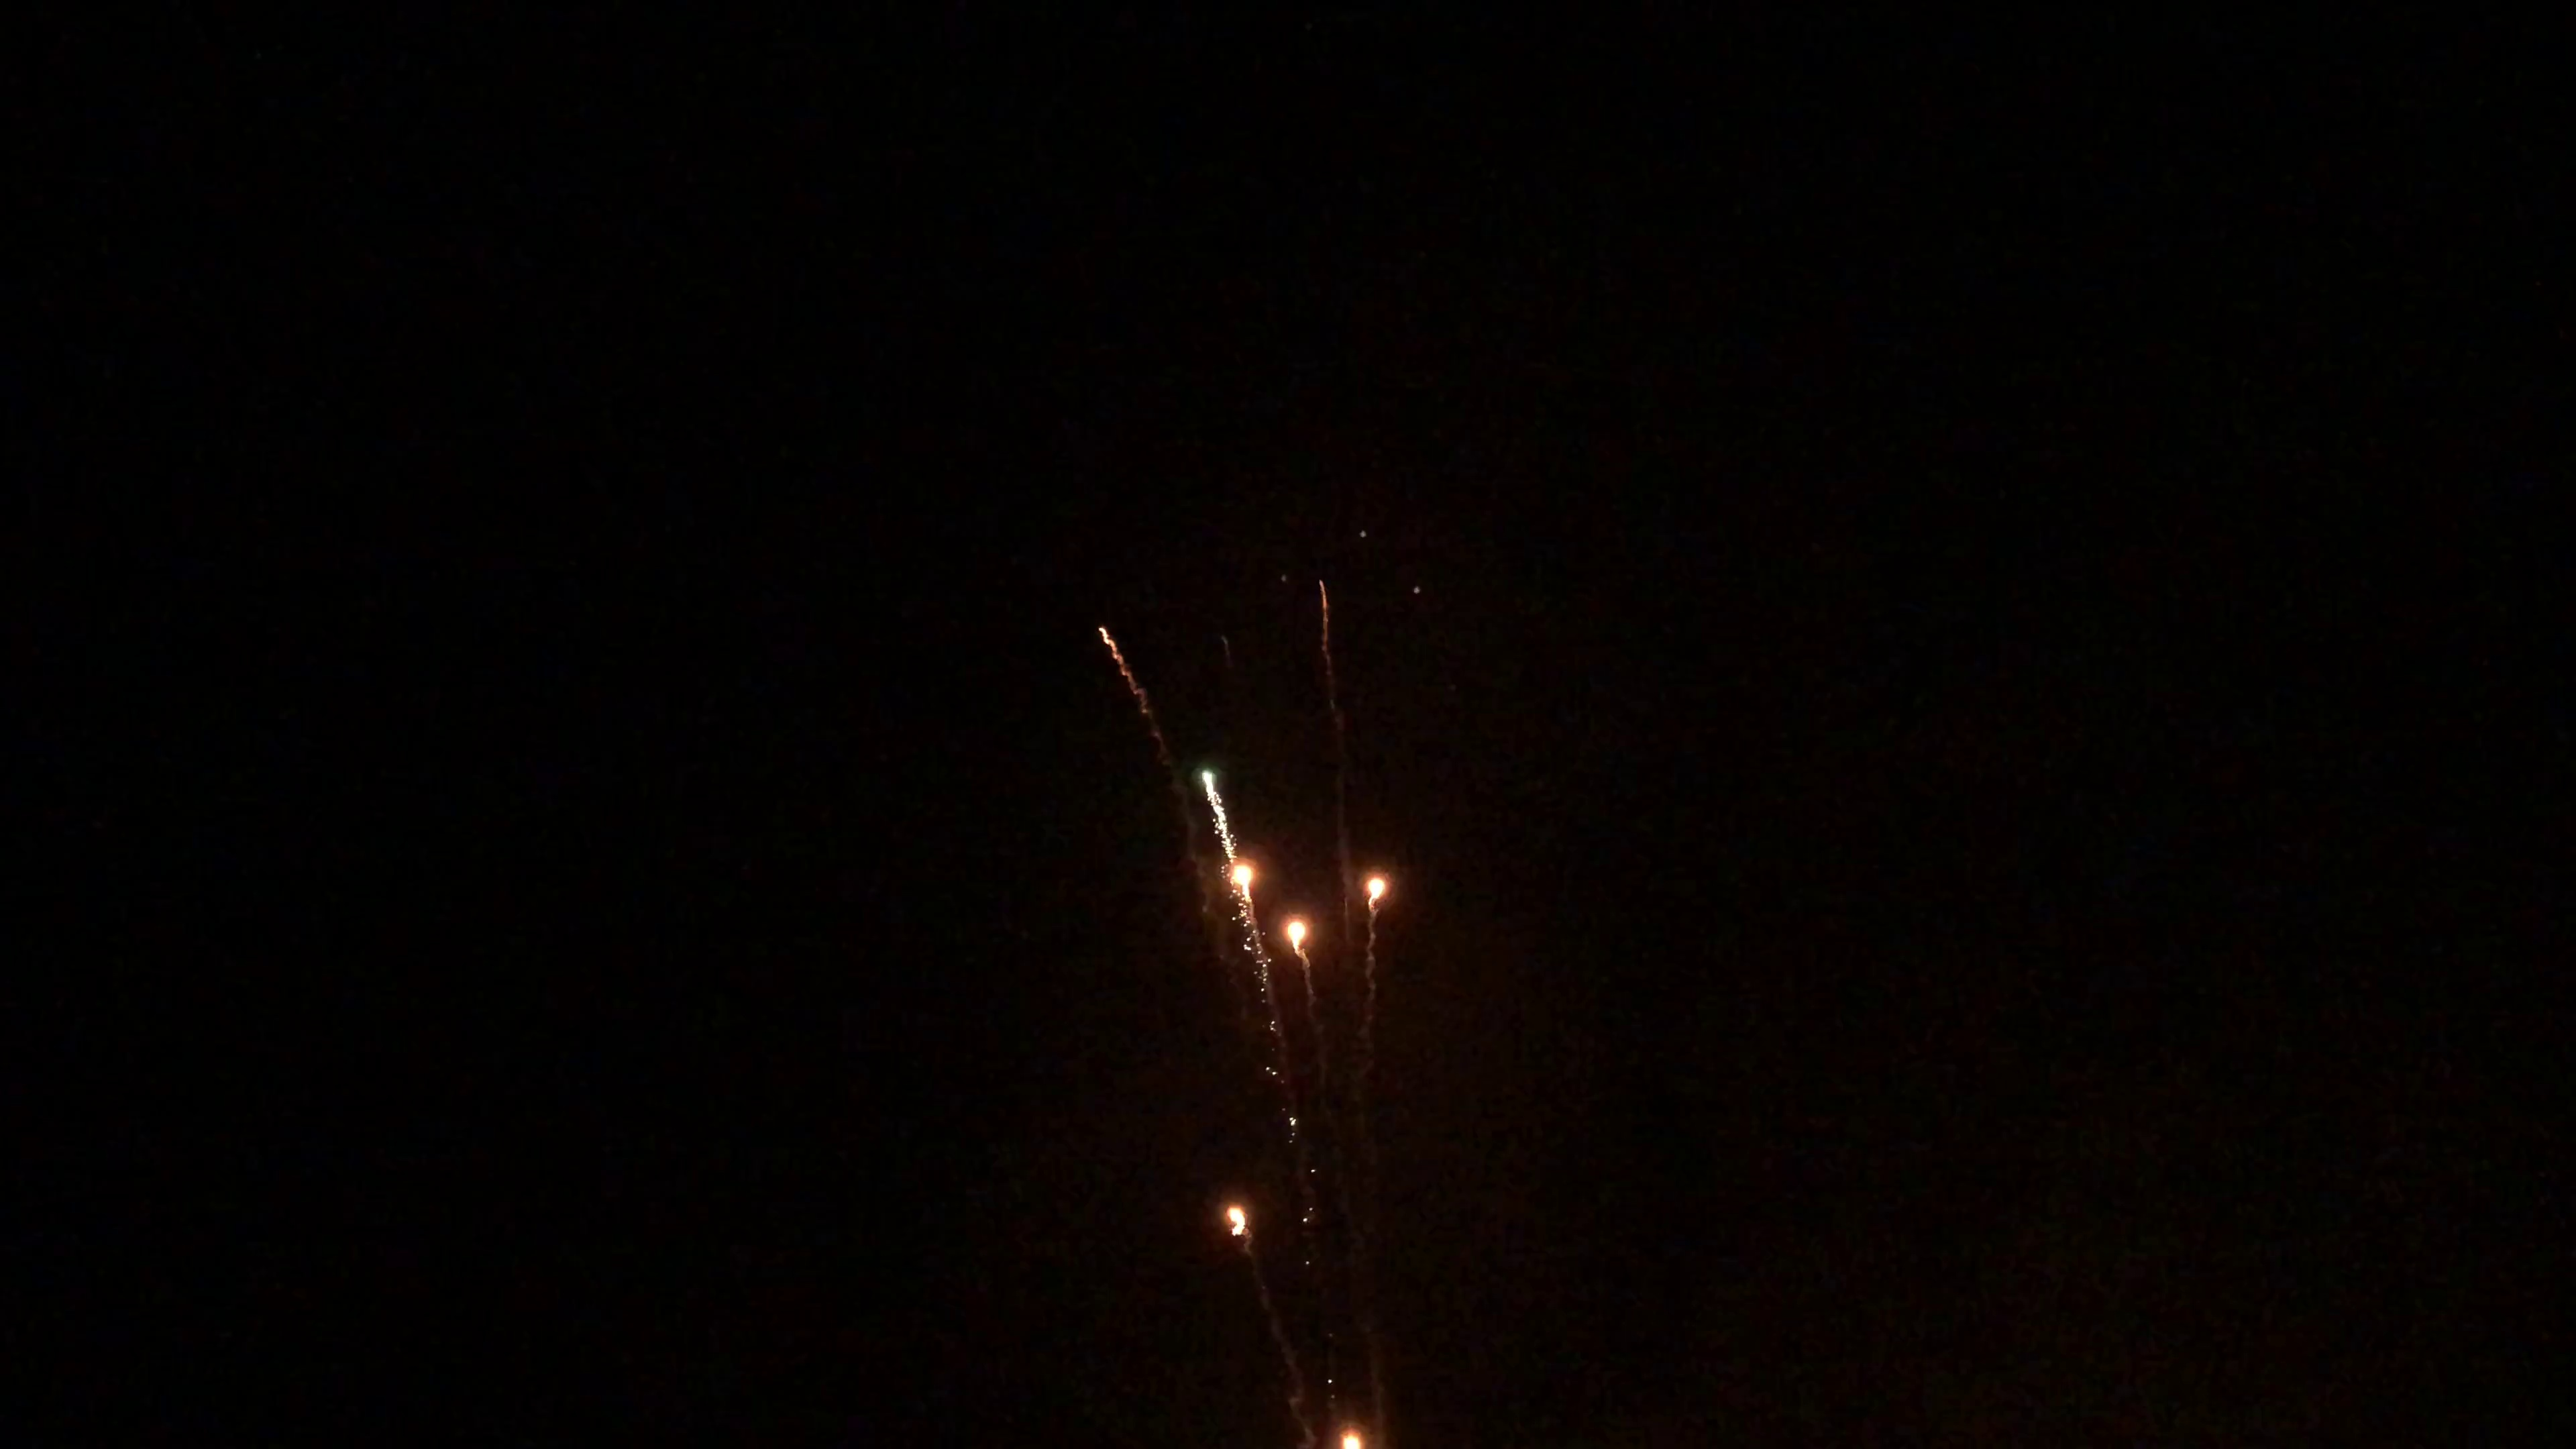}
        \caption{Video 4}
    \end{subfigure}
    % Video 5
    \begin{subfigure}[b]{0.3\textwidth}
        \centering
        \includegraphics[width=\textwidth]{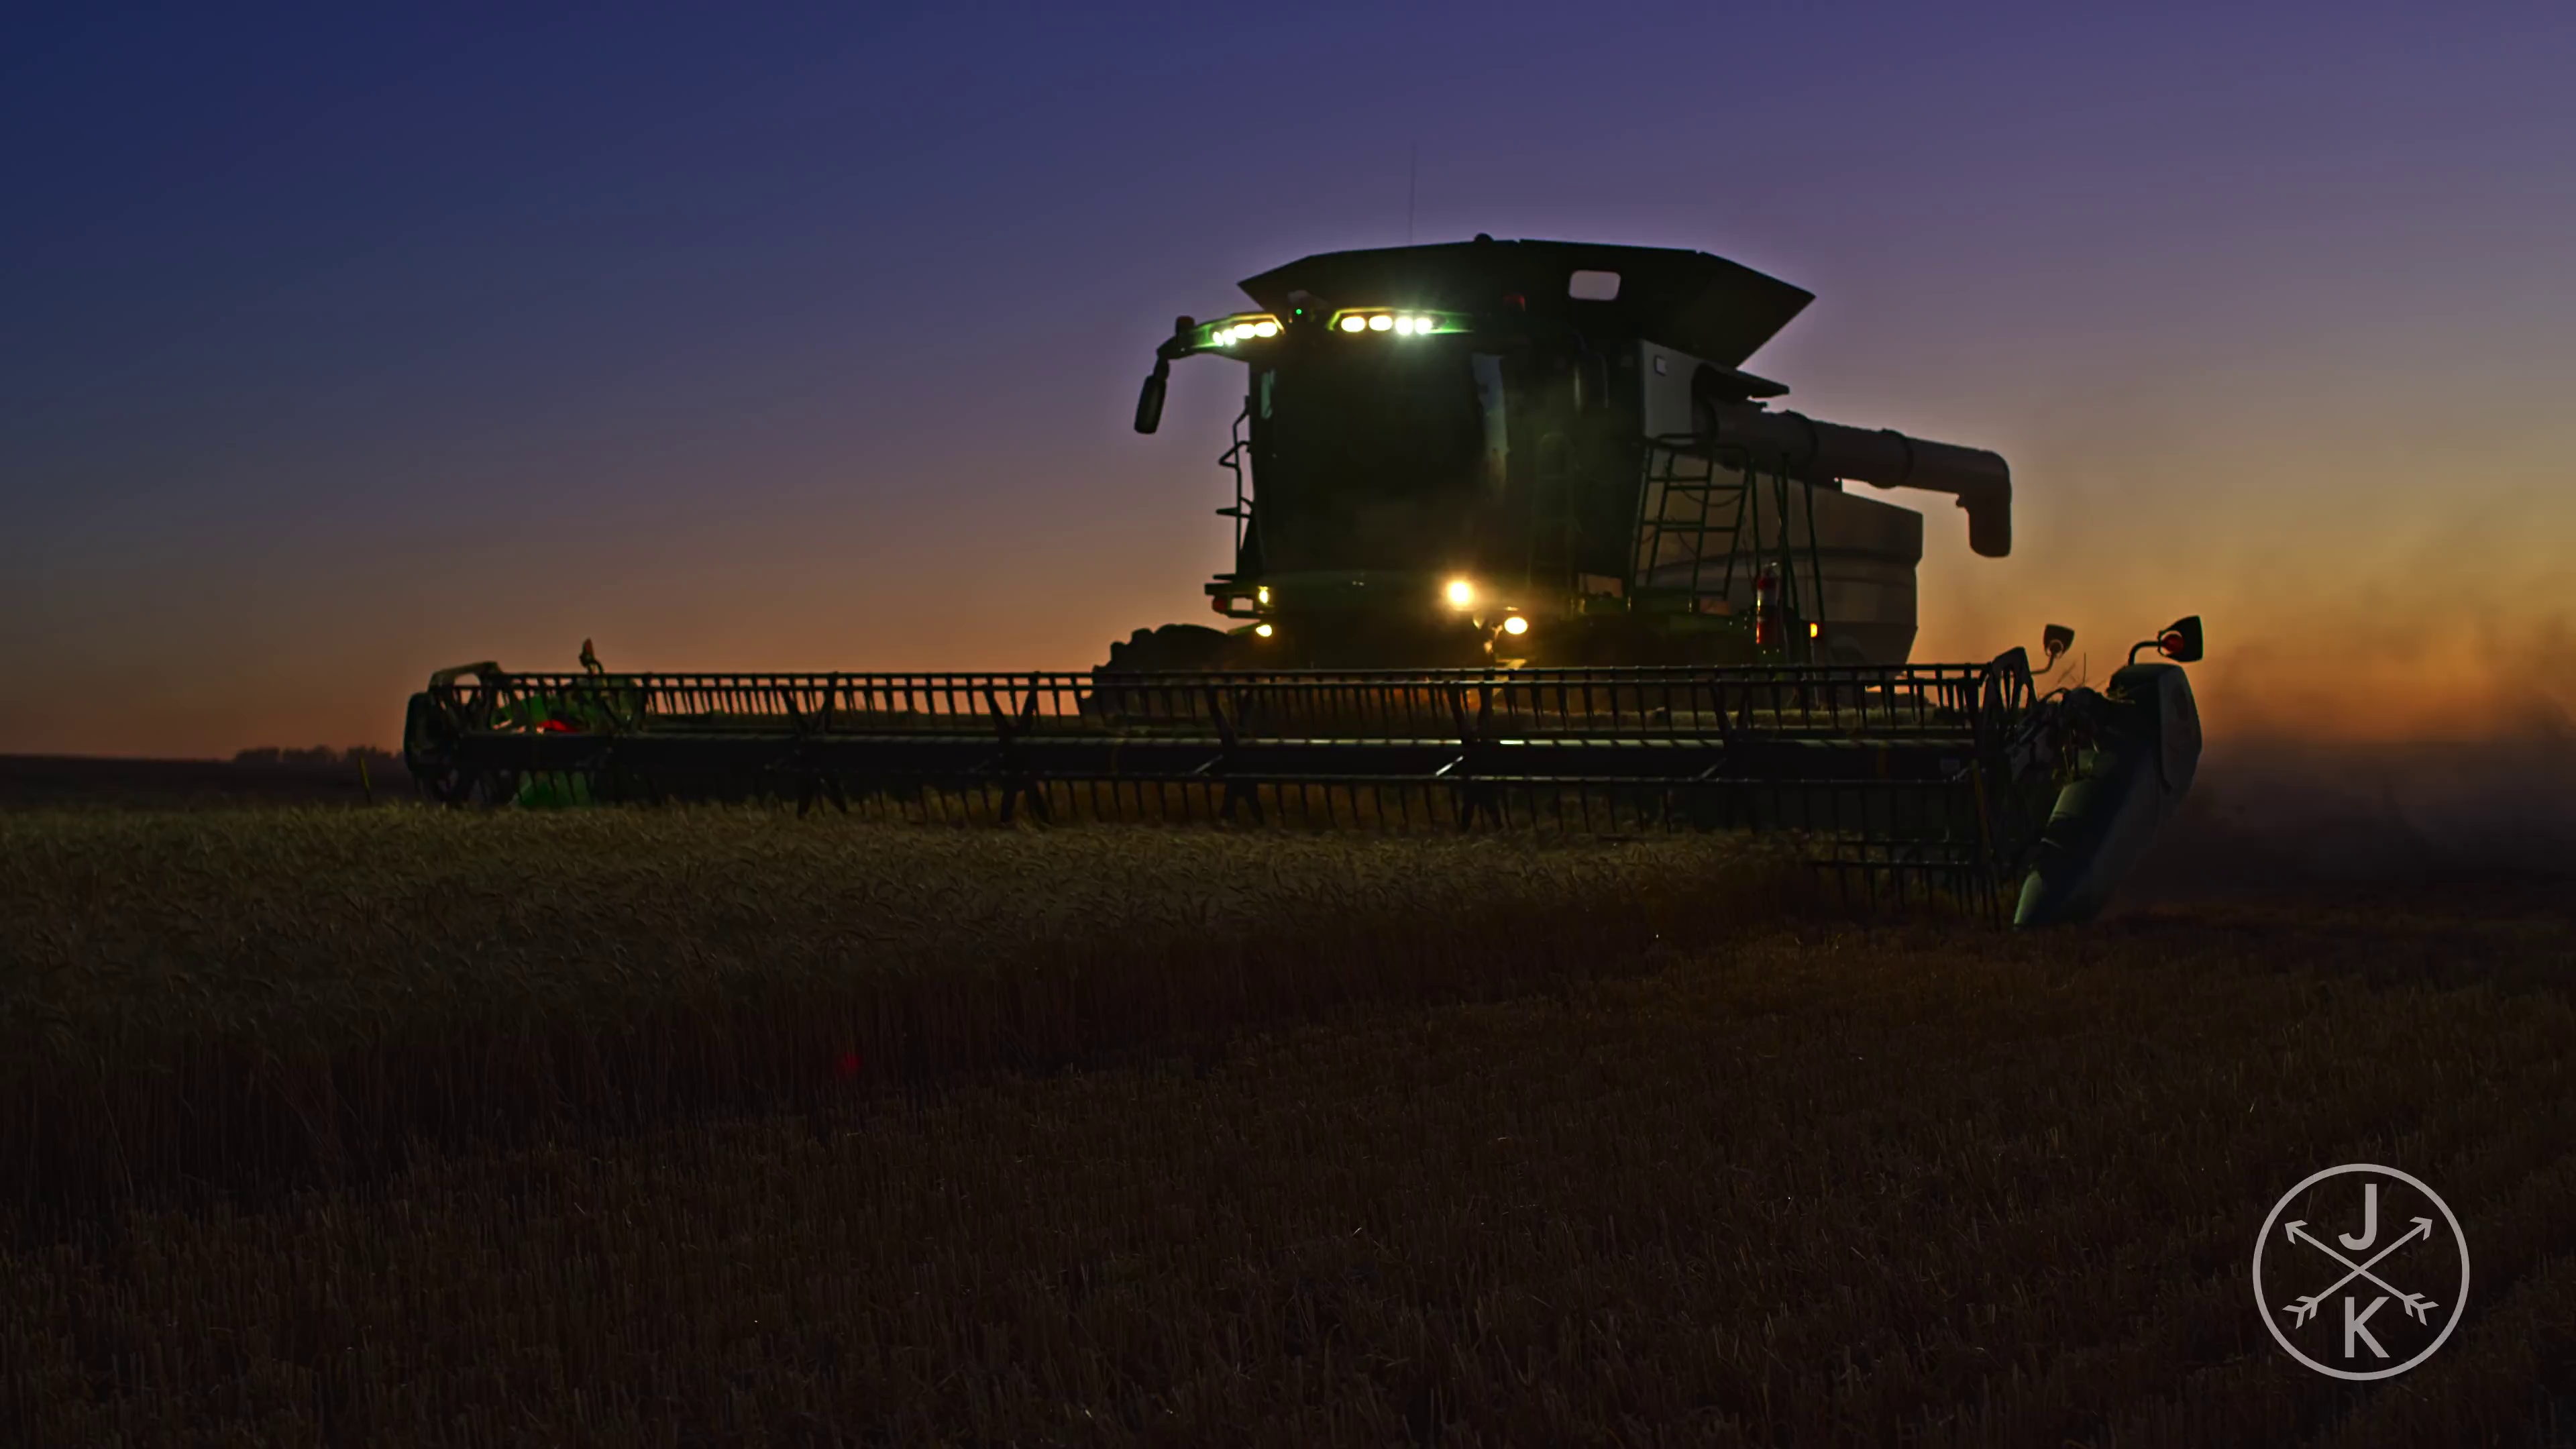}
        \caption{Video 5}
    \end{subfigure}
    % Video 6
    \begin{subfigure}[b]{0.3\textwidth}
        \centering
        \includegraphics[width=\textwidth]{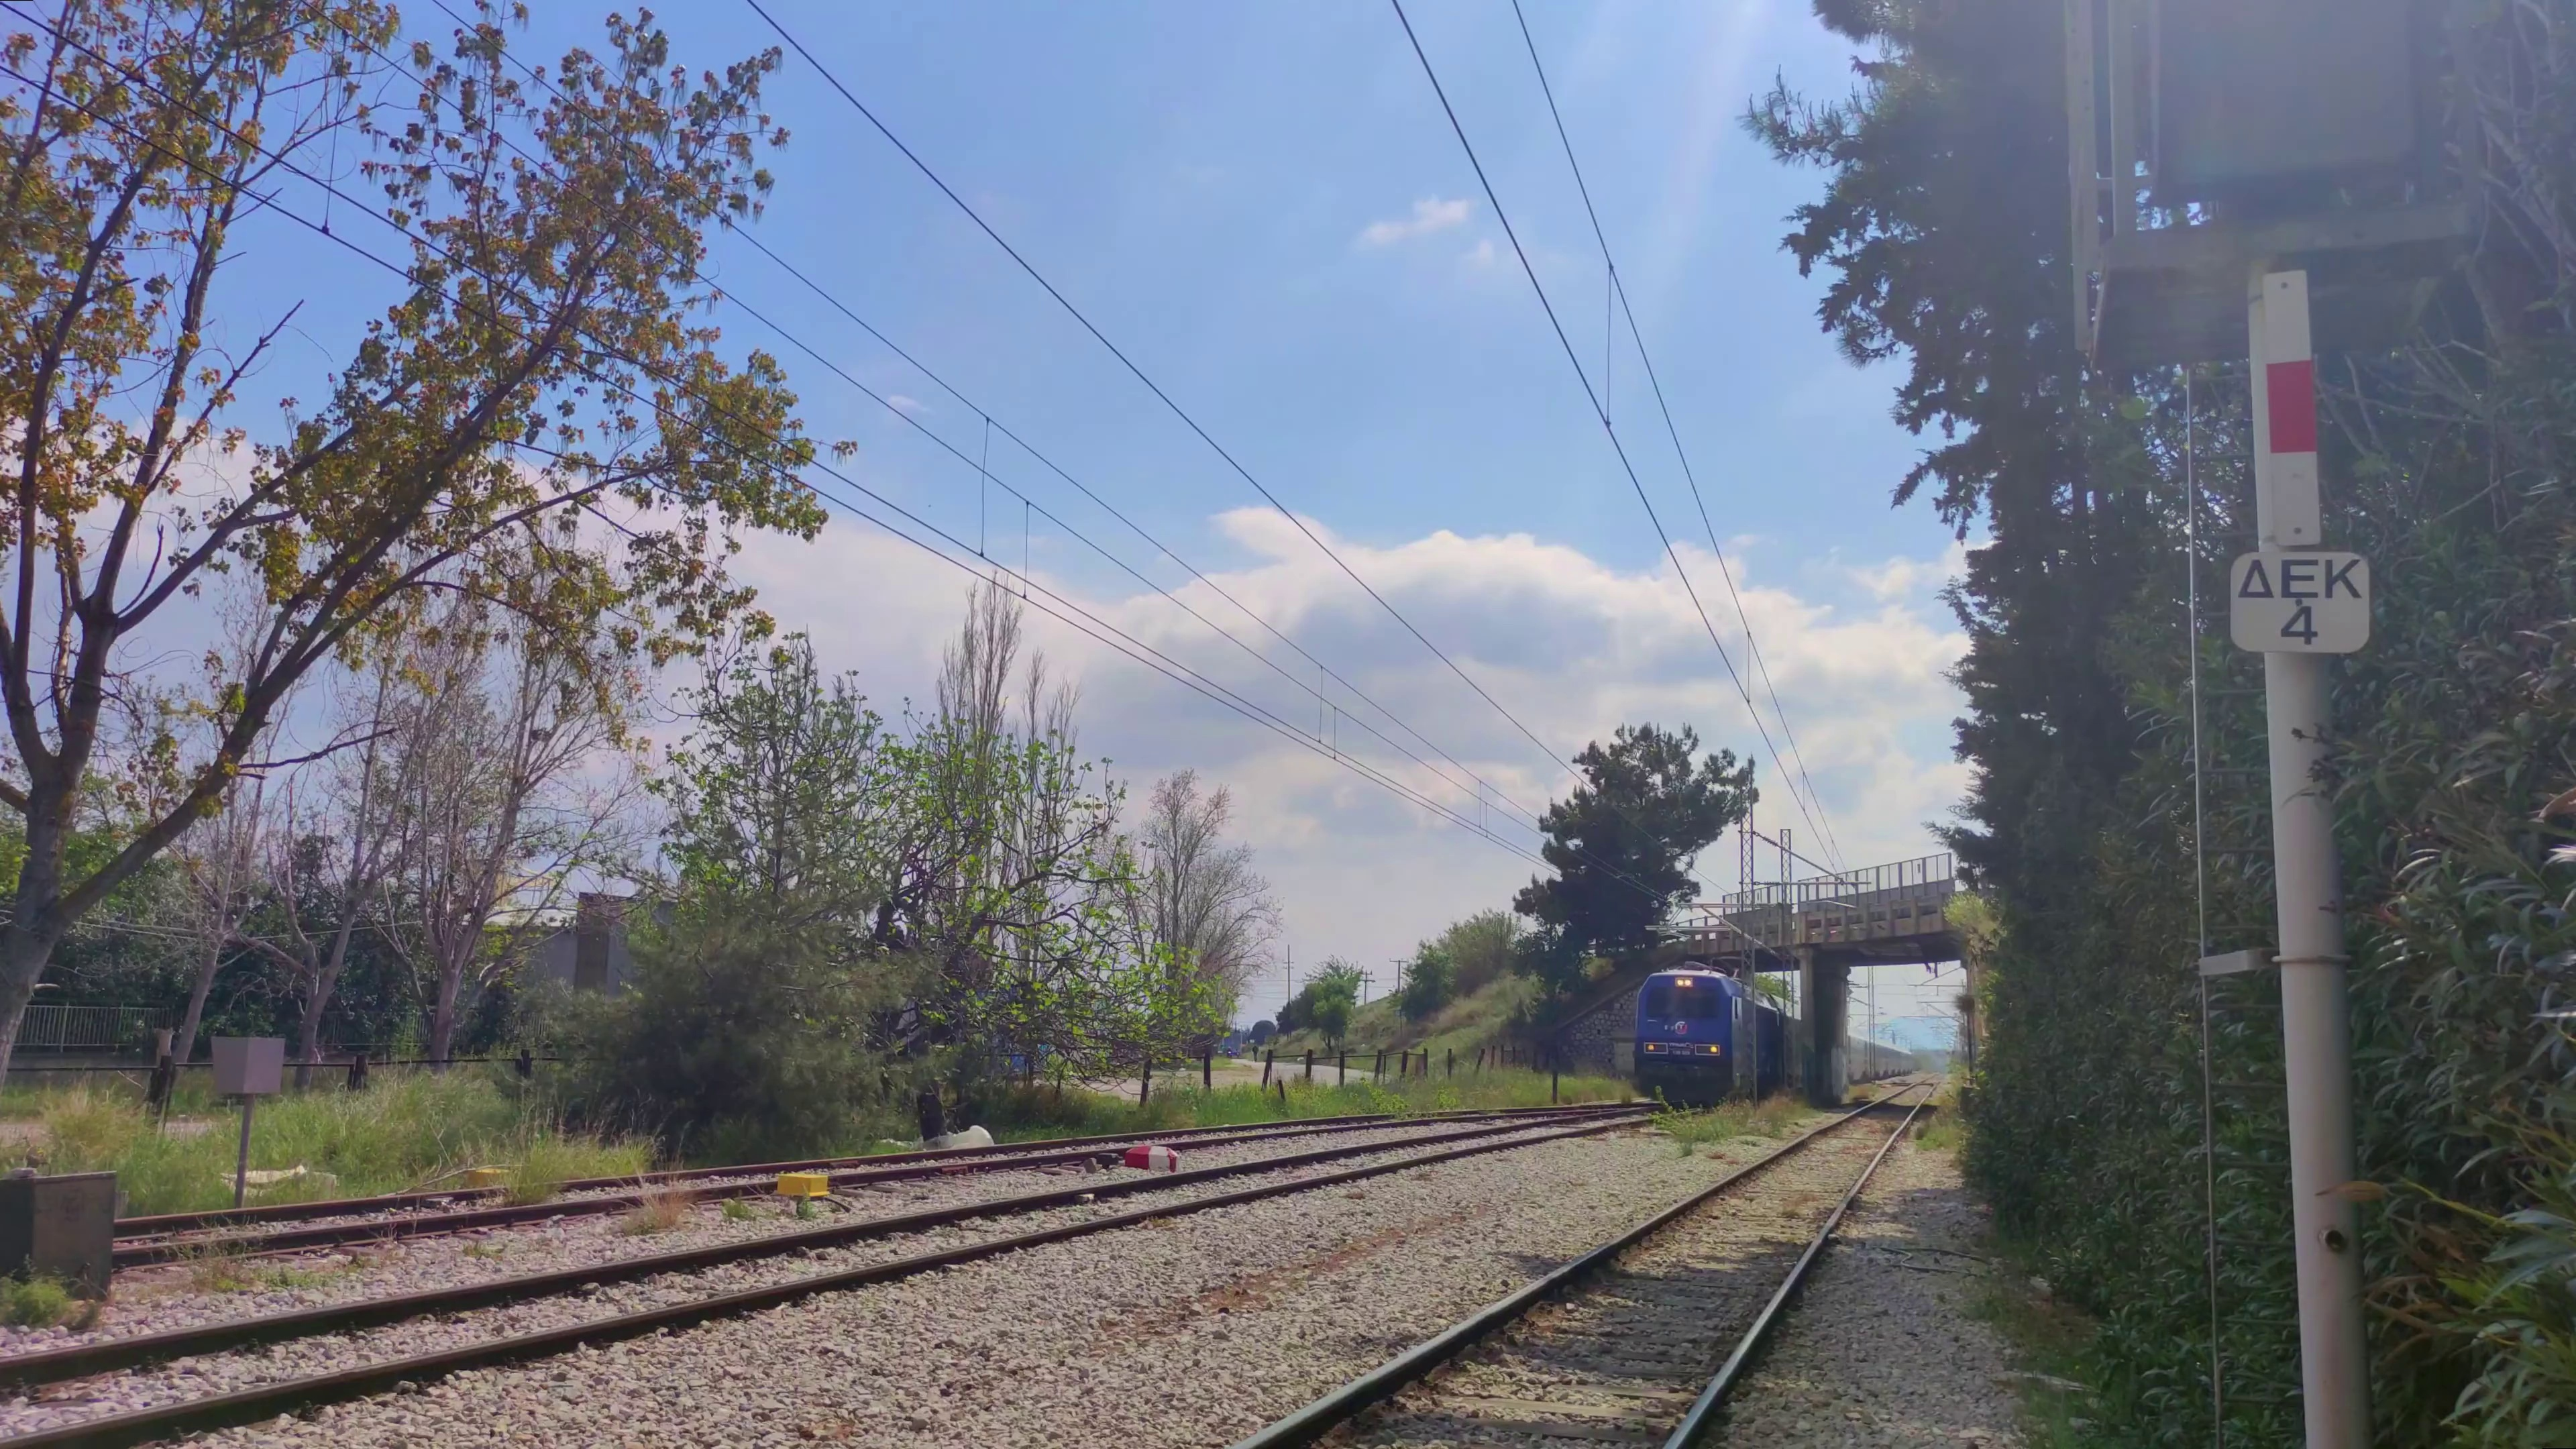}
        \caption{Video 6}
    \end{subfigure}
    
    \vspace{0.5cm}
    
    % Video 7
    \begin{subfigure}[b]{0.3\textwidth}
        \centering
        \includegraphics[width=\textwidth]{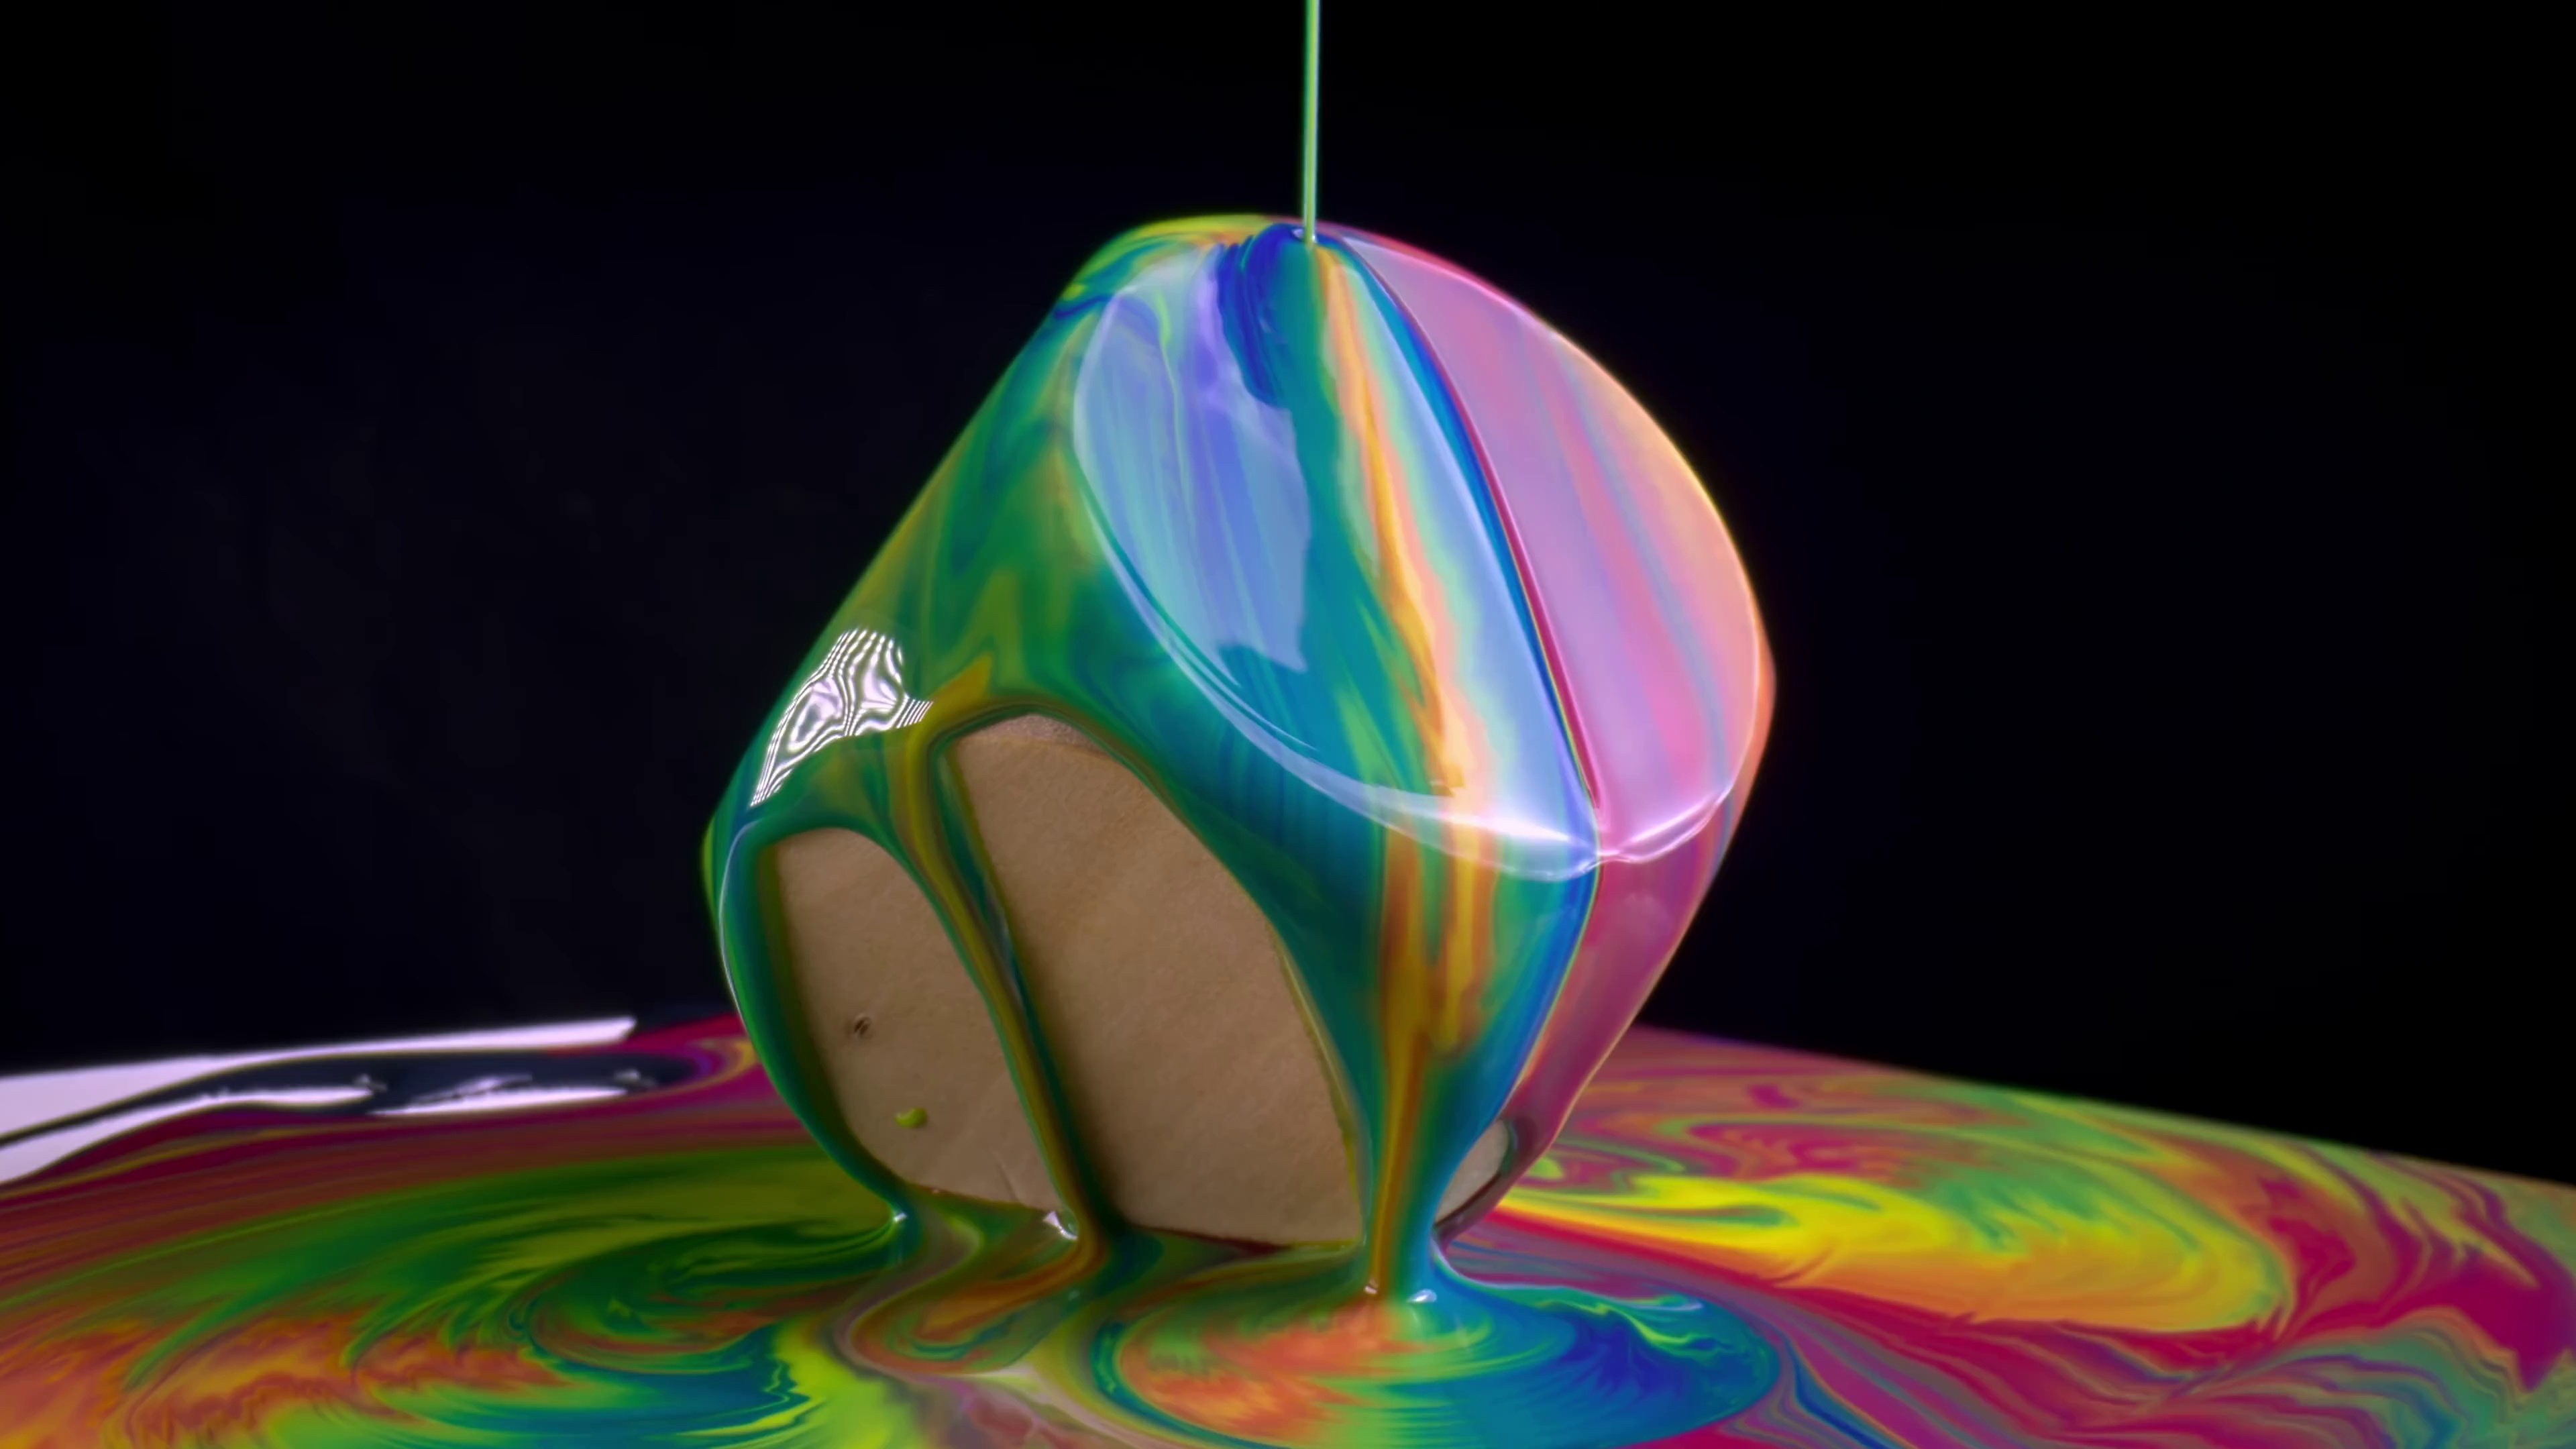}
        \caption{Video 7}
    \end{subfigure}
    % Video 8
    \begin{subfigure}[b]{0.3\textwidth}
        \centering
        \includegraphics[width=\textwidth]{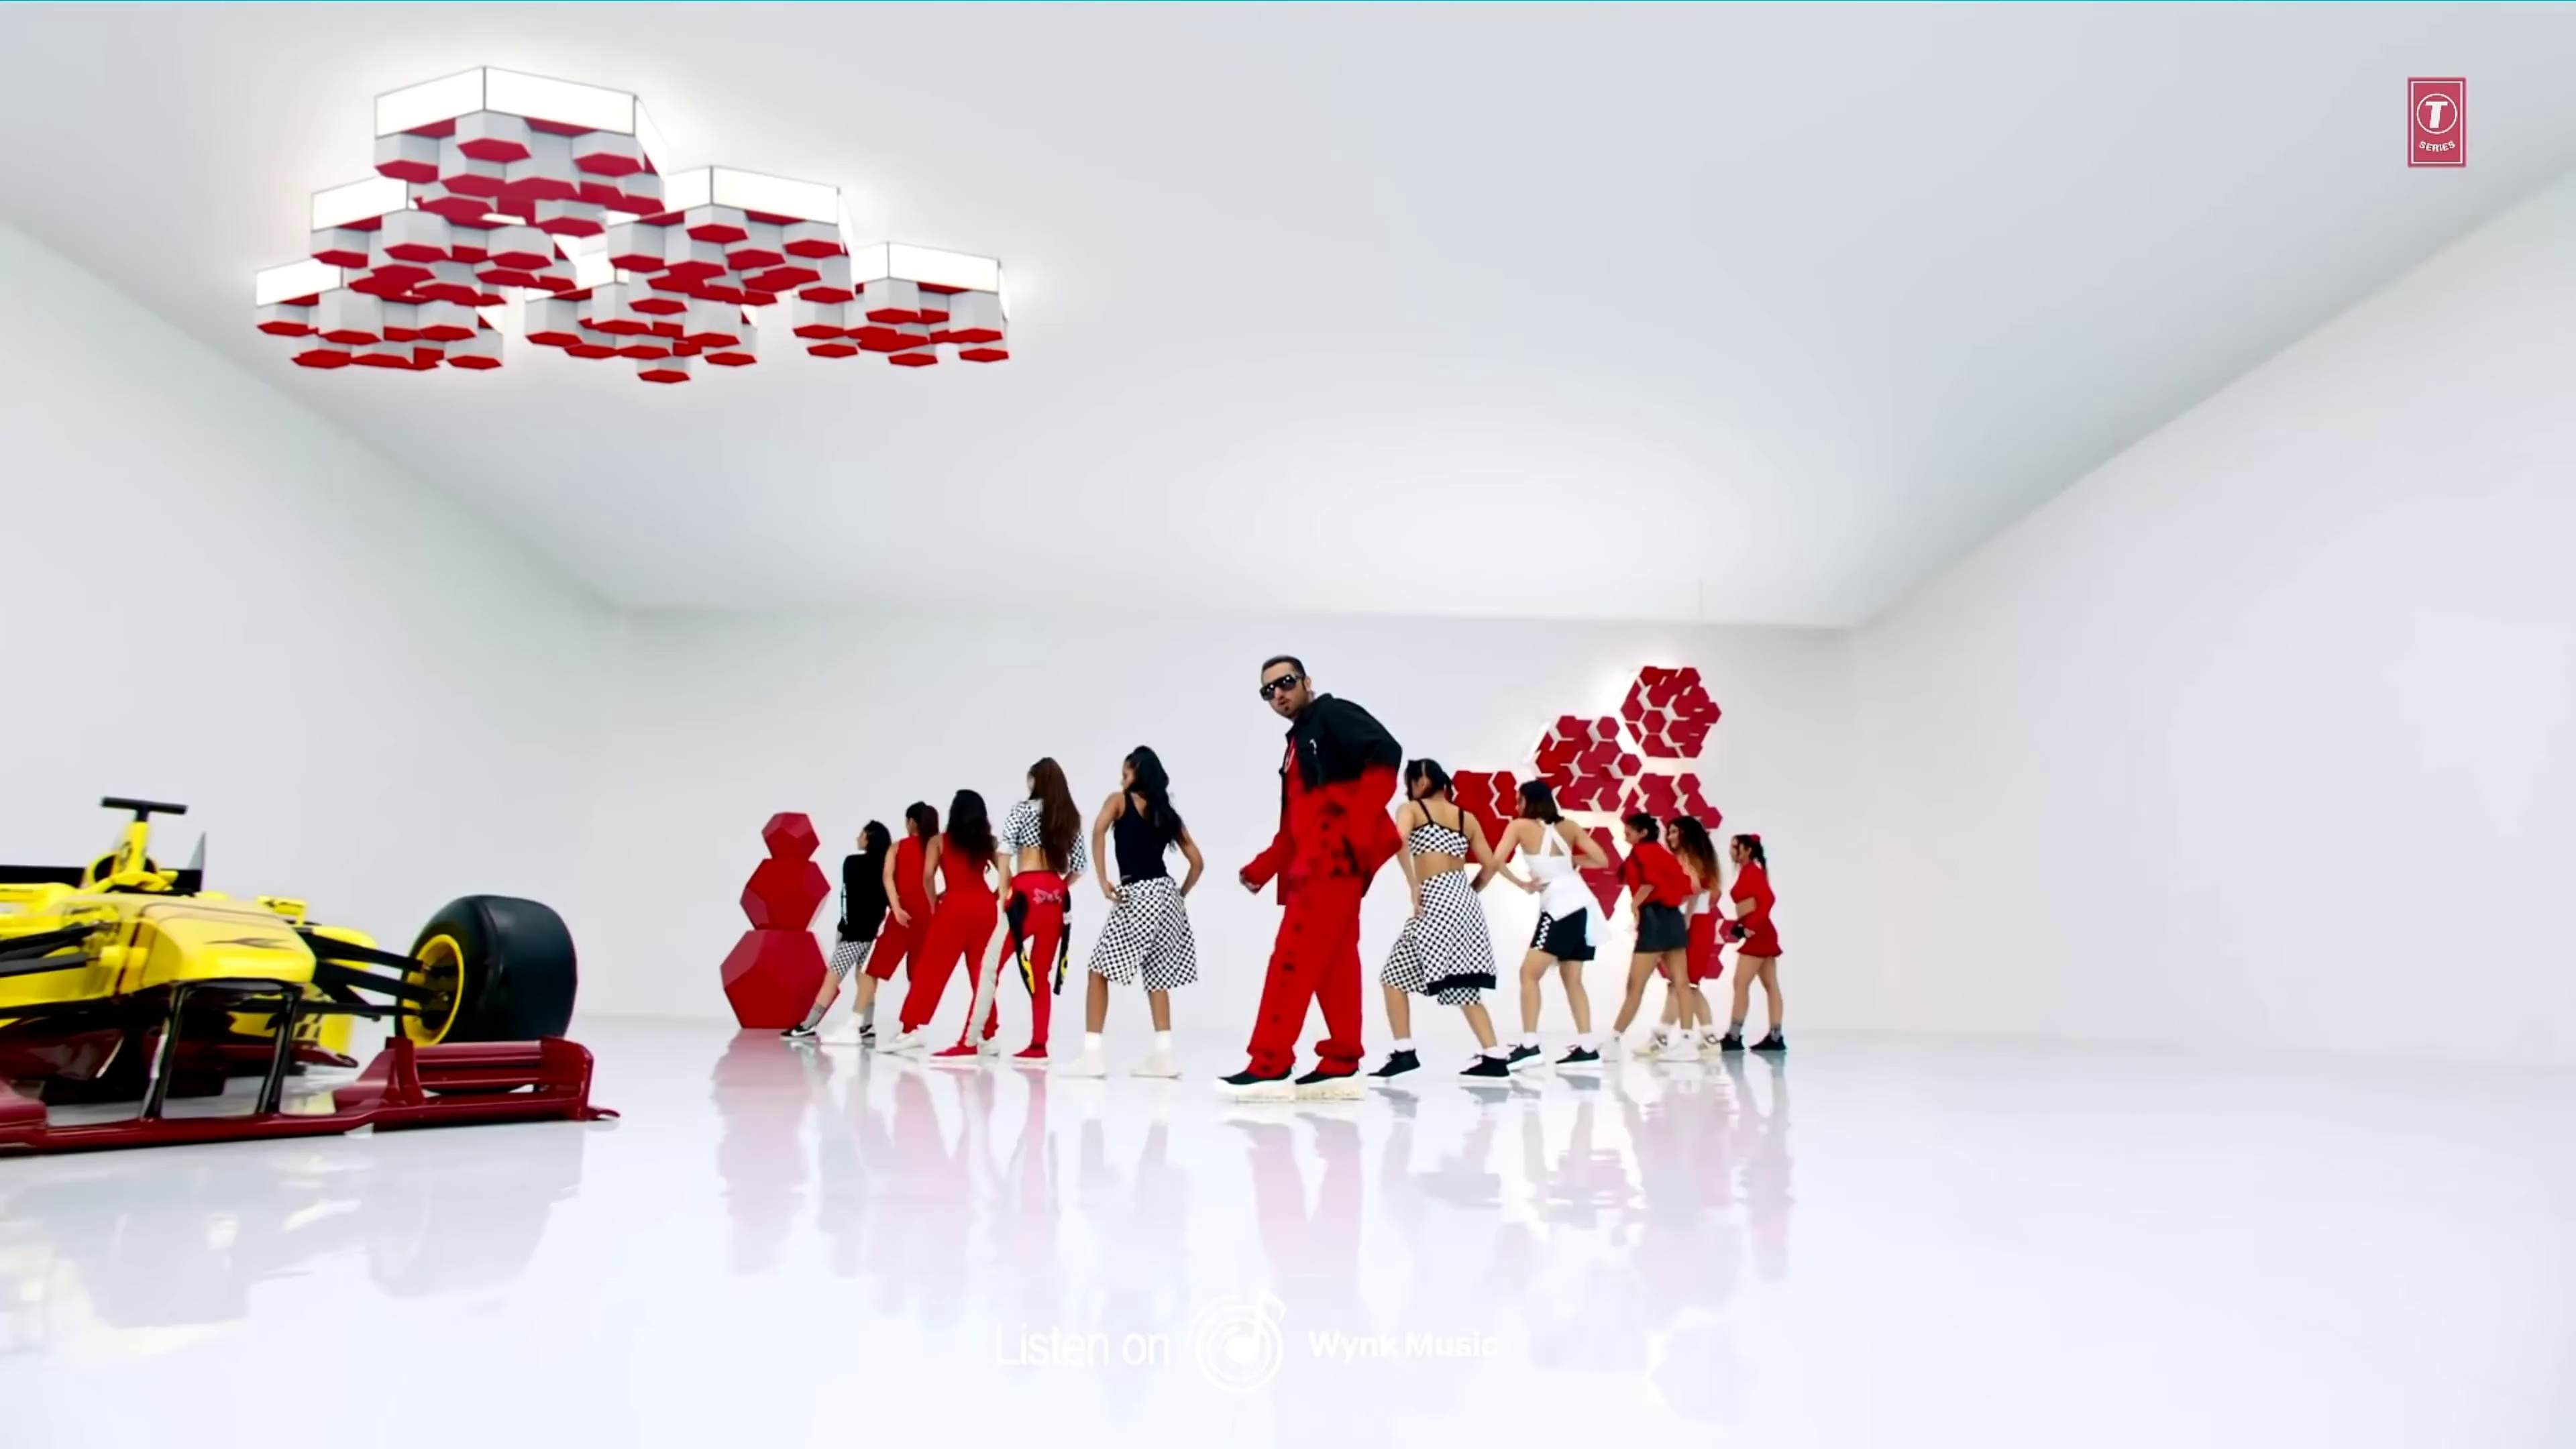}
        \caption{Video 8}
    \end{subfigure}
    % Video 9
    \begin{subfigure}[b]{0.3\textwidth}
        \centering
        \includegraphics[width=\textwidth]{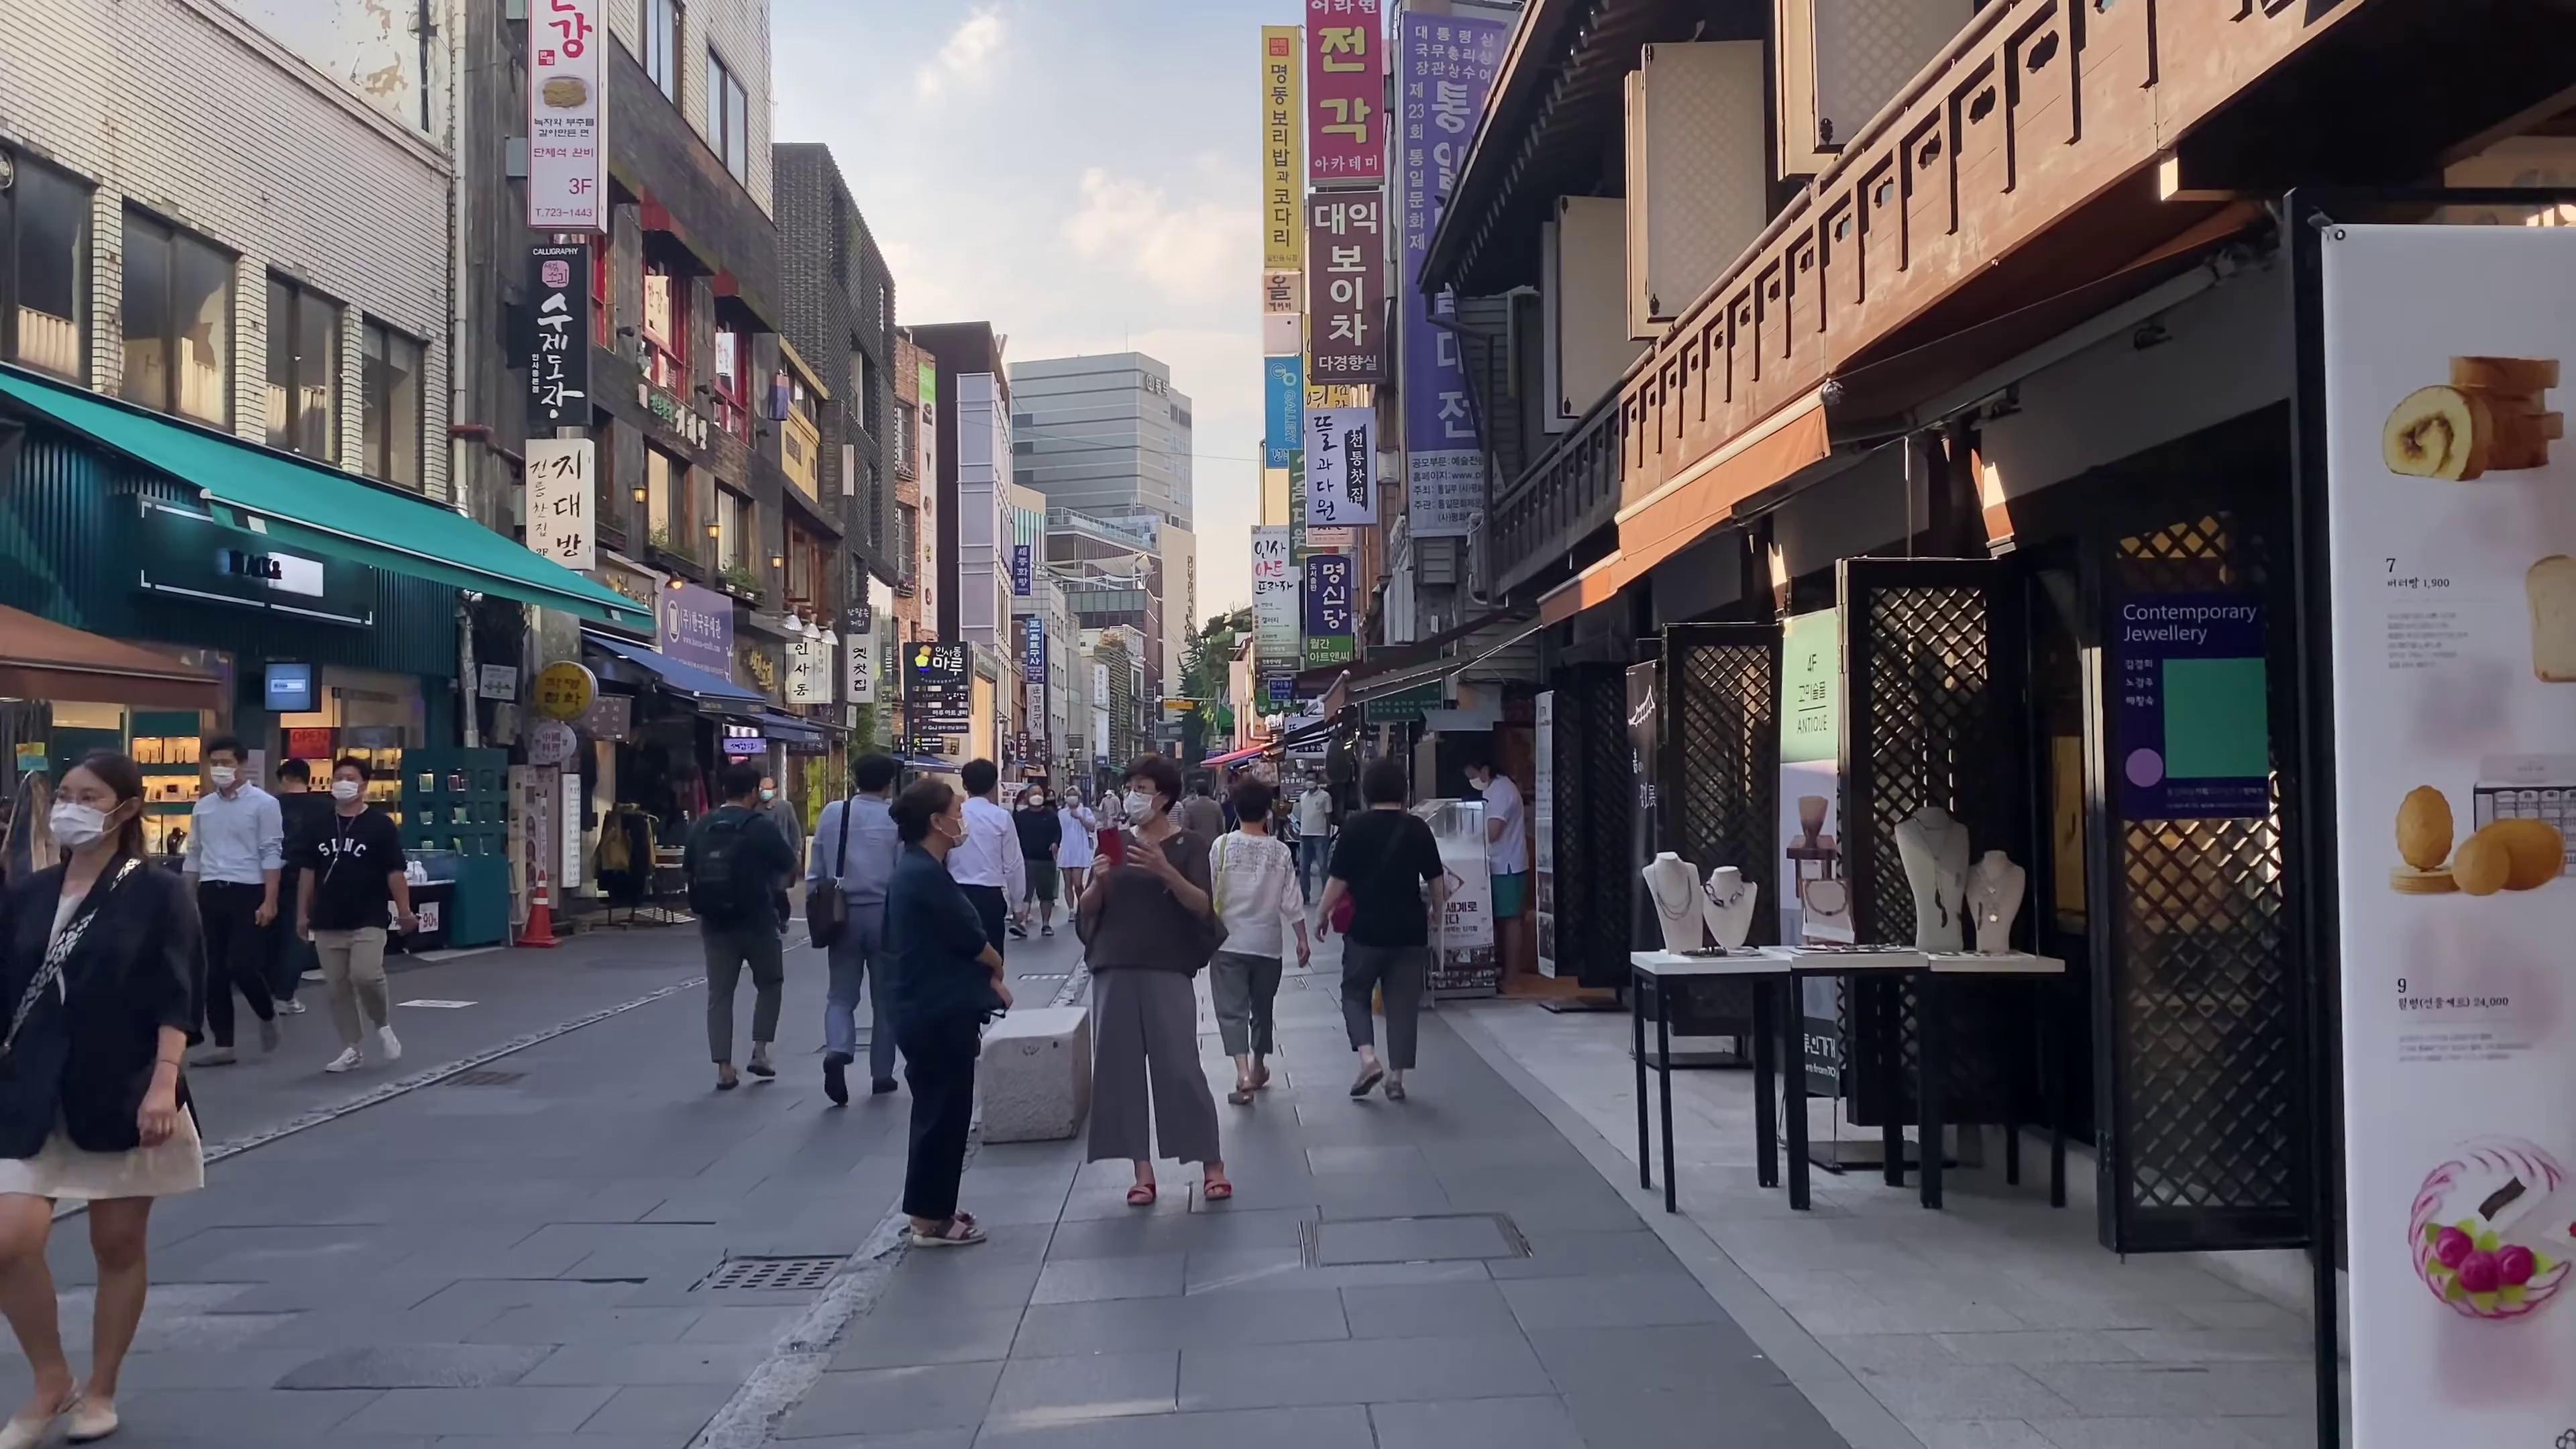}
        \caption{Video 9}
    \end{subfigure}

    \vspace{0.5cm}
    
    % Video 10
    \begin{subfigure}[b]{0.3\textwidth}
        \centering
        \includegraphics[width=\textwidth]{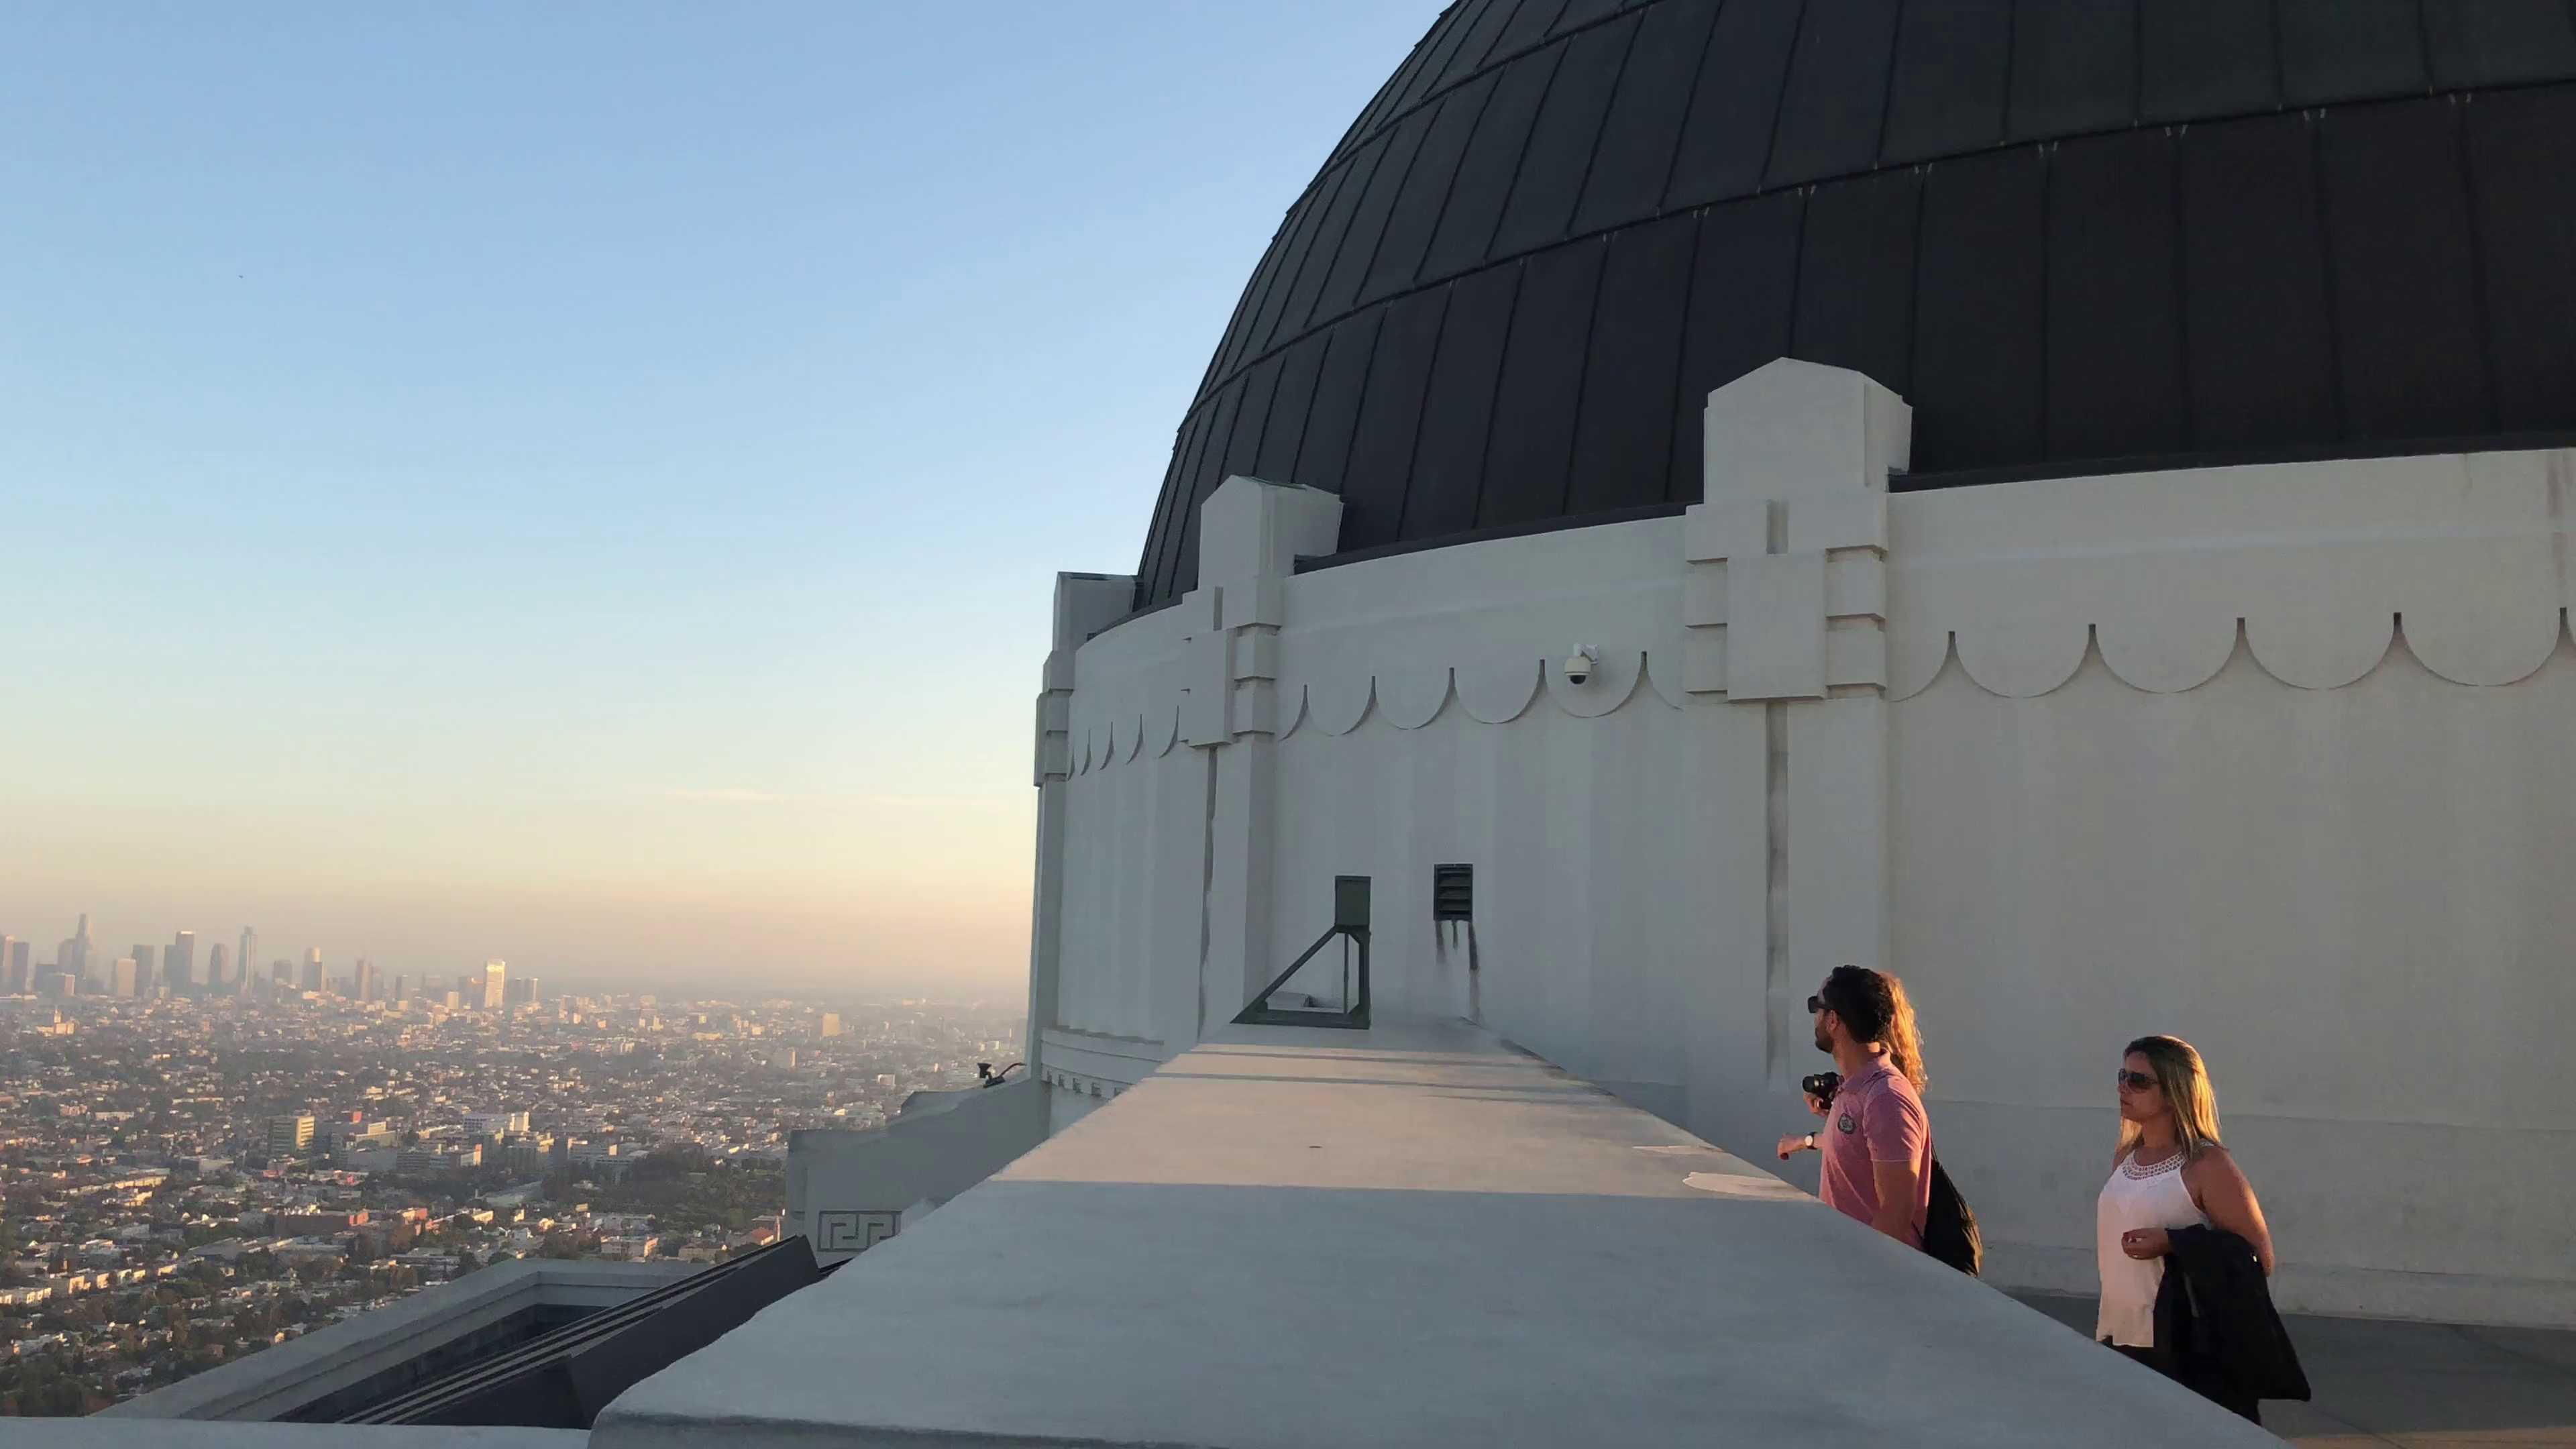}
        \caption{Video 10}
    \end{subfigure}

    \caption{\textbf{Examples of video frames from Video 1 to Video 10 used in the evaluation.}}
    \label{fig:video_examples}
\end{figure*}

\subsection{Training and Evaluation Details}
We extract distortion-related features from 20 randomly cropped patches, each with a resolution of \(384 \times 384\). The same patch positions are used across all frames within each video. During training, a single patch selected randomly from these 20 is processed through the diffusion feature extractor to capture the distortion-related features. In contrast, for inference, all 20 patches are processed to extract these features, which are then input into the downstream VQA network. The final video quality score is calculated by averaging the output scores from these 20 patches. The diffusion feature extractor comprises 1,699 million parameters, with only 363 million trainable parameters attributed to the Controller module. The VQA model itself contains an additional 95.29 million parameters. In terms of computational efficiency, the inference time for the diffusion feature extractor is 1.03 seconds per frame, while the VQA model processes each input in 0.807 seconds on a single Nvidia V100 GPU. Regarding computational complexity, the diffusion feature extractor requires 130.63 GFLOPs, whereas the VQA model demands 92.23 GFLOPs.

Some results presented in Tables 1 through 5 of the main paper are sourced from~\cite{wu2022disentangling,wu2023towards,lu2024kvq, liu2024scaling,mi2024clif,wu2023q}. Moreover, in Figure 7 of the main paper, we showcase t-SNE results highlighting semantic and distortion representations from ViT-L/16 and the diffusion feature extractor. To complement these results, \figref{fig:distortion_examples} and \figref{fig:video_examples} provide representative examples.

\subsection{Evaluation Metrics}
In our evaluation, we employ two metrics to assess the performance of our model: Spearman's Rank-Order Correlation Coefficient (SRCC) and Pearson's Linear Correlation Coefficient (PLCC).

PLCC evaluates the degree of linear correlation between the predicted and ground truth quality scores. It measures how closely the predictions align with the true values on a linear scale, making it sensitive to numerical differences. 

SRCC, on the other hand, assesses the monotonic relationship between two datasets, focusing on the rank order of the data rather than their actual values. This makes SRCC robust to outliers and skewed distributions. Both metrics produce values ranging from $-1$ to $1$, where a score of $1$ signifies perfect correlation, $-1$ indicates perfect inverse correlation, and $0$ reflects no correlation. Higher absolute values for these metrics indicate better model performance, with positive values demonstrating strong agreement with the ground truth.

For PLCC, let $s_i$ and $\hat{s}_i$ denote the ground truth and predicted quality scores for the $i$-th image, respectively. Let $\mu_{s_i}$ and $\mu_{\hat{s}_i}$ represent their respective means, and $N$ the total number of test images. PLCC is defined as:
\begin{equation}
    \operatorname{PLCC} =\frac{\sum^{N}_{i=1}(s_i-\mu_{s_i})(\hat{s}_i-\mu_{\hat{s}_i})}{\sqrt{\sum^{N}_{i=1}(s_i-\mu_{s_i})^{2}}\sqrt{\sum^{N}_{i=1}(\hat{s}_i-\mu_{\hat{s}_i})^{2}}}.
\end{equation}

For SRCC, let $d_i$ represent the rank difference between the ground truth and predicted scores for the $i$-th test image. SRCC is calculated as:
\begin{equation}
    \operatorname{SRCC} =1-\frac{6\sum^{N}_{i=1}d^2_i}{N(N^2-1)}.
\end{equation}

Both metrics provide complementary insights into the model's performance, with higher values indicating greater accuracy and consistency with human judgments.

\clearpage
