# Supplementary material for: DiffVQA: Video Quality Assessment Using Diffusion Feature Extractor
Source: arXiv:2505.03261 source file (2025-05-06)
Supplement: Supplementary file 2 [file dataset.tex]

\section{Datasets}
We evaluate the proposed model on six widely recognized UGC VQA datasets: KoNViD-1k~\cite{hosu2017konstanz}, LIVE-VQC~\cite{hosu2017konstanz}, YouTube-UGC~\cite{wang2019youtube}, LSVQ~\cite{ying2021patch}, KVQ~\cite{lu2024kvq}, and Maxwell~\cite{wu2023exploring}. Examples of video frames from each dataset are shown in \figref{fig:dataset-examples}. The KoNViD-1k dataset contains 1,200 videos sampled from a wide variety of real-world scenes, providing diverse visual content. The LIVE-VQC dataset includes 585 videos captured in authentic settings, focusing on realistic and varied video quality challenges. The YouTube-UGC dataset, comprising 1,147 videos, is notably diverse, spanning 15 video categories such as animation, gaming, HDR, live music, and sports. The LSVQ dataset includes 39,076 videos, making it the largest UGC VQA dataset to date and a vital benchmark for VQA research. The KVQ dataset represents the first large-scale kaleidoscope short-form video database, consisting of 4,200 user-uploaded or processed videos from short-form UGC platforms. The Maxwell dataset contains 4,543 videos covering 16 dimensions, including 13 specific quality factors and 3 abstract quality ratings. It is split into a training set of 3,634 videos and a reserved test set of 909 videos, enabling comprehensive evaluation of multi-dimensional video quality attributes, particularly for dynamic and in-the-wild content.

\begin{figure*}[t]
    \centering
    \begin{subfigure}[b]{0.32\textwidth}
        \centering
        \includegraphics[width=\linewidth]{figures/all_images/dataset_sample/konvid_sample.png}
        \caption{KoNViD-1k}
        \label{fig:konvid-1k}
    \end{subfigure}
    \hfill
    \begin{subfigure}[b]{0.32\textwidth}
        \centering
        \includegraphics[width=\linewidth]{figures/all_images/dataset_sample/livevqc_sample.png}
        \caption{LIVE-VQC}
        \label{fig:live-vqc}
    \end{subfigure}
    \hfill
    \begin{subfigure}[b]{0.32\textwidth}
        \centering
        \includegraphics[width=\linewidth]{figures/all_images/dataset_sample/ytugc_sample.png}
        \caption{YouTube-UGC}
        \label{fig:youtube-ugc}
    \end{subfigure}
    \vspace{1em}
    \begin{subfigure}[b]{0.32\textwidth}
        \centering
        \includegraphics[width=\linewidth]{figures/all_images/dataset_sample/lsvq_sample.png}
        \caption{LSVQ}
        \label{fig:lsvq}
    \end{subfigure}
    \hfill
    \begin{subfigure}[b]{0.32\textwidth}
        \centering
        \includegraphics[width=\linewidth]{figures/all_images/dataset_sample/kvq_sample.png}
        \caption{KVQ}
        \label{fig:kvq}
    \end{subfigure}
    \hfill
    \begin{subfigure}[b]{0.32\textwidth}
        \centering
        \includegraphics[width=\linewidth]{figures/all_images/dataset_sample/maxwell_sample.png}
        \caption{Maxwell}
        \label{fig:maxwell}
    \end{subfigure}
    \caption{\textbf{Examples of video frames from the six evaluated datasets.} Each row contains three columns showing examples from different datasets: (a) KoNViD-1k~\cite{hosu2017konstanz}, (b) LIVE-VQC~\cite{hosu2017konstanz}, (c) YouTube-UGC~\cite{wang2019youtube}, (d) LSVQ~\cite{ying2021patch}, (e) KVQ~\cite{lu2024kvq}, and (f) Maxwell~\cite{wu2023exploring}.}
    \label{fig:dataset-examples}
\end{figure*}
