# Supplementary material for: DiffVQA: Video Quality Assessment Using Diffusion Feature Extractor
Source: arXiv:2505.03261 source file (2025-05-06)
Supplement: Supplementary file 4 [file implementation.tex]

\section{Implementation Details}

\begin{figure*}[t]
    \centering
    % Sharp
    \begin{subfigure}[b]{0.3\textwidth}
        \centering
        \includegraphics[width=\textwidth]{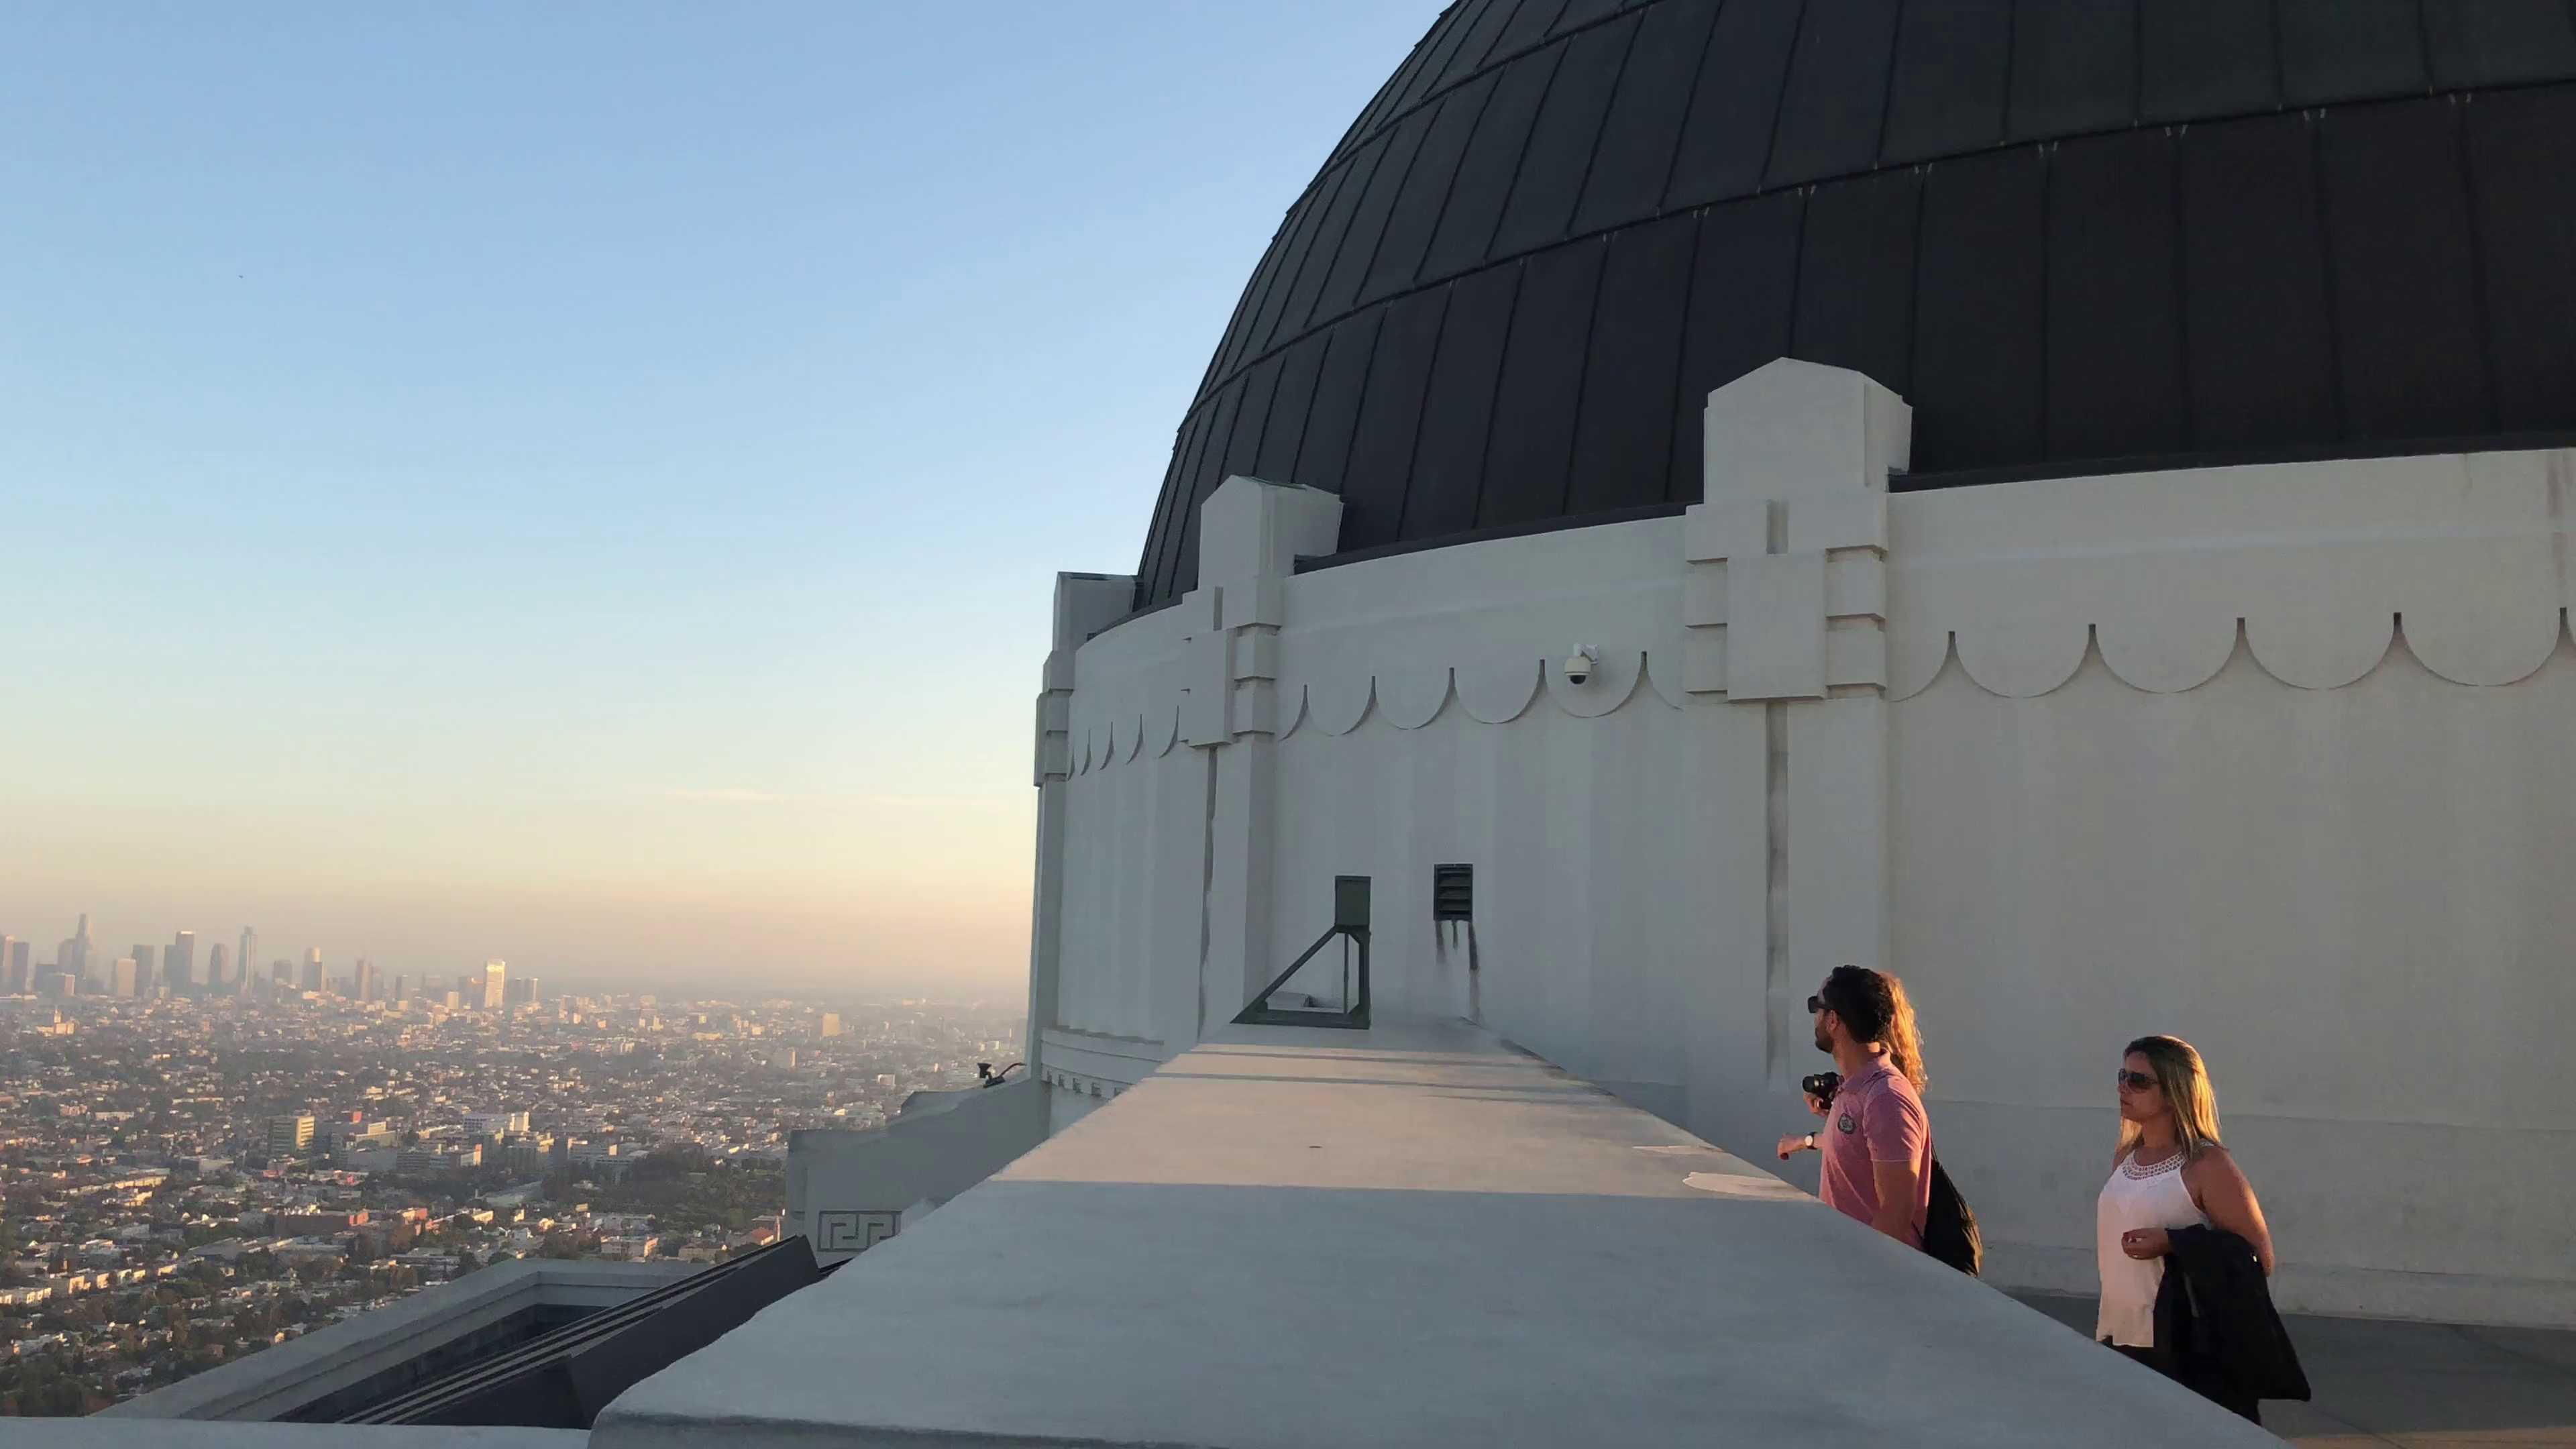}
        \caption{Sharp}
    \end{subfigure}
    % Gaussian Noise
    \begin{subfigure}[b]{0.3\textwidth}
        \centering
        \includegraphics[width=\textwidth]{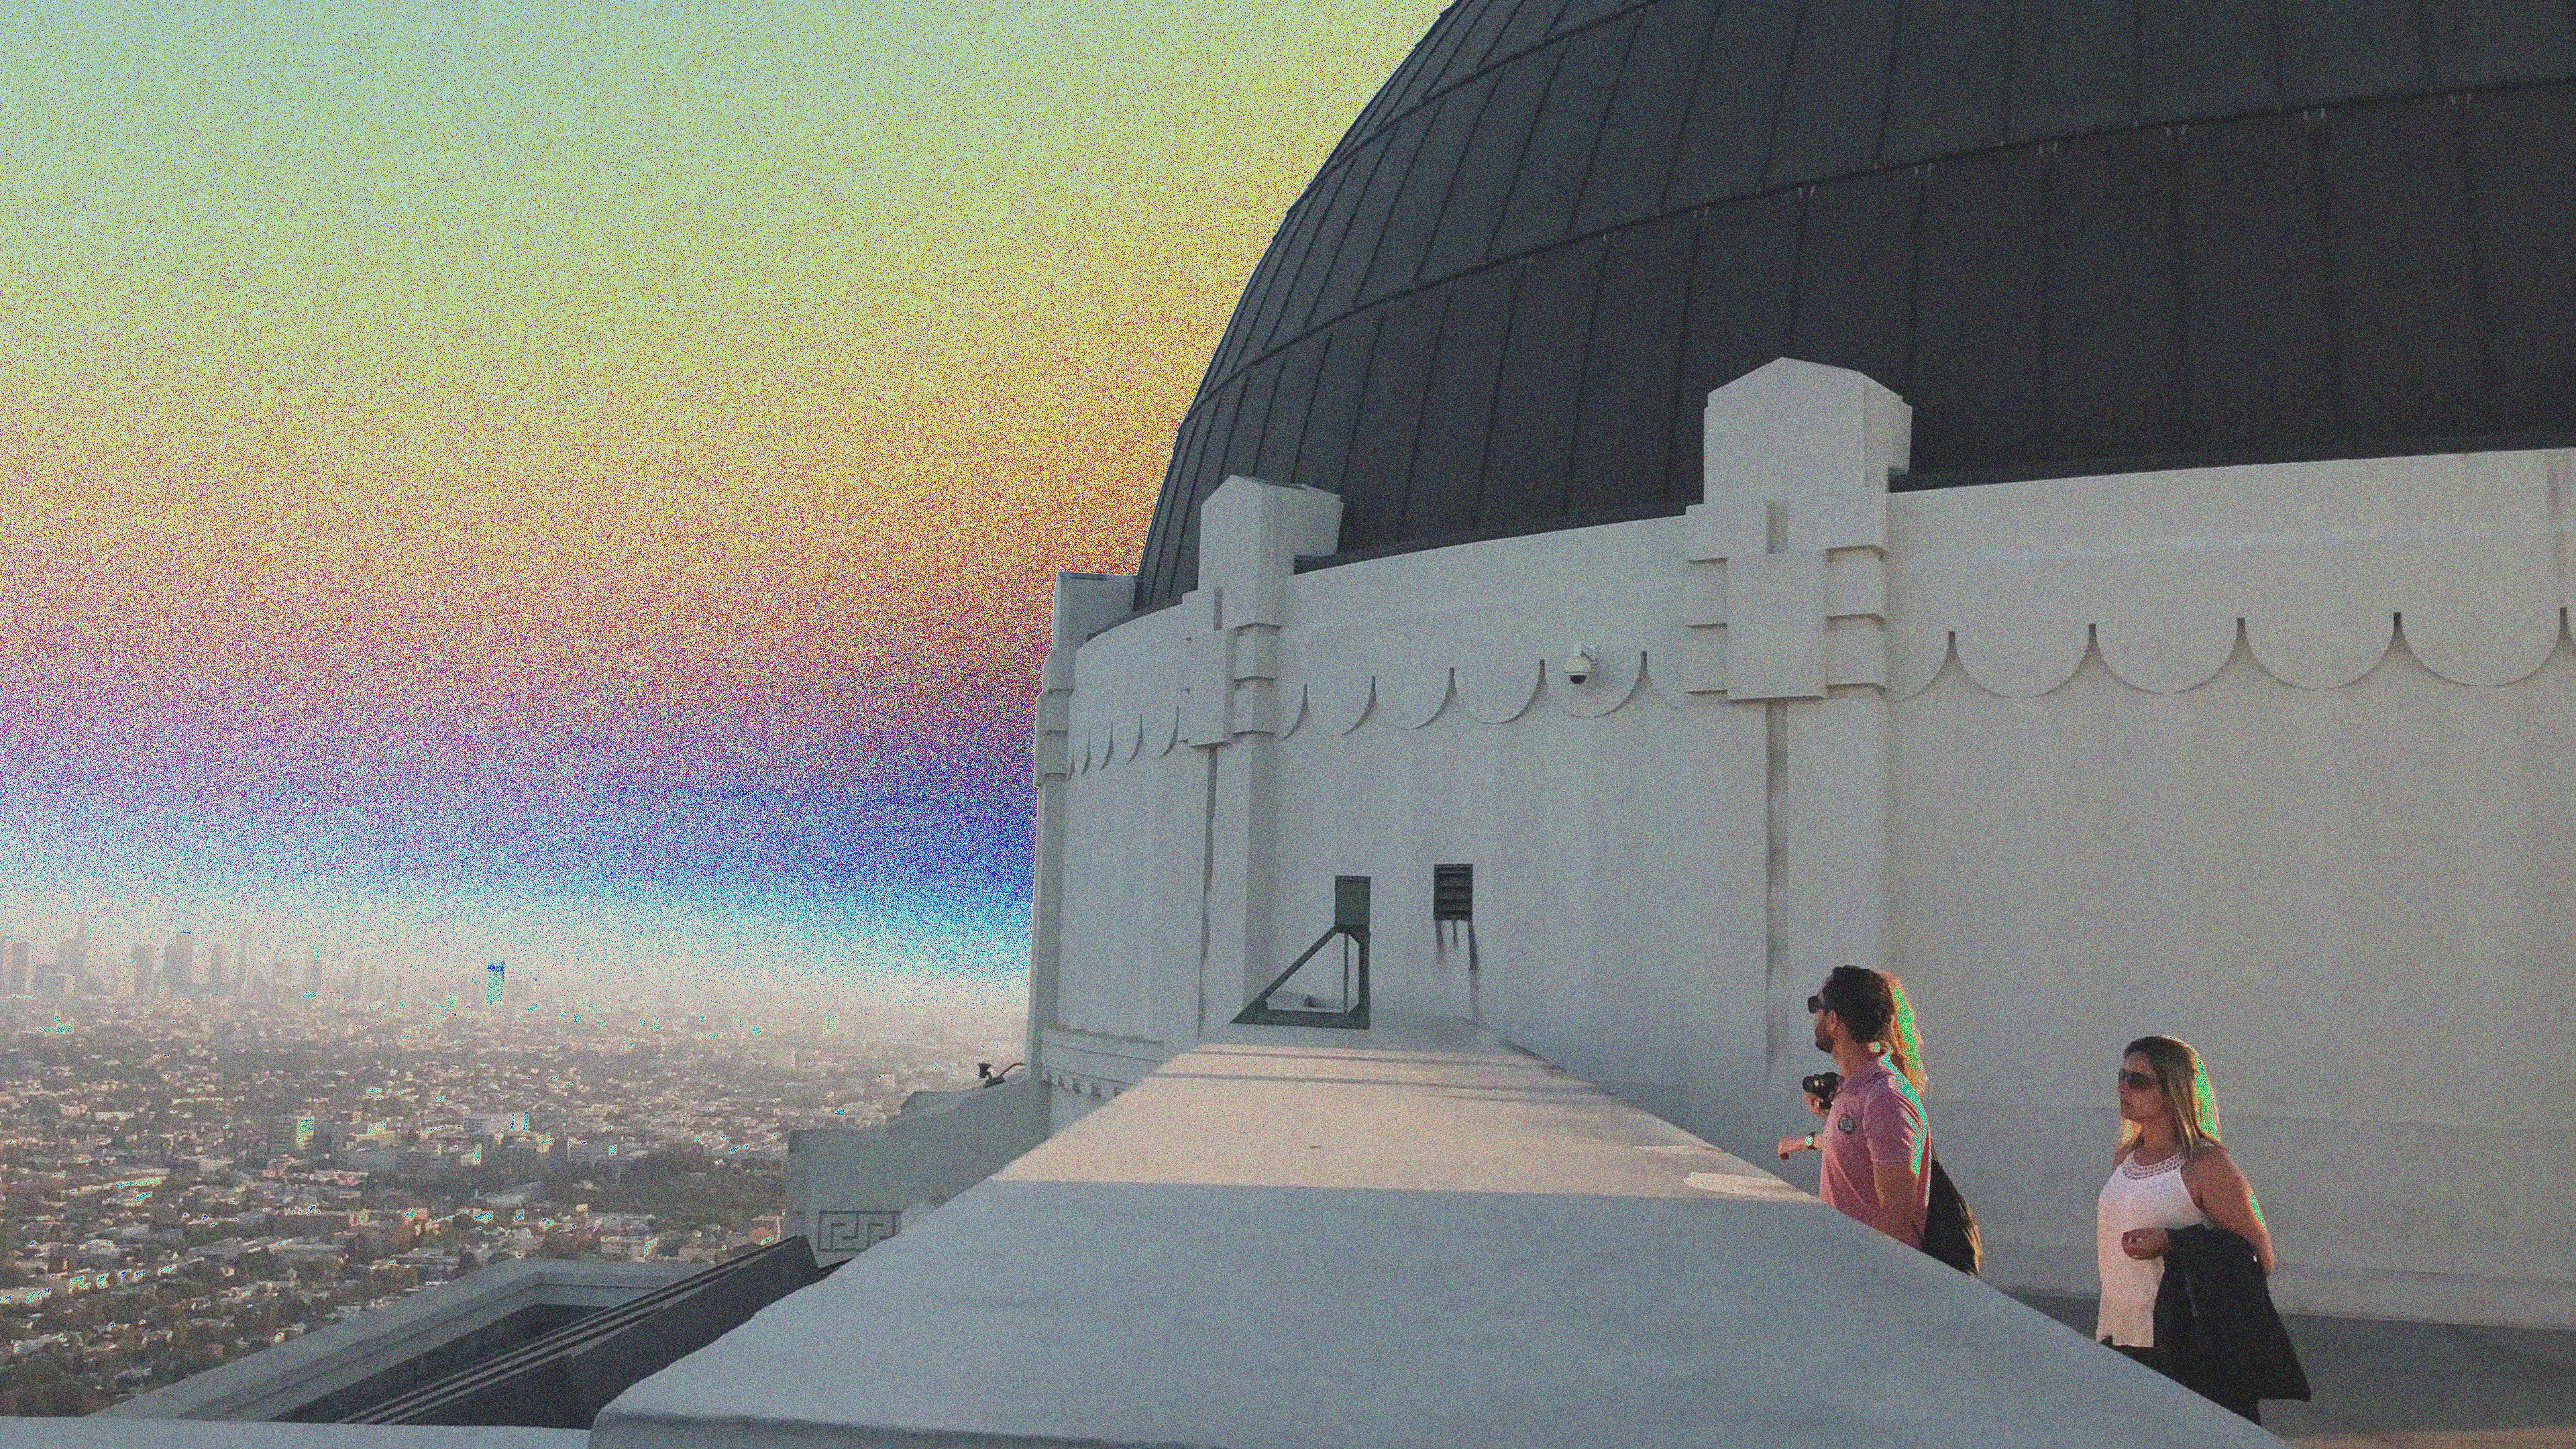}
        \caption{Gaussian Noise}
    \end{subfigure}
    % ISO Noise
    \begin{subfigure}[b]{0.3\textwidth}
        \centering
        \includegraphics[width=\textwidth]{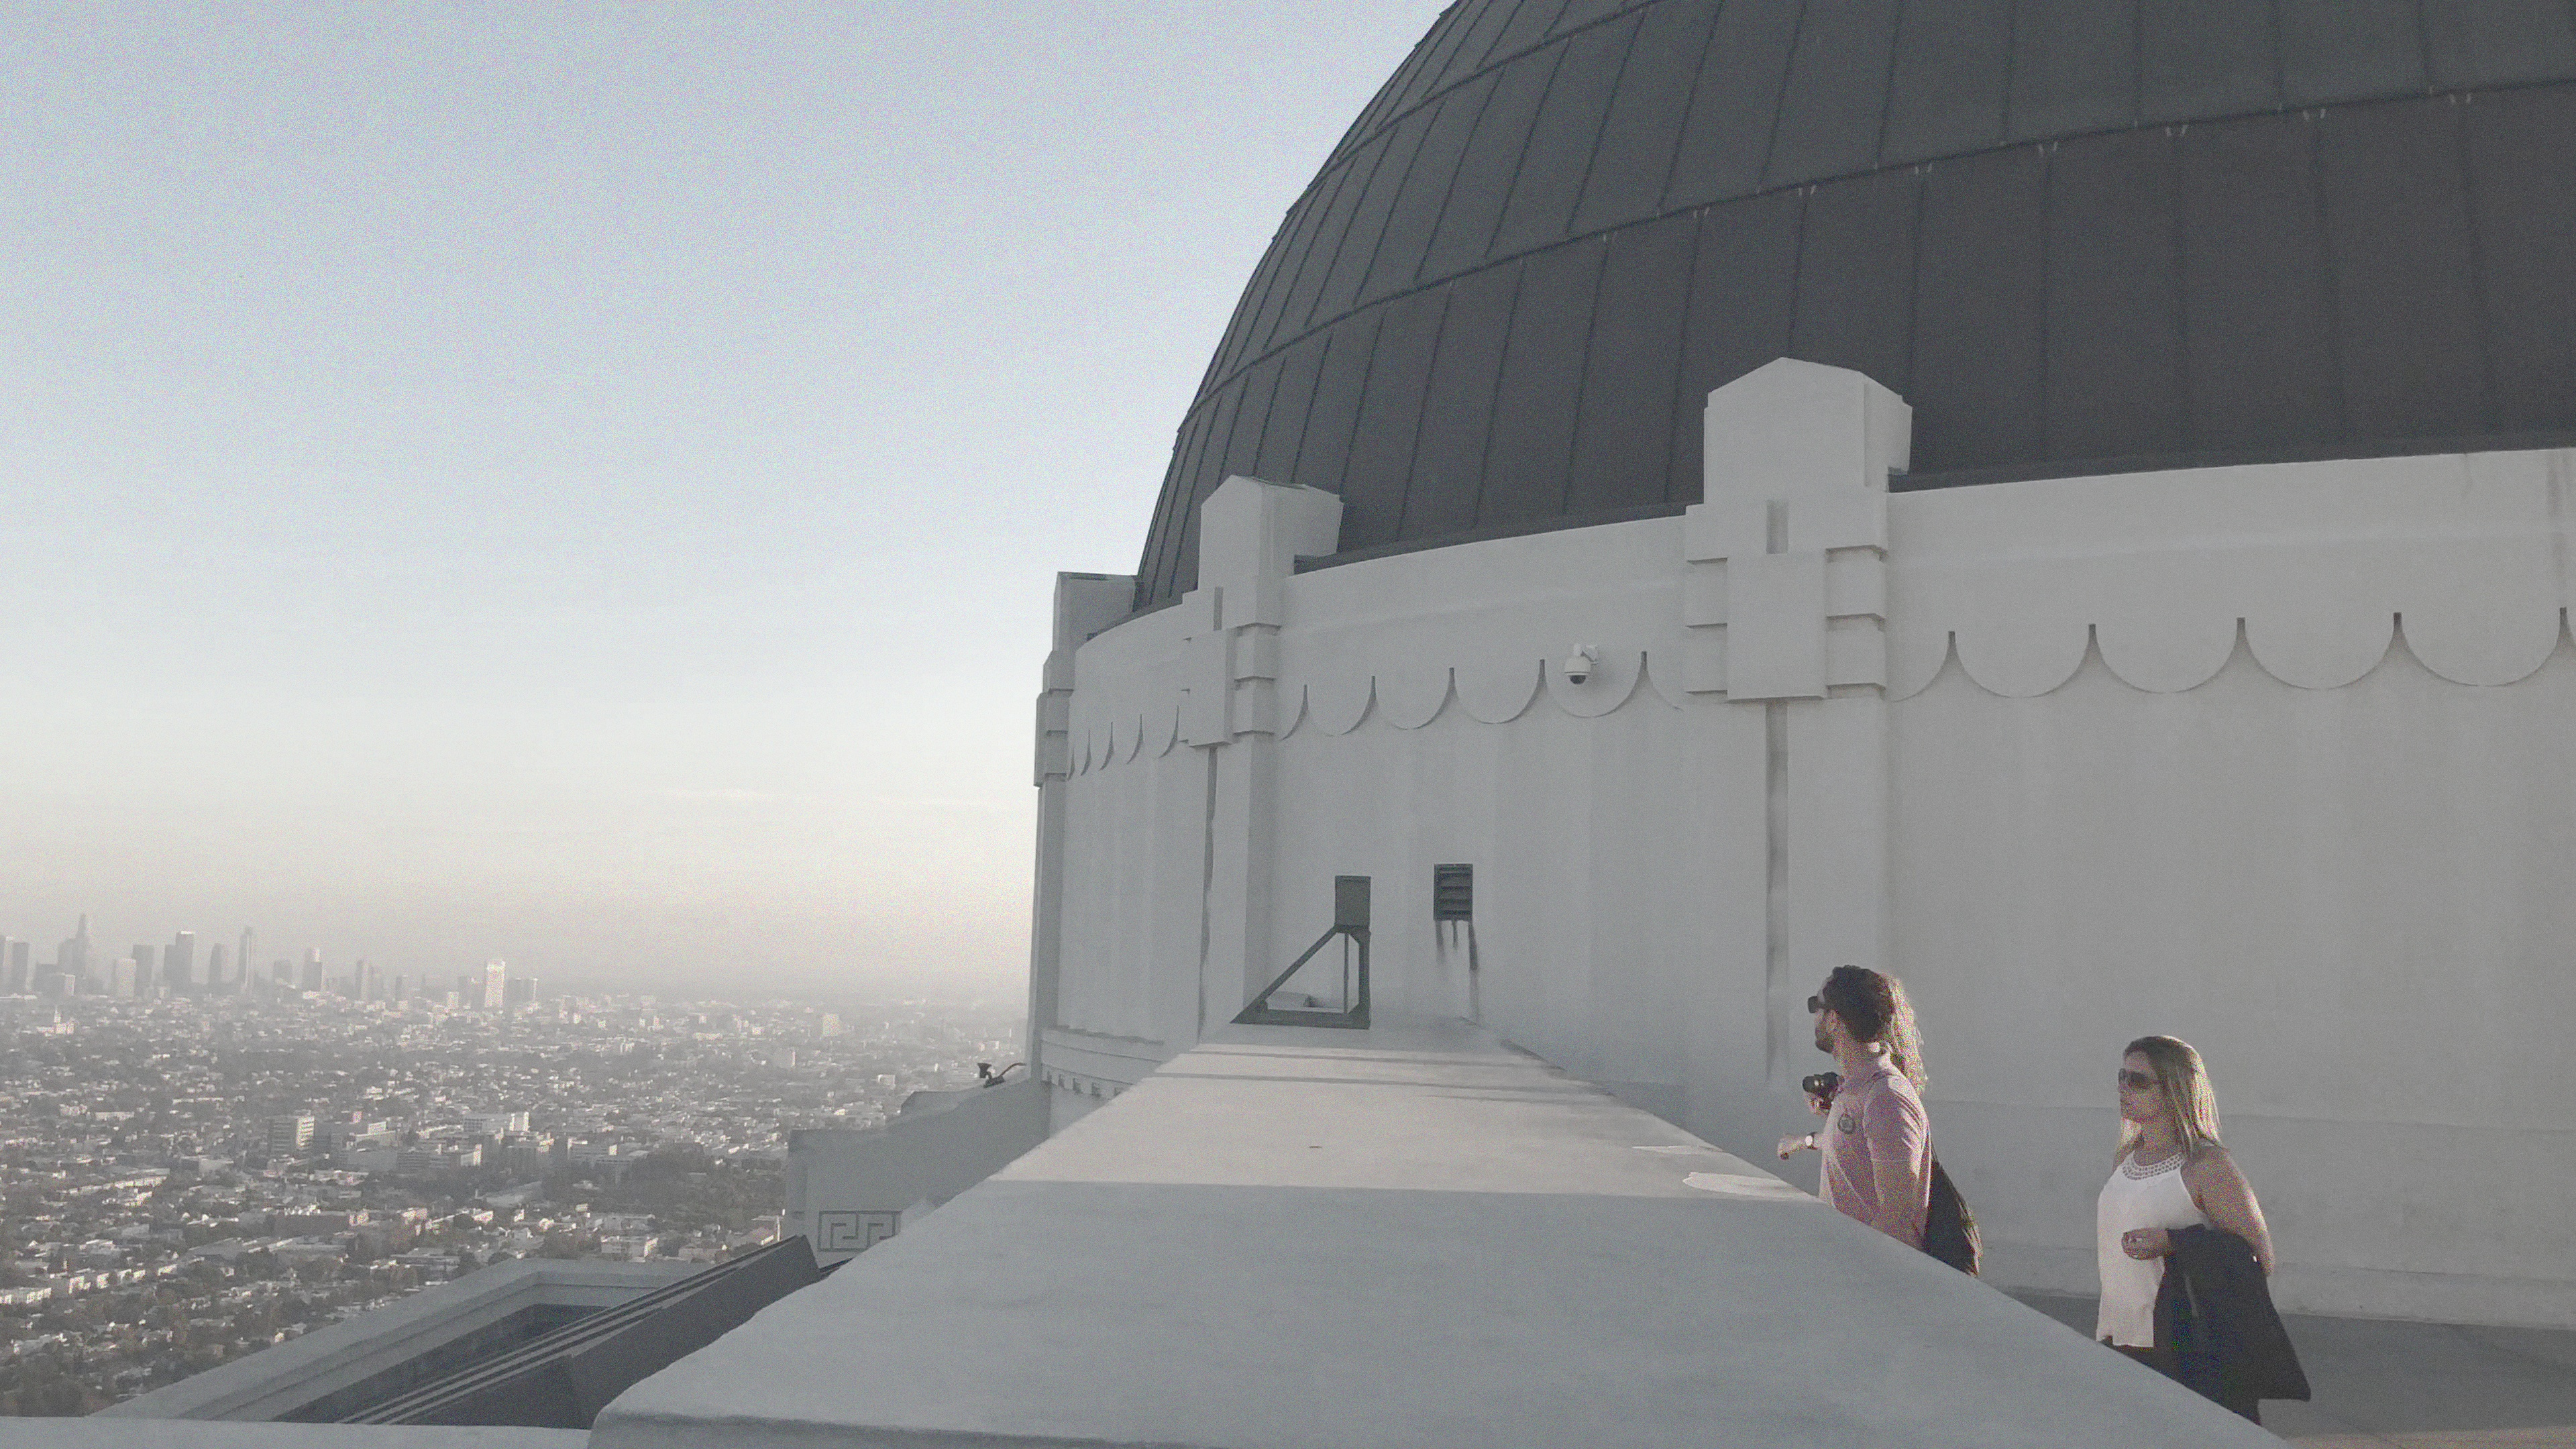}
        \caption{ISO Noise}
    \end{subfigure}
    \\    
    % Motion Blur
    \begin{subfigure}[b]{0.3\textwidth}
        \centering
        \includegraphics[width=\textwidth]{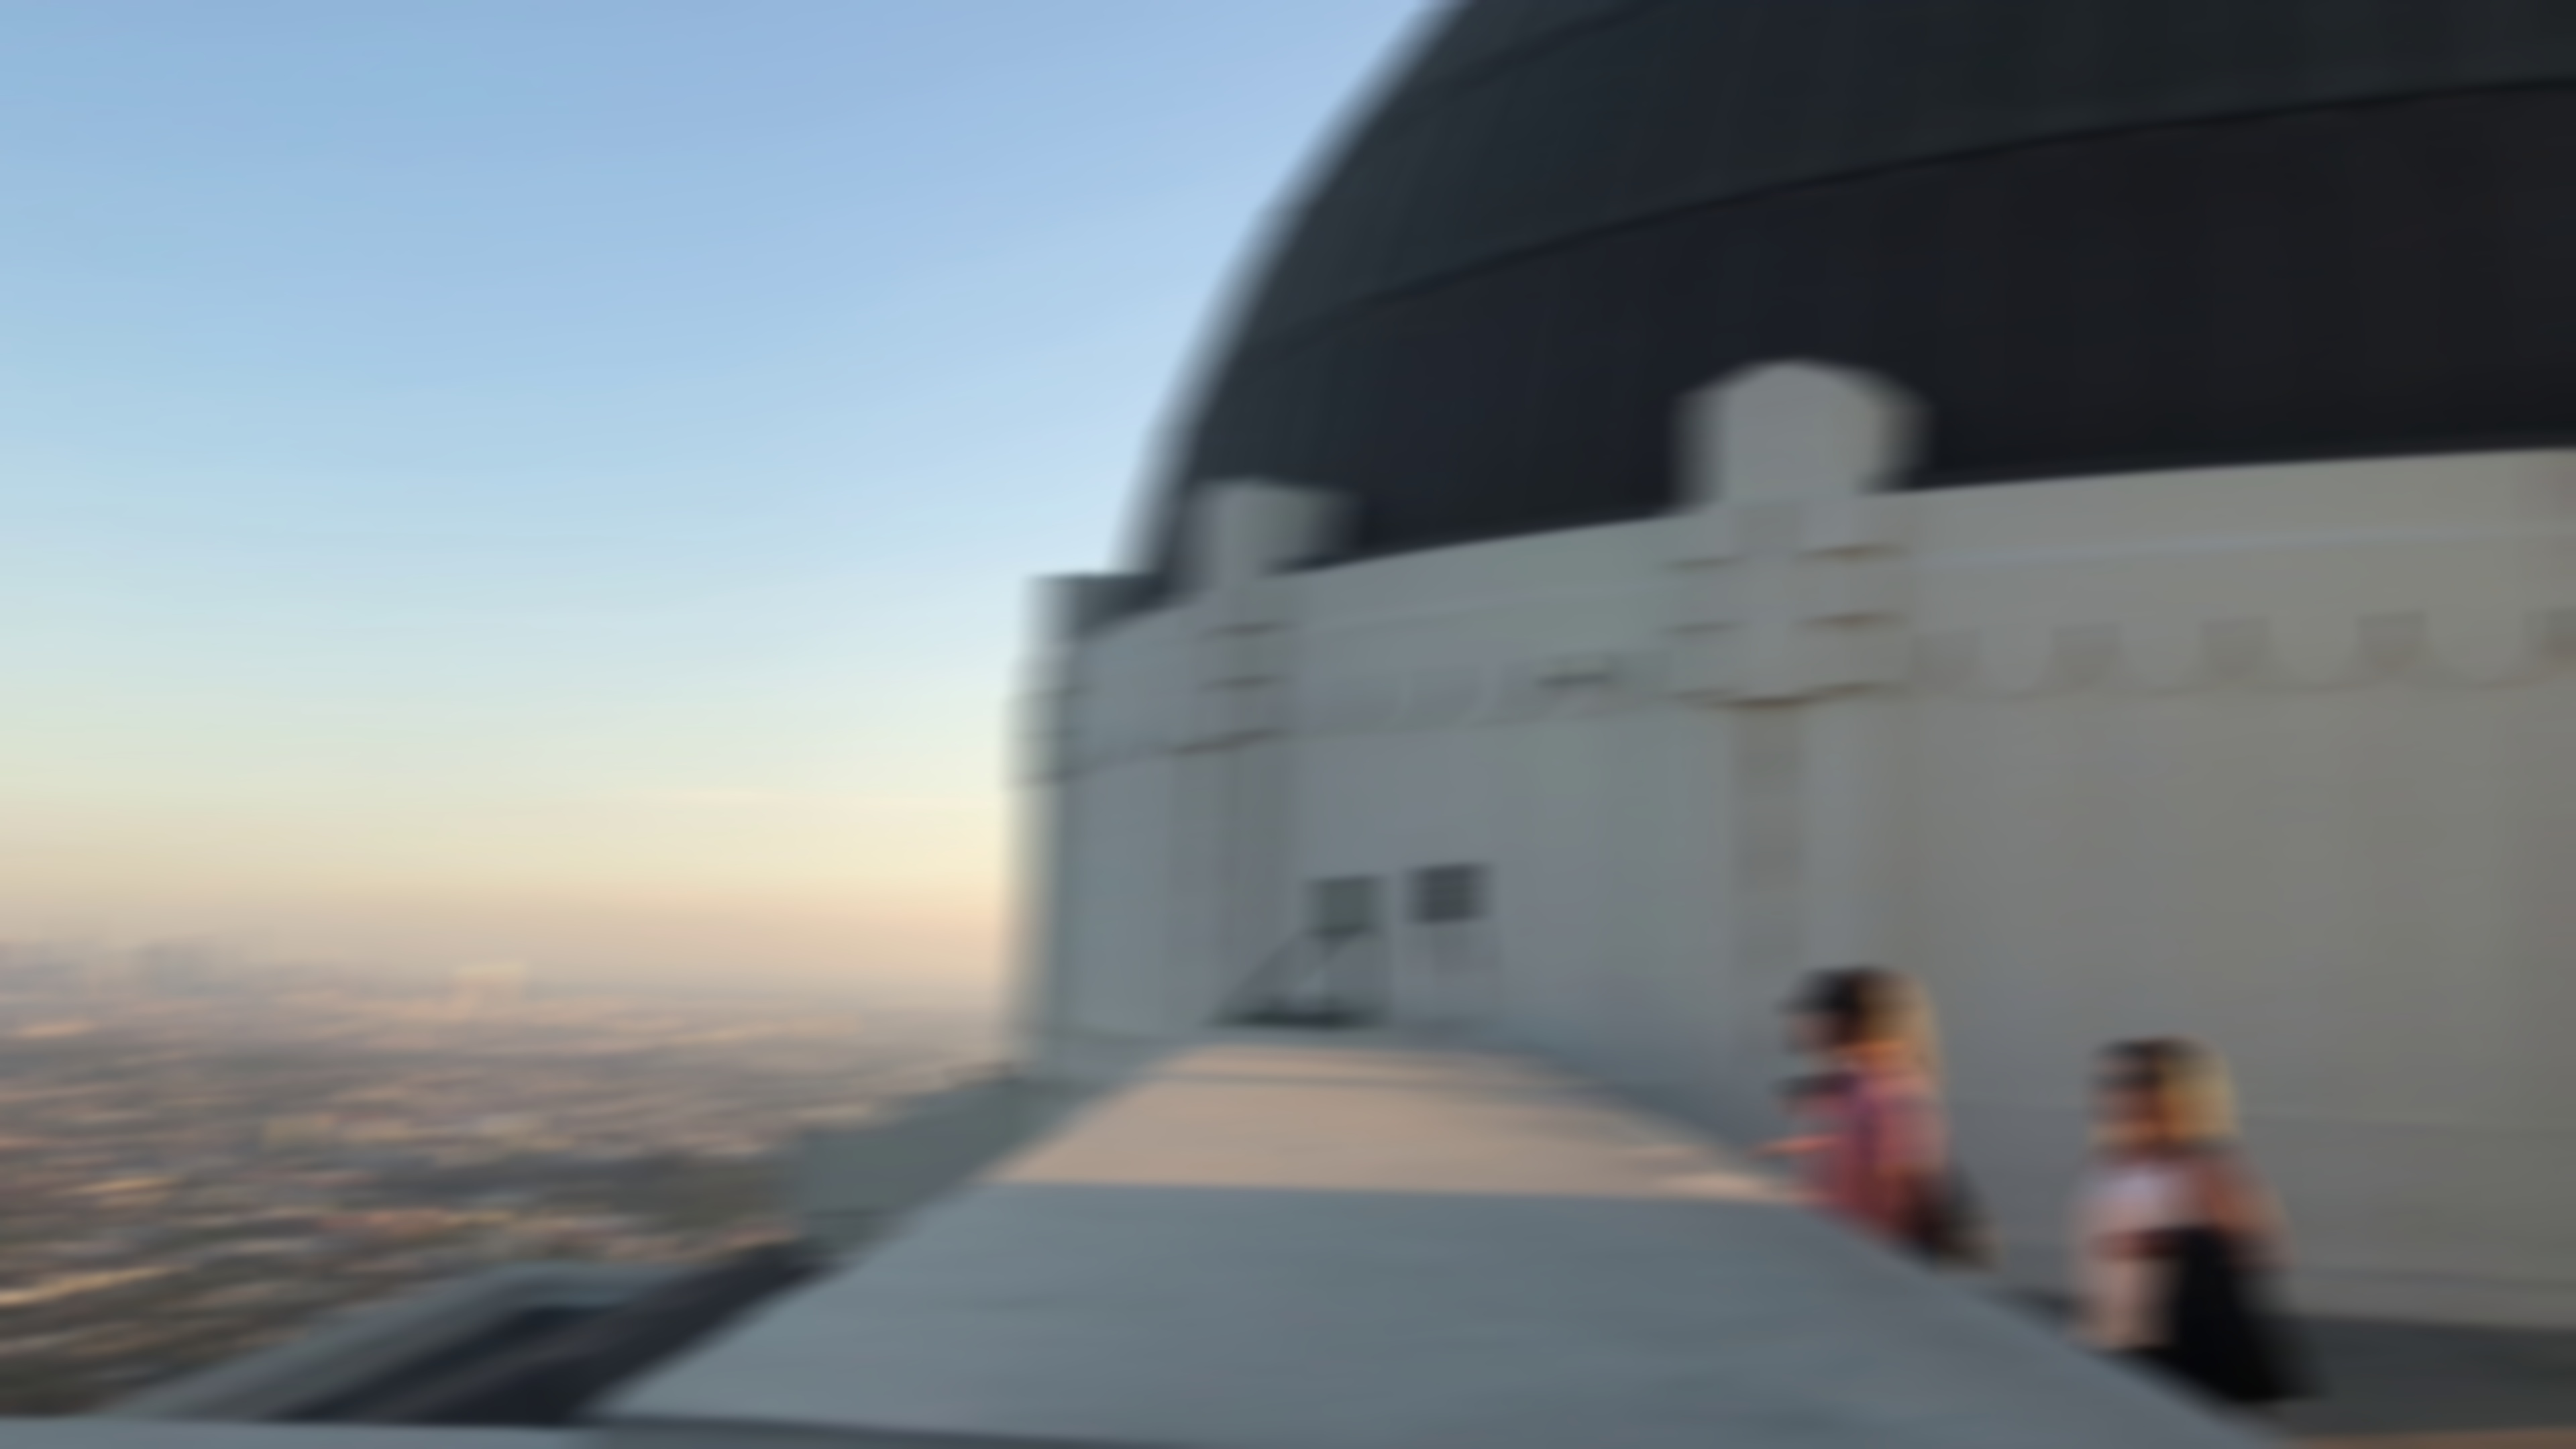}
        \caption{Motion Blur}
    \end{subfigure}
    % Compression
    \begin{subfigure}[b]{0.3\textwidth}
        \centering
        \includegraphics[width=\textwidth]{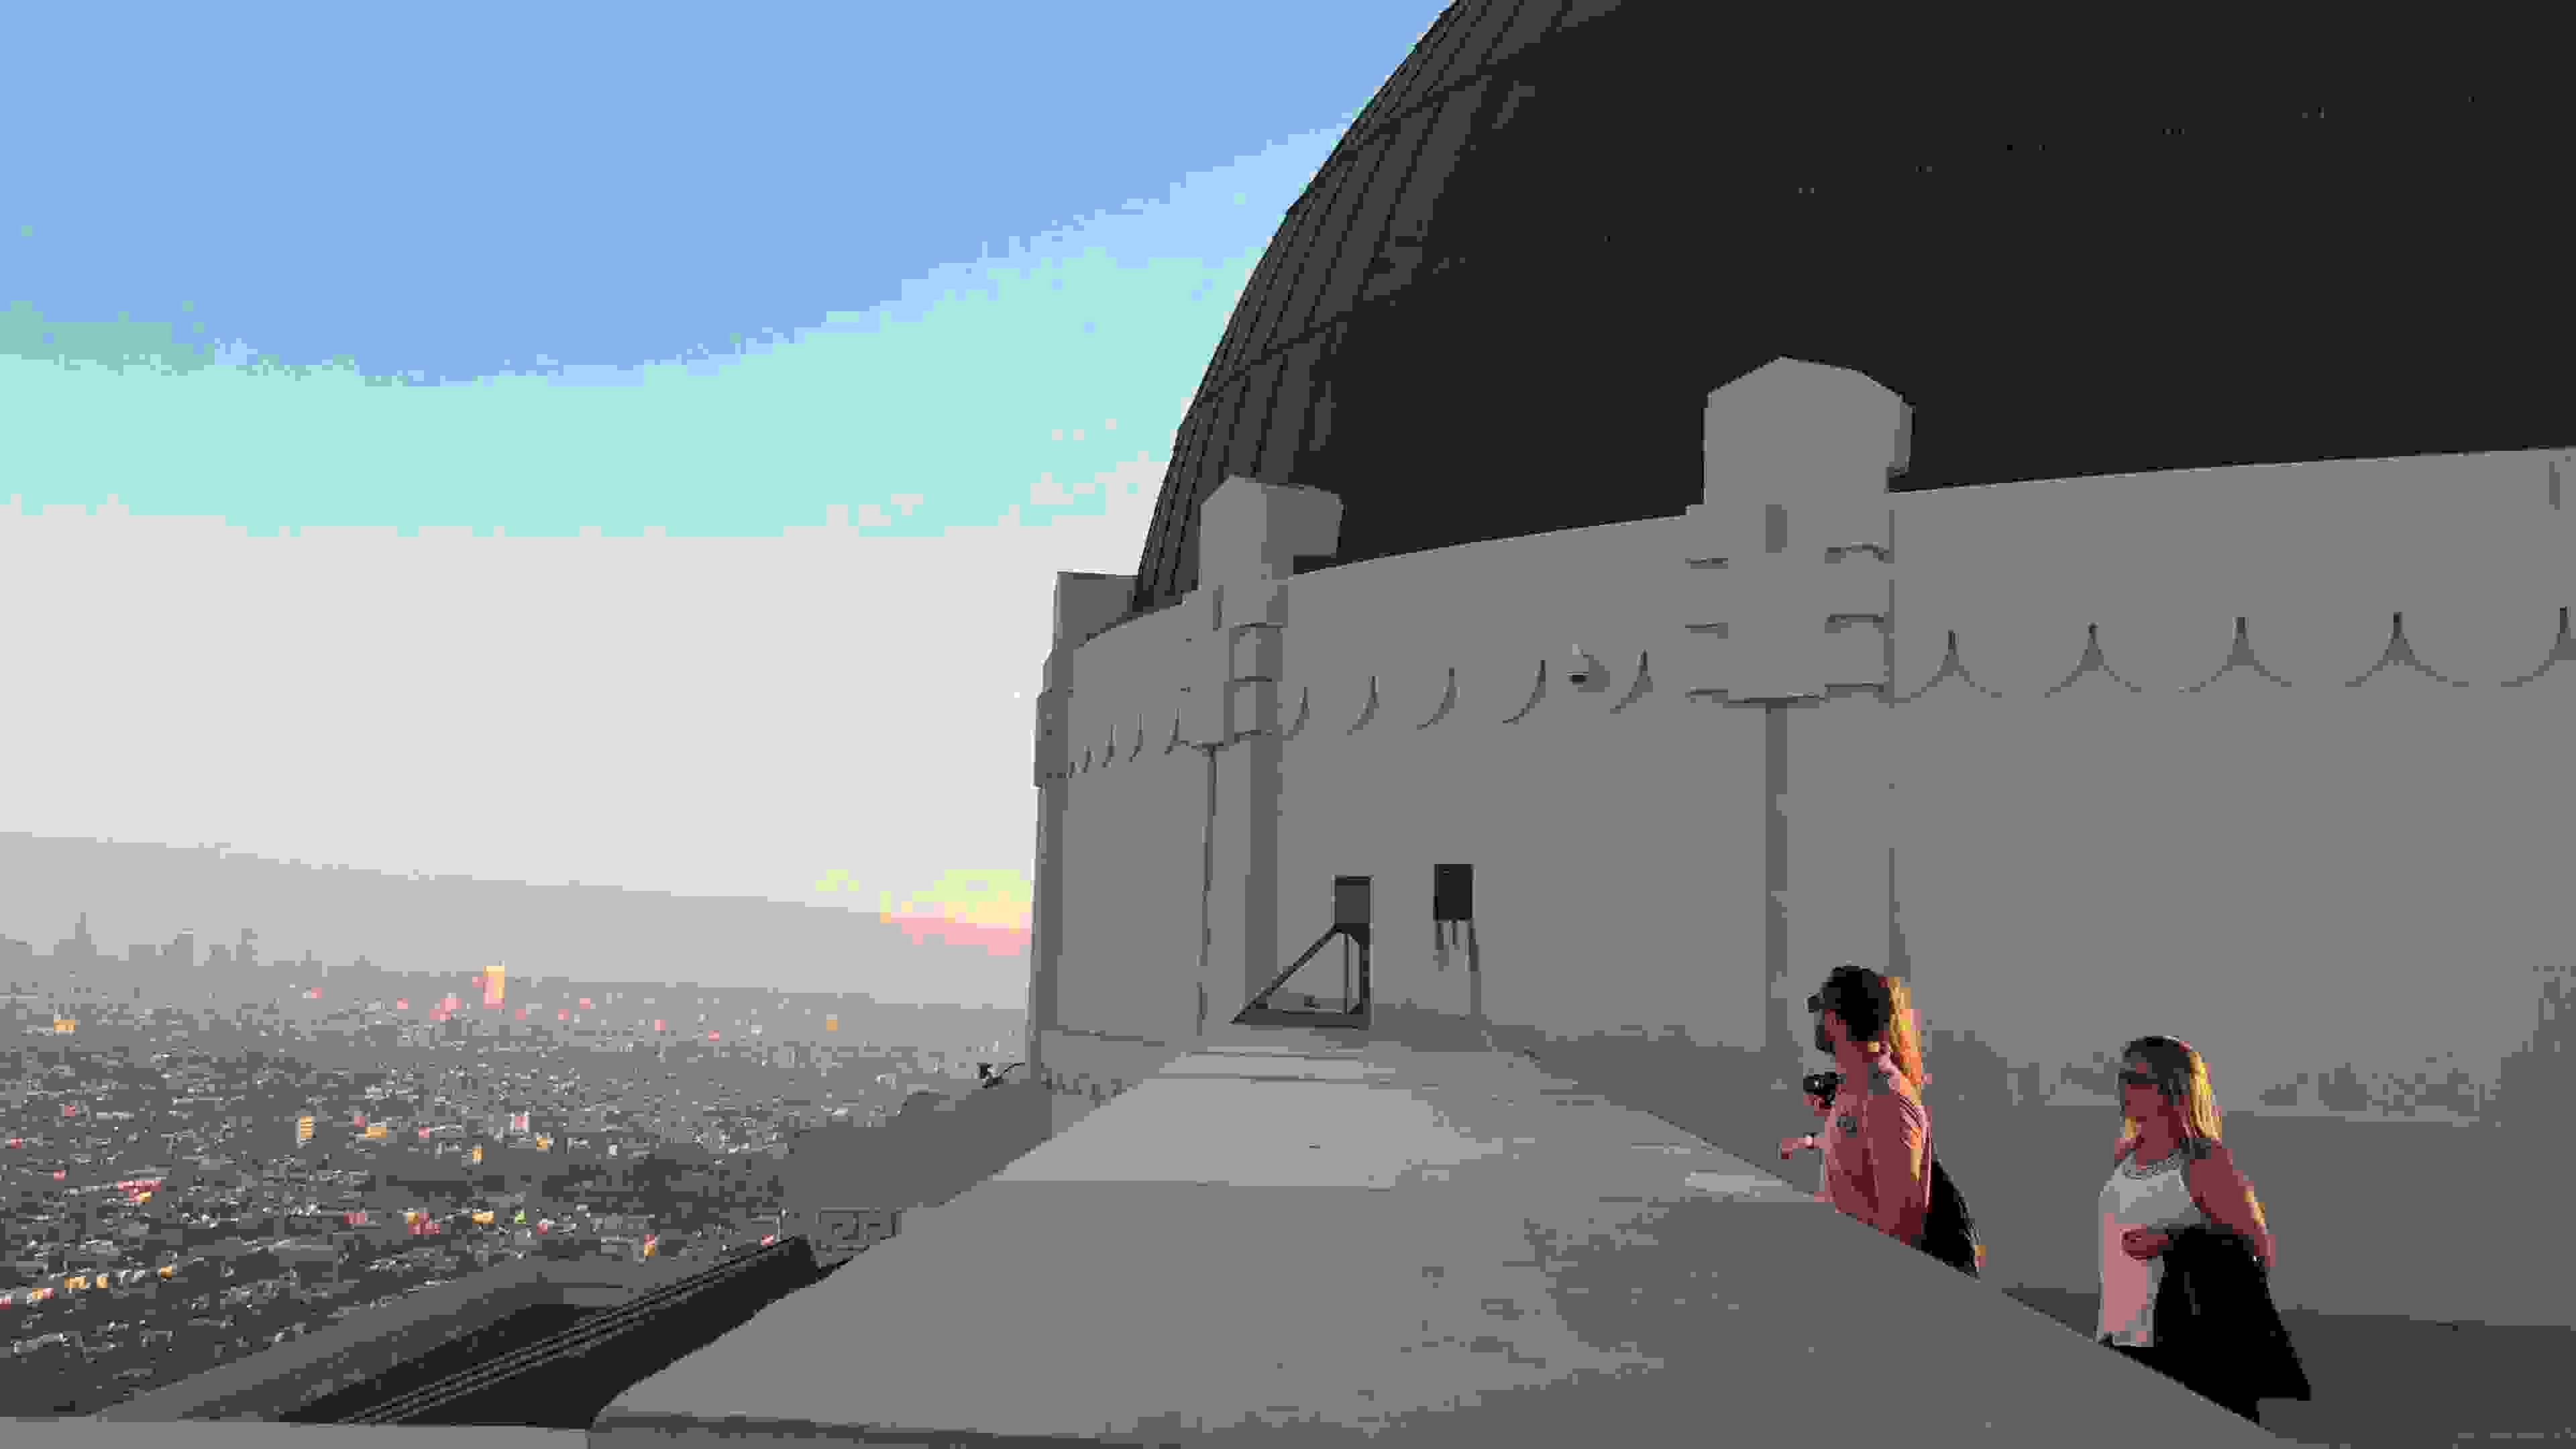}
        \caption{Compression}
    \end{subfigure}
    % Zoom Blur
    \begin{subfigure}[b]{0.3\textwidth}
        \centering
        \includegraphics[width=\textwidth]{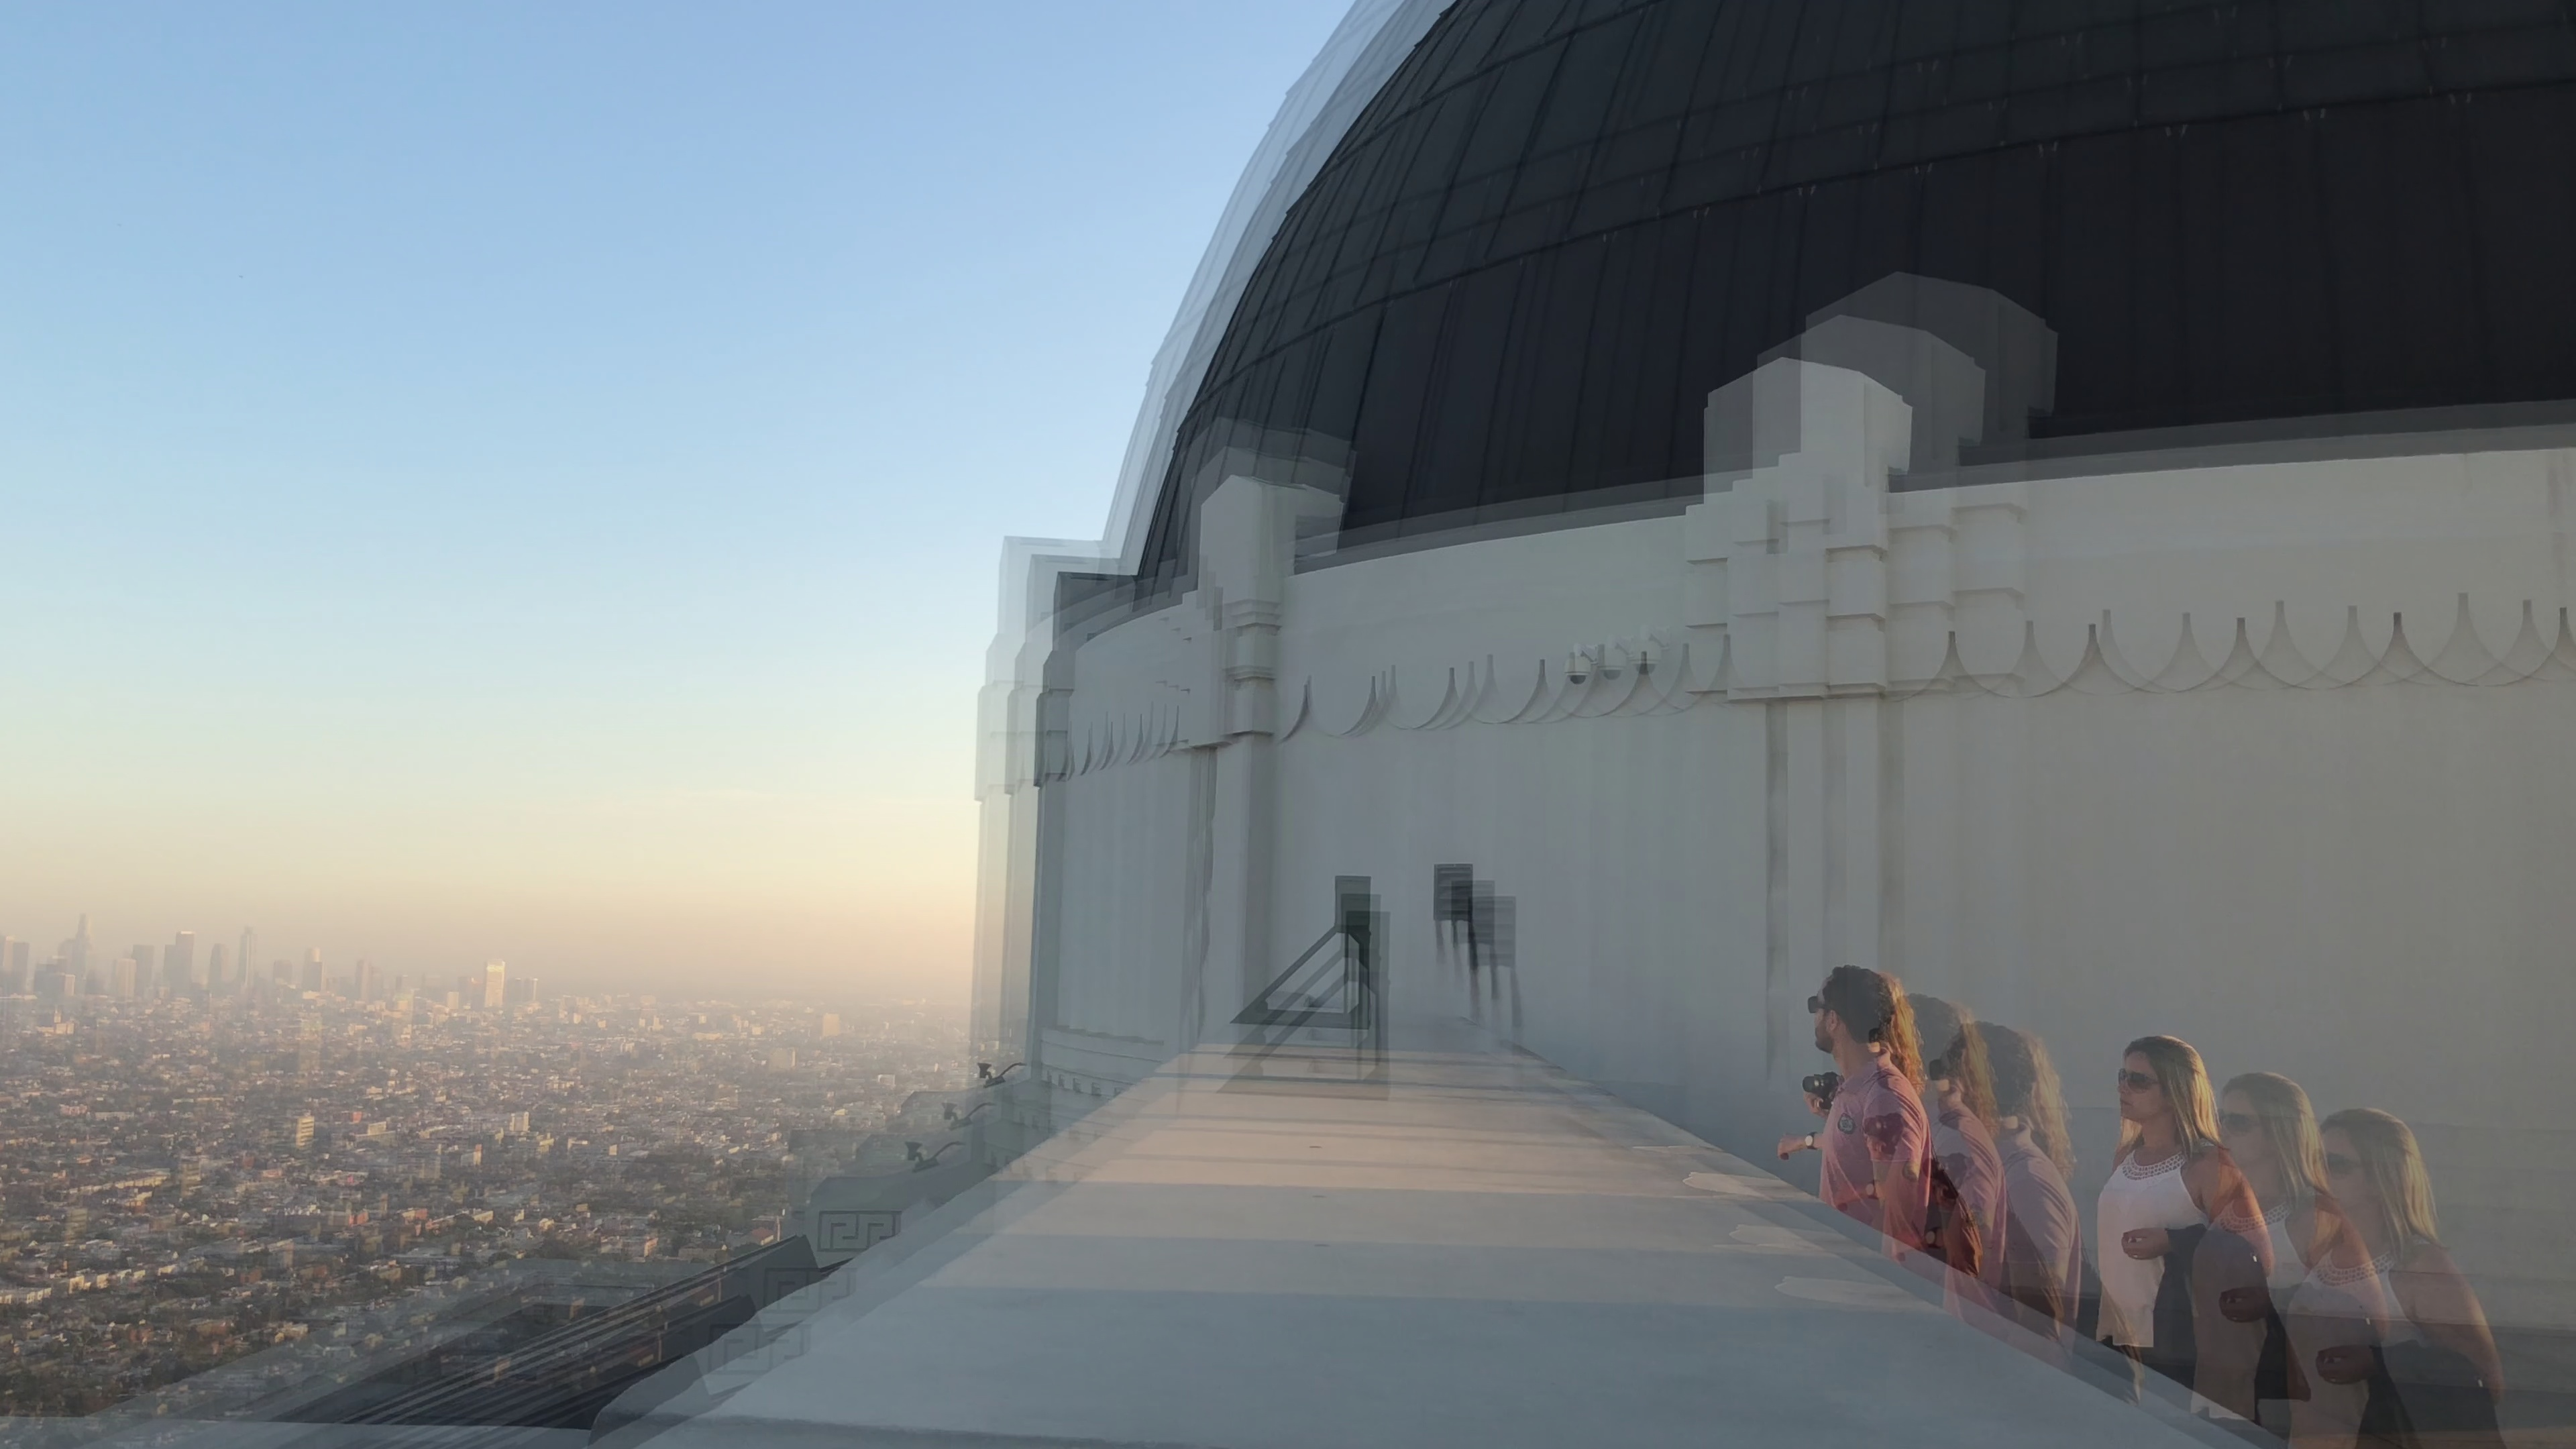}
        \caption{Zoom Blur}
    \end{subfigure}

    \caption{\textbf{Examples of video frames with different distortion types.}}
    \label{fig:distortion_examples}
\end{figure*}

\begin{figure*}[t]
    \centering
    % Video 1
    \begin{subfigure}[b]{0.3\textwidth}
        \centering
        \includegraphics[width=\textwidth]{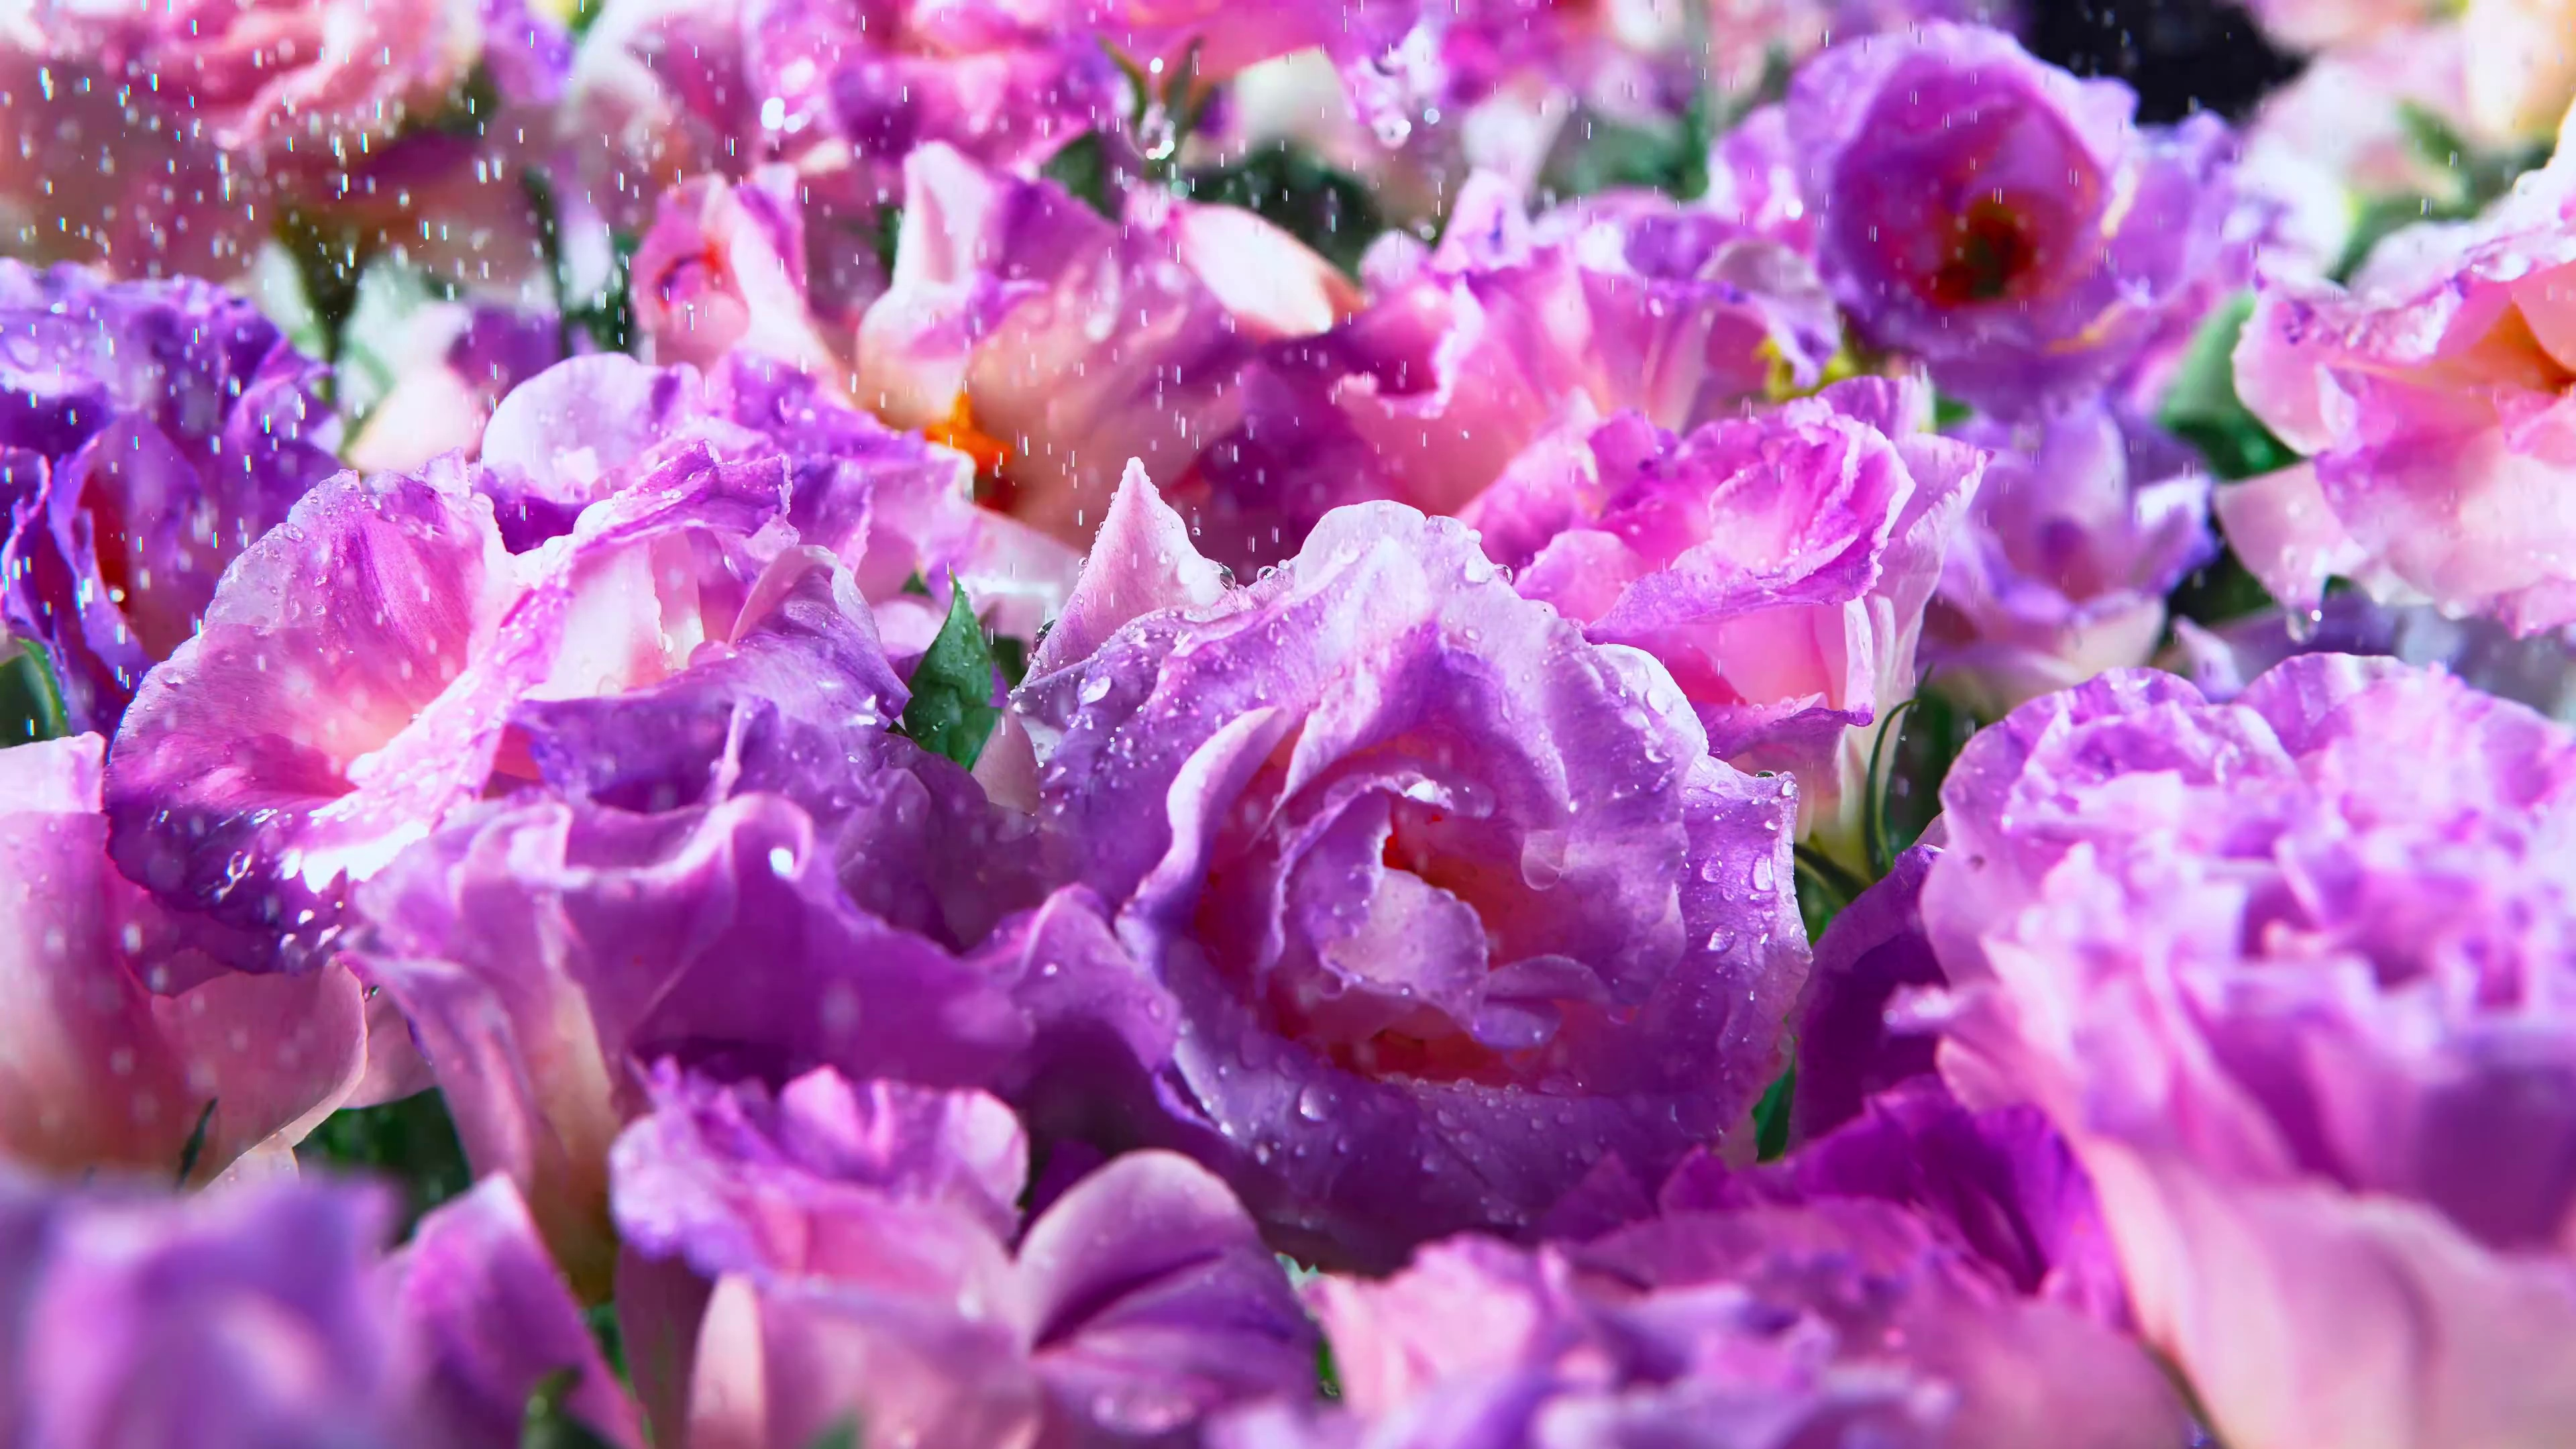}
        \caption{Video 1}
    \end{subfigure}
    % Video 2
    \begin{subfigure}[b]{0.3\textwidth}
        \centering
        \includegraphics[width=\textwidth]{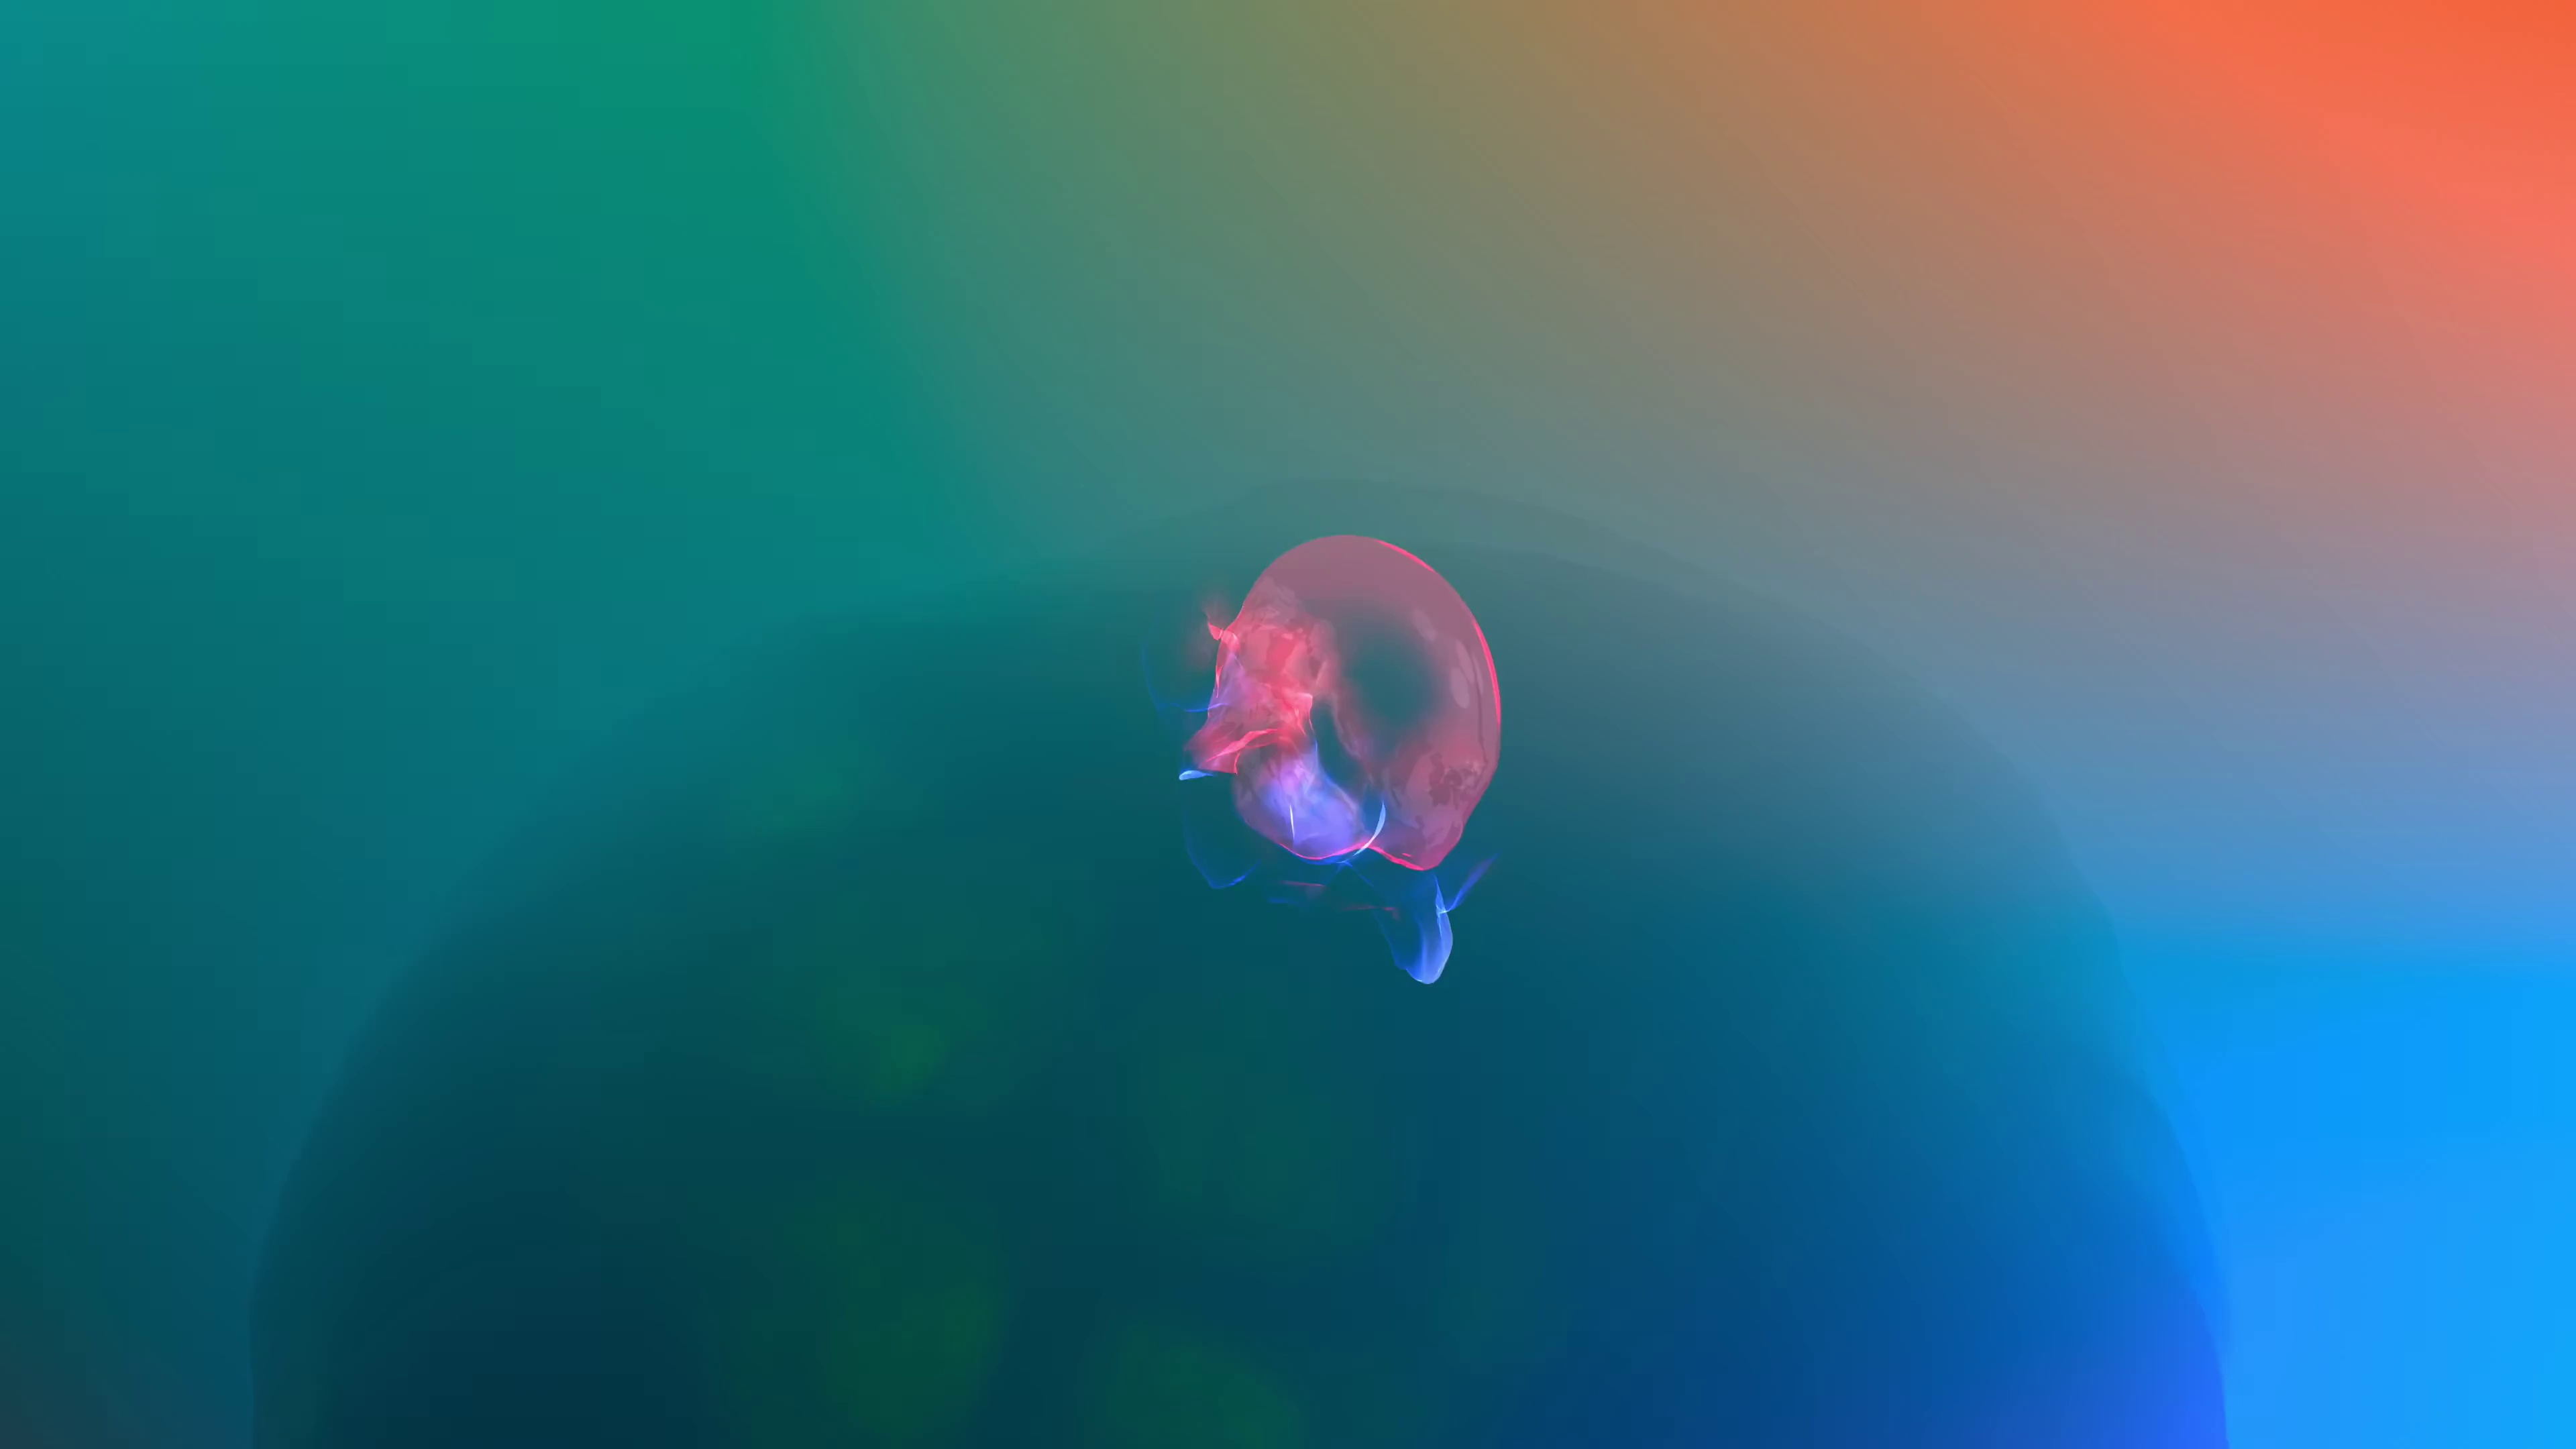}
        \caption{Video 2}
    \end{subfigure}
    % Video 3
    \begin{subfigure}[b]{0.3\textwidth}
        \centering
        \includegraphics[width=\textwidth]{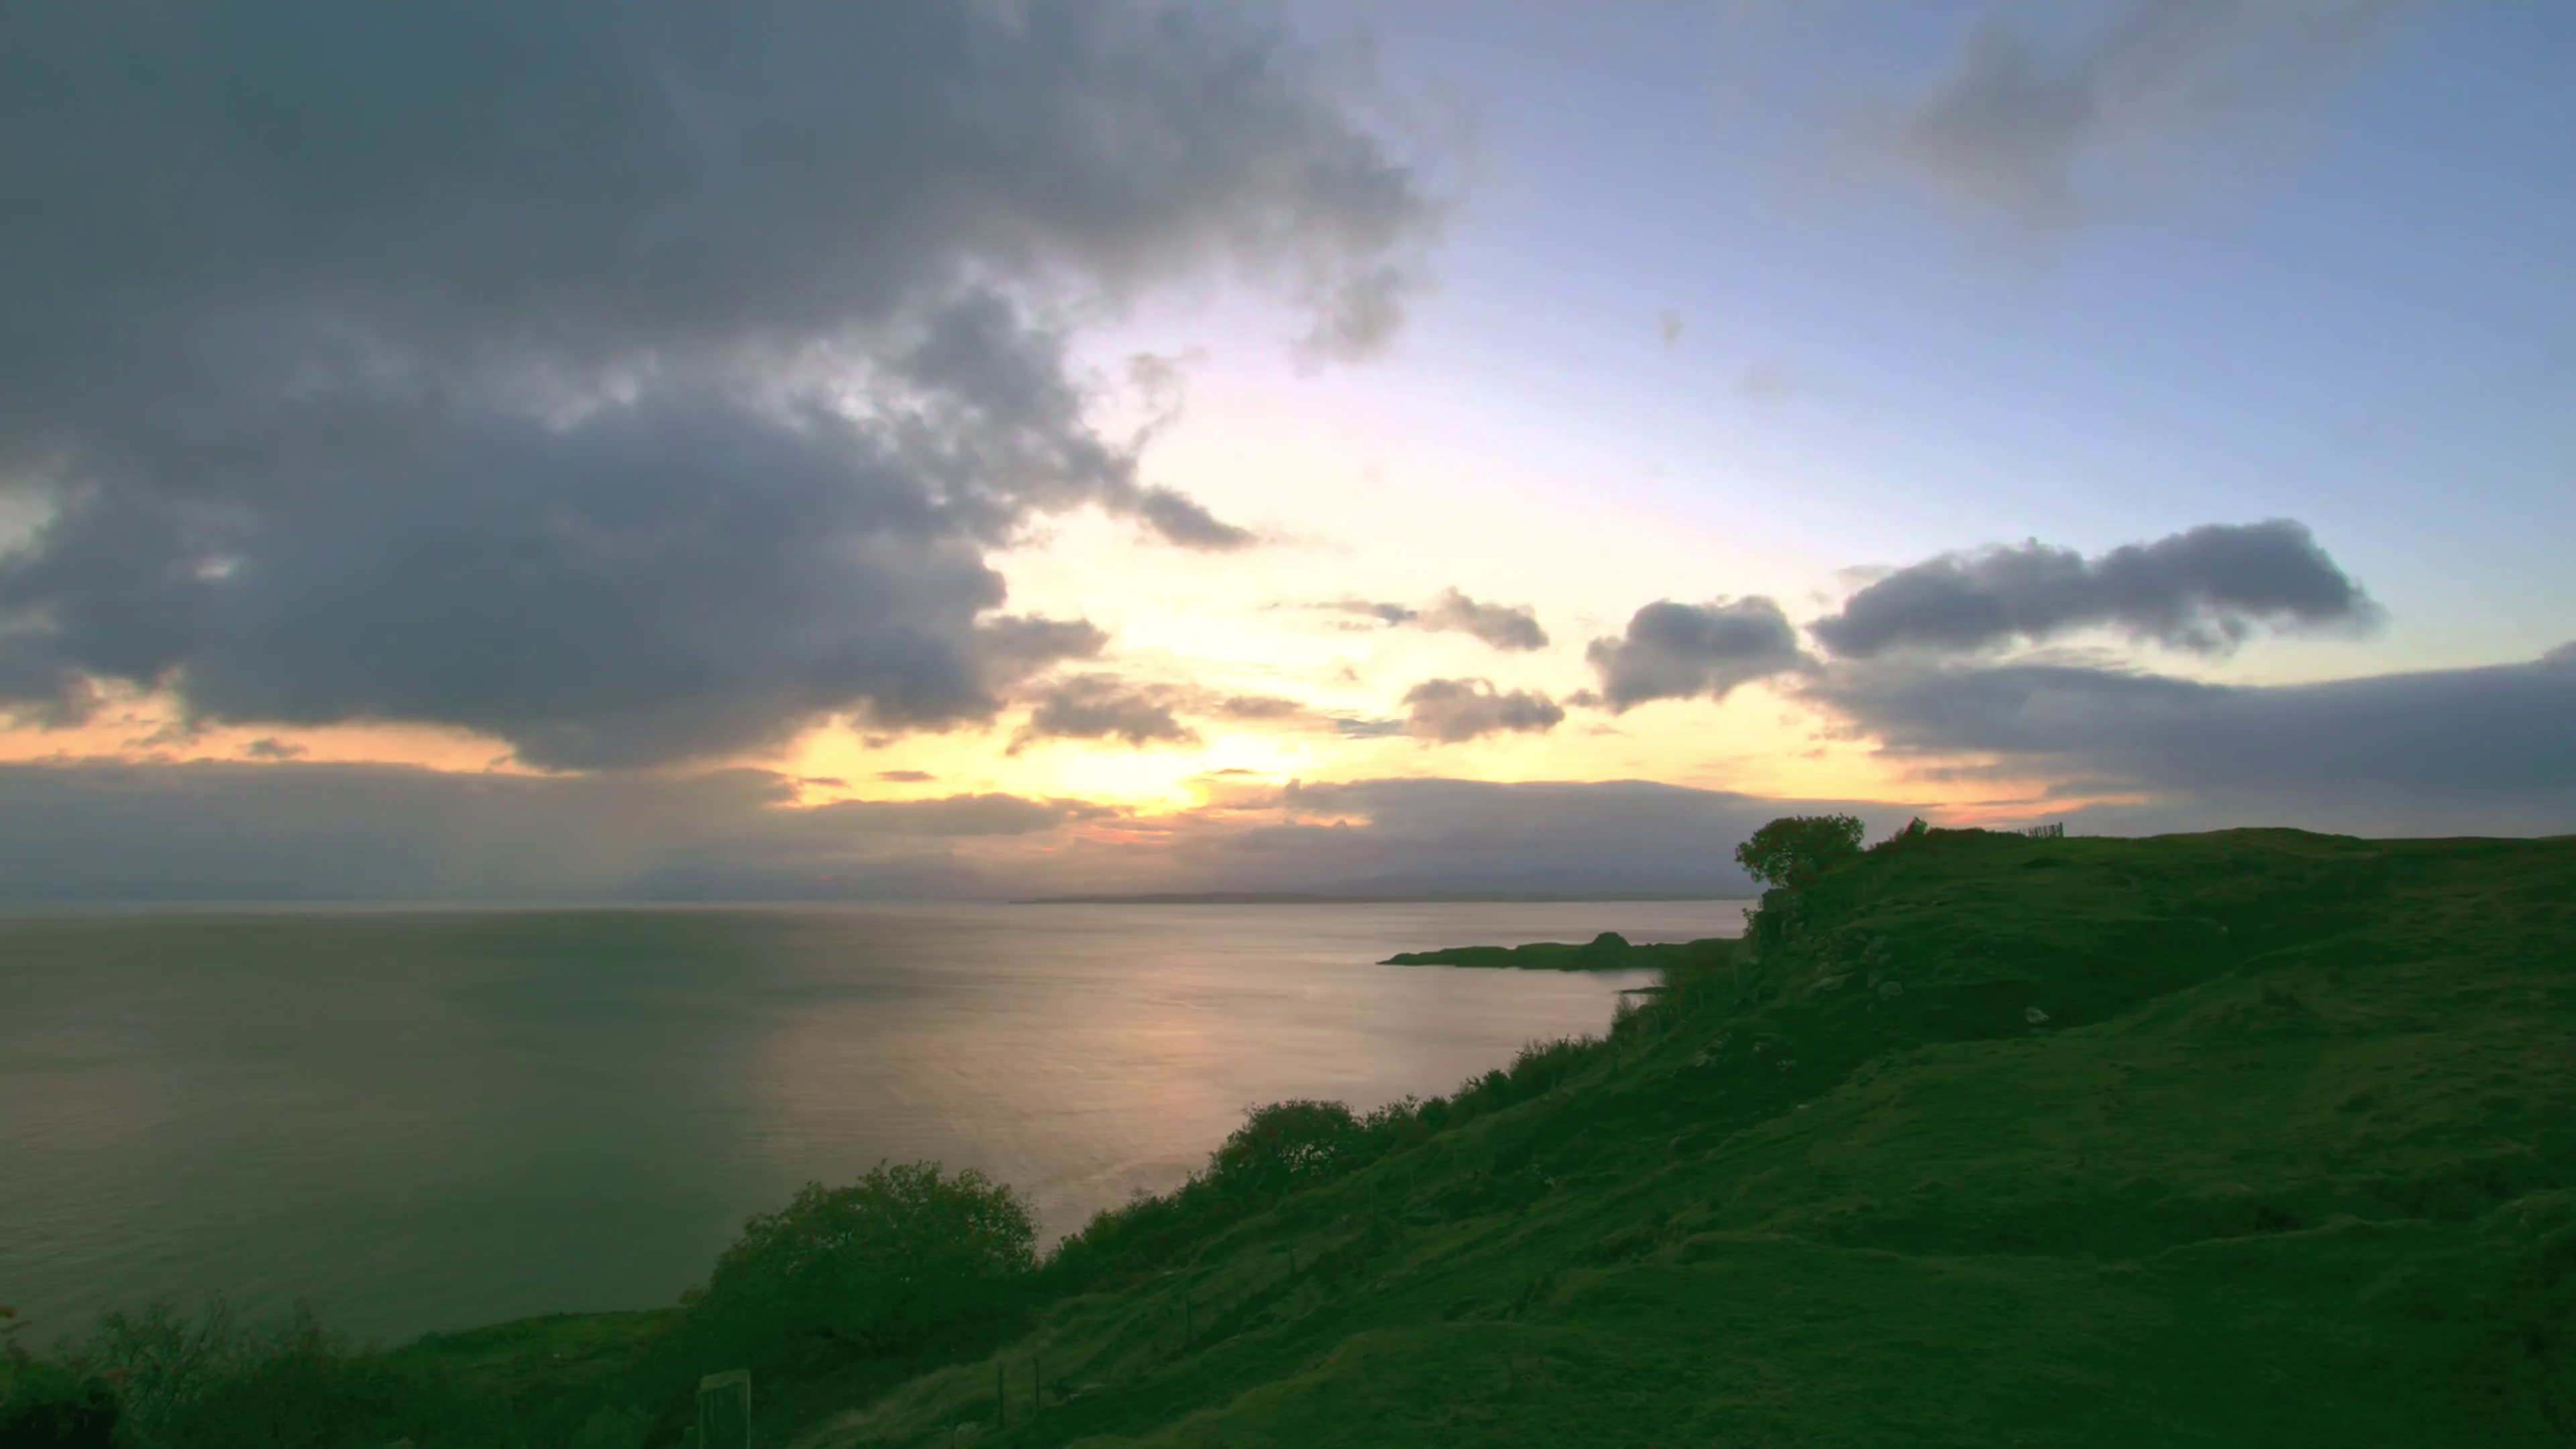}
        \caption{Video 3}
    \end{subfigure}
    
    \vspace{0.5cm}
    
    % Video 4
    \begin{subfigure}[b]{0.3\textwidth}
        \centering
        \includegraphics[width=\textwidth]{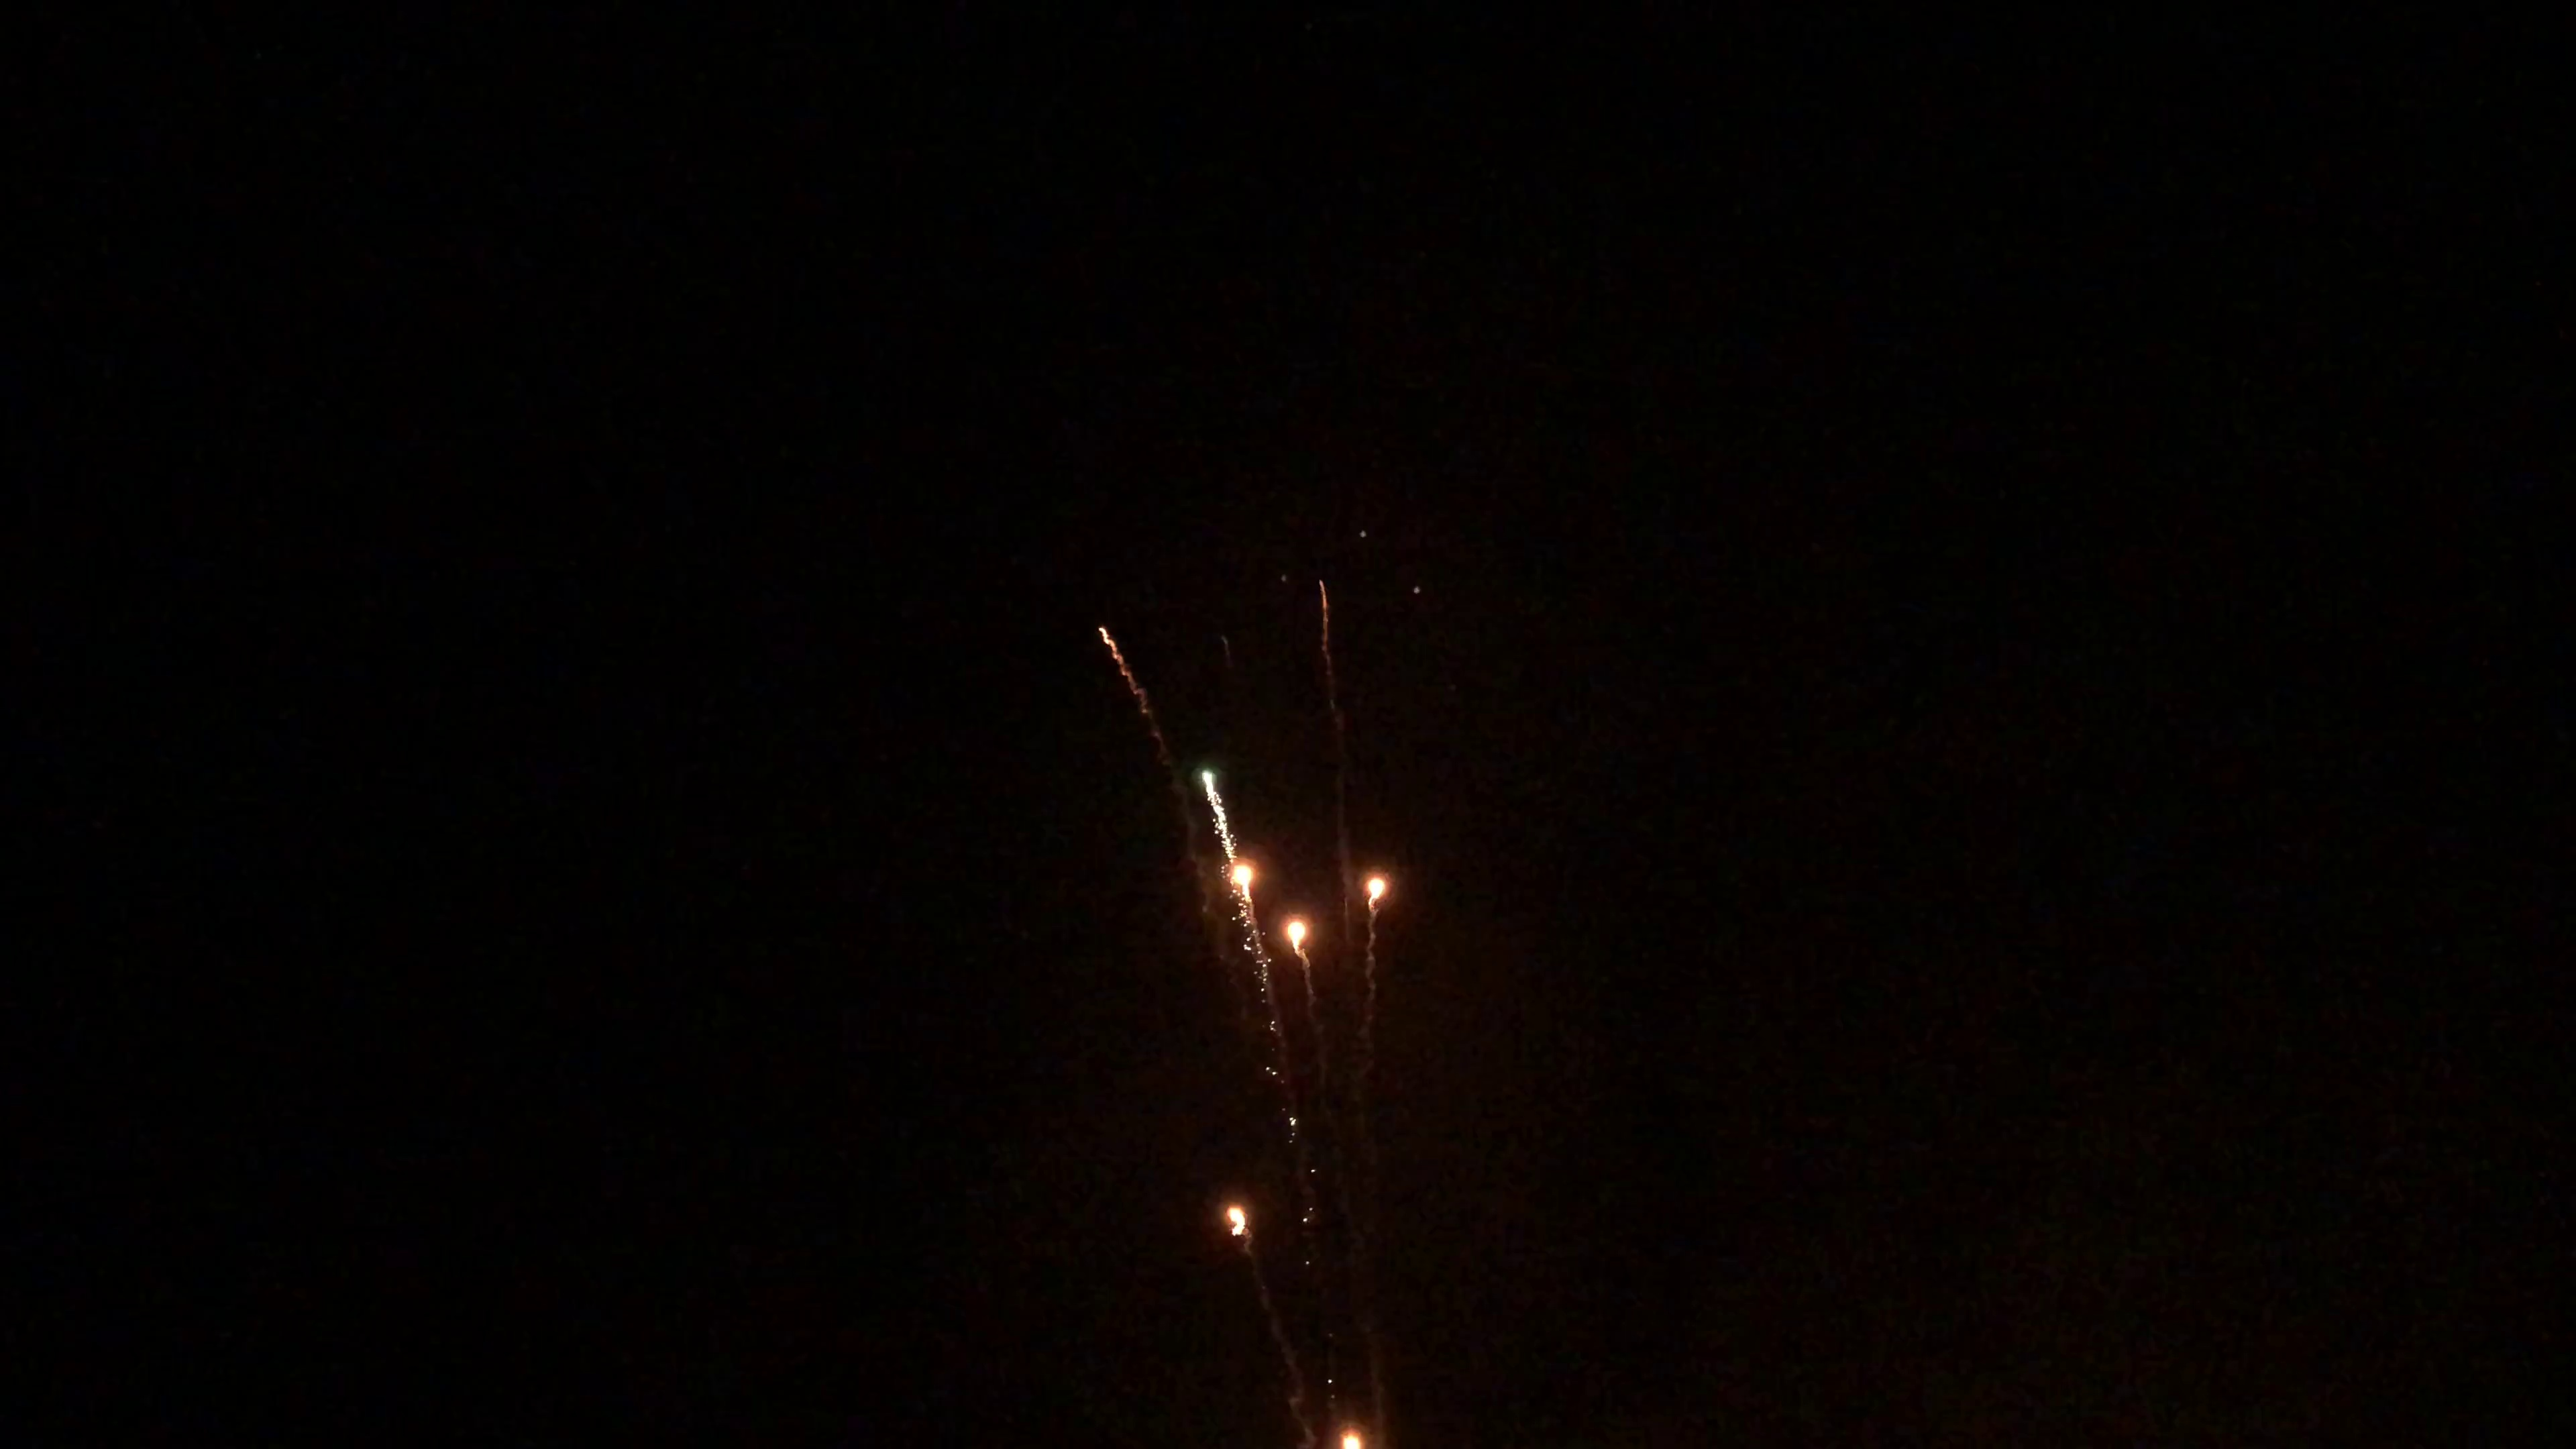}
        \caption{Video 4}
    \end{subfigure}
    % Video 5
    \begin{subfigure}[b]{0.3\textwidth}
        \centering
        \includegraphics[width=\textwidth]{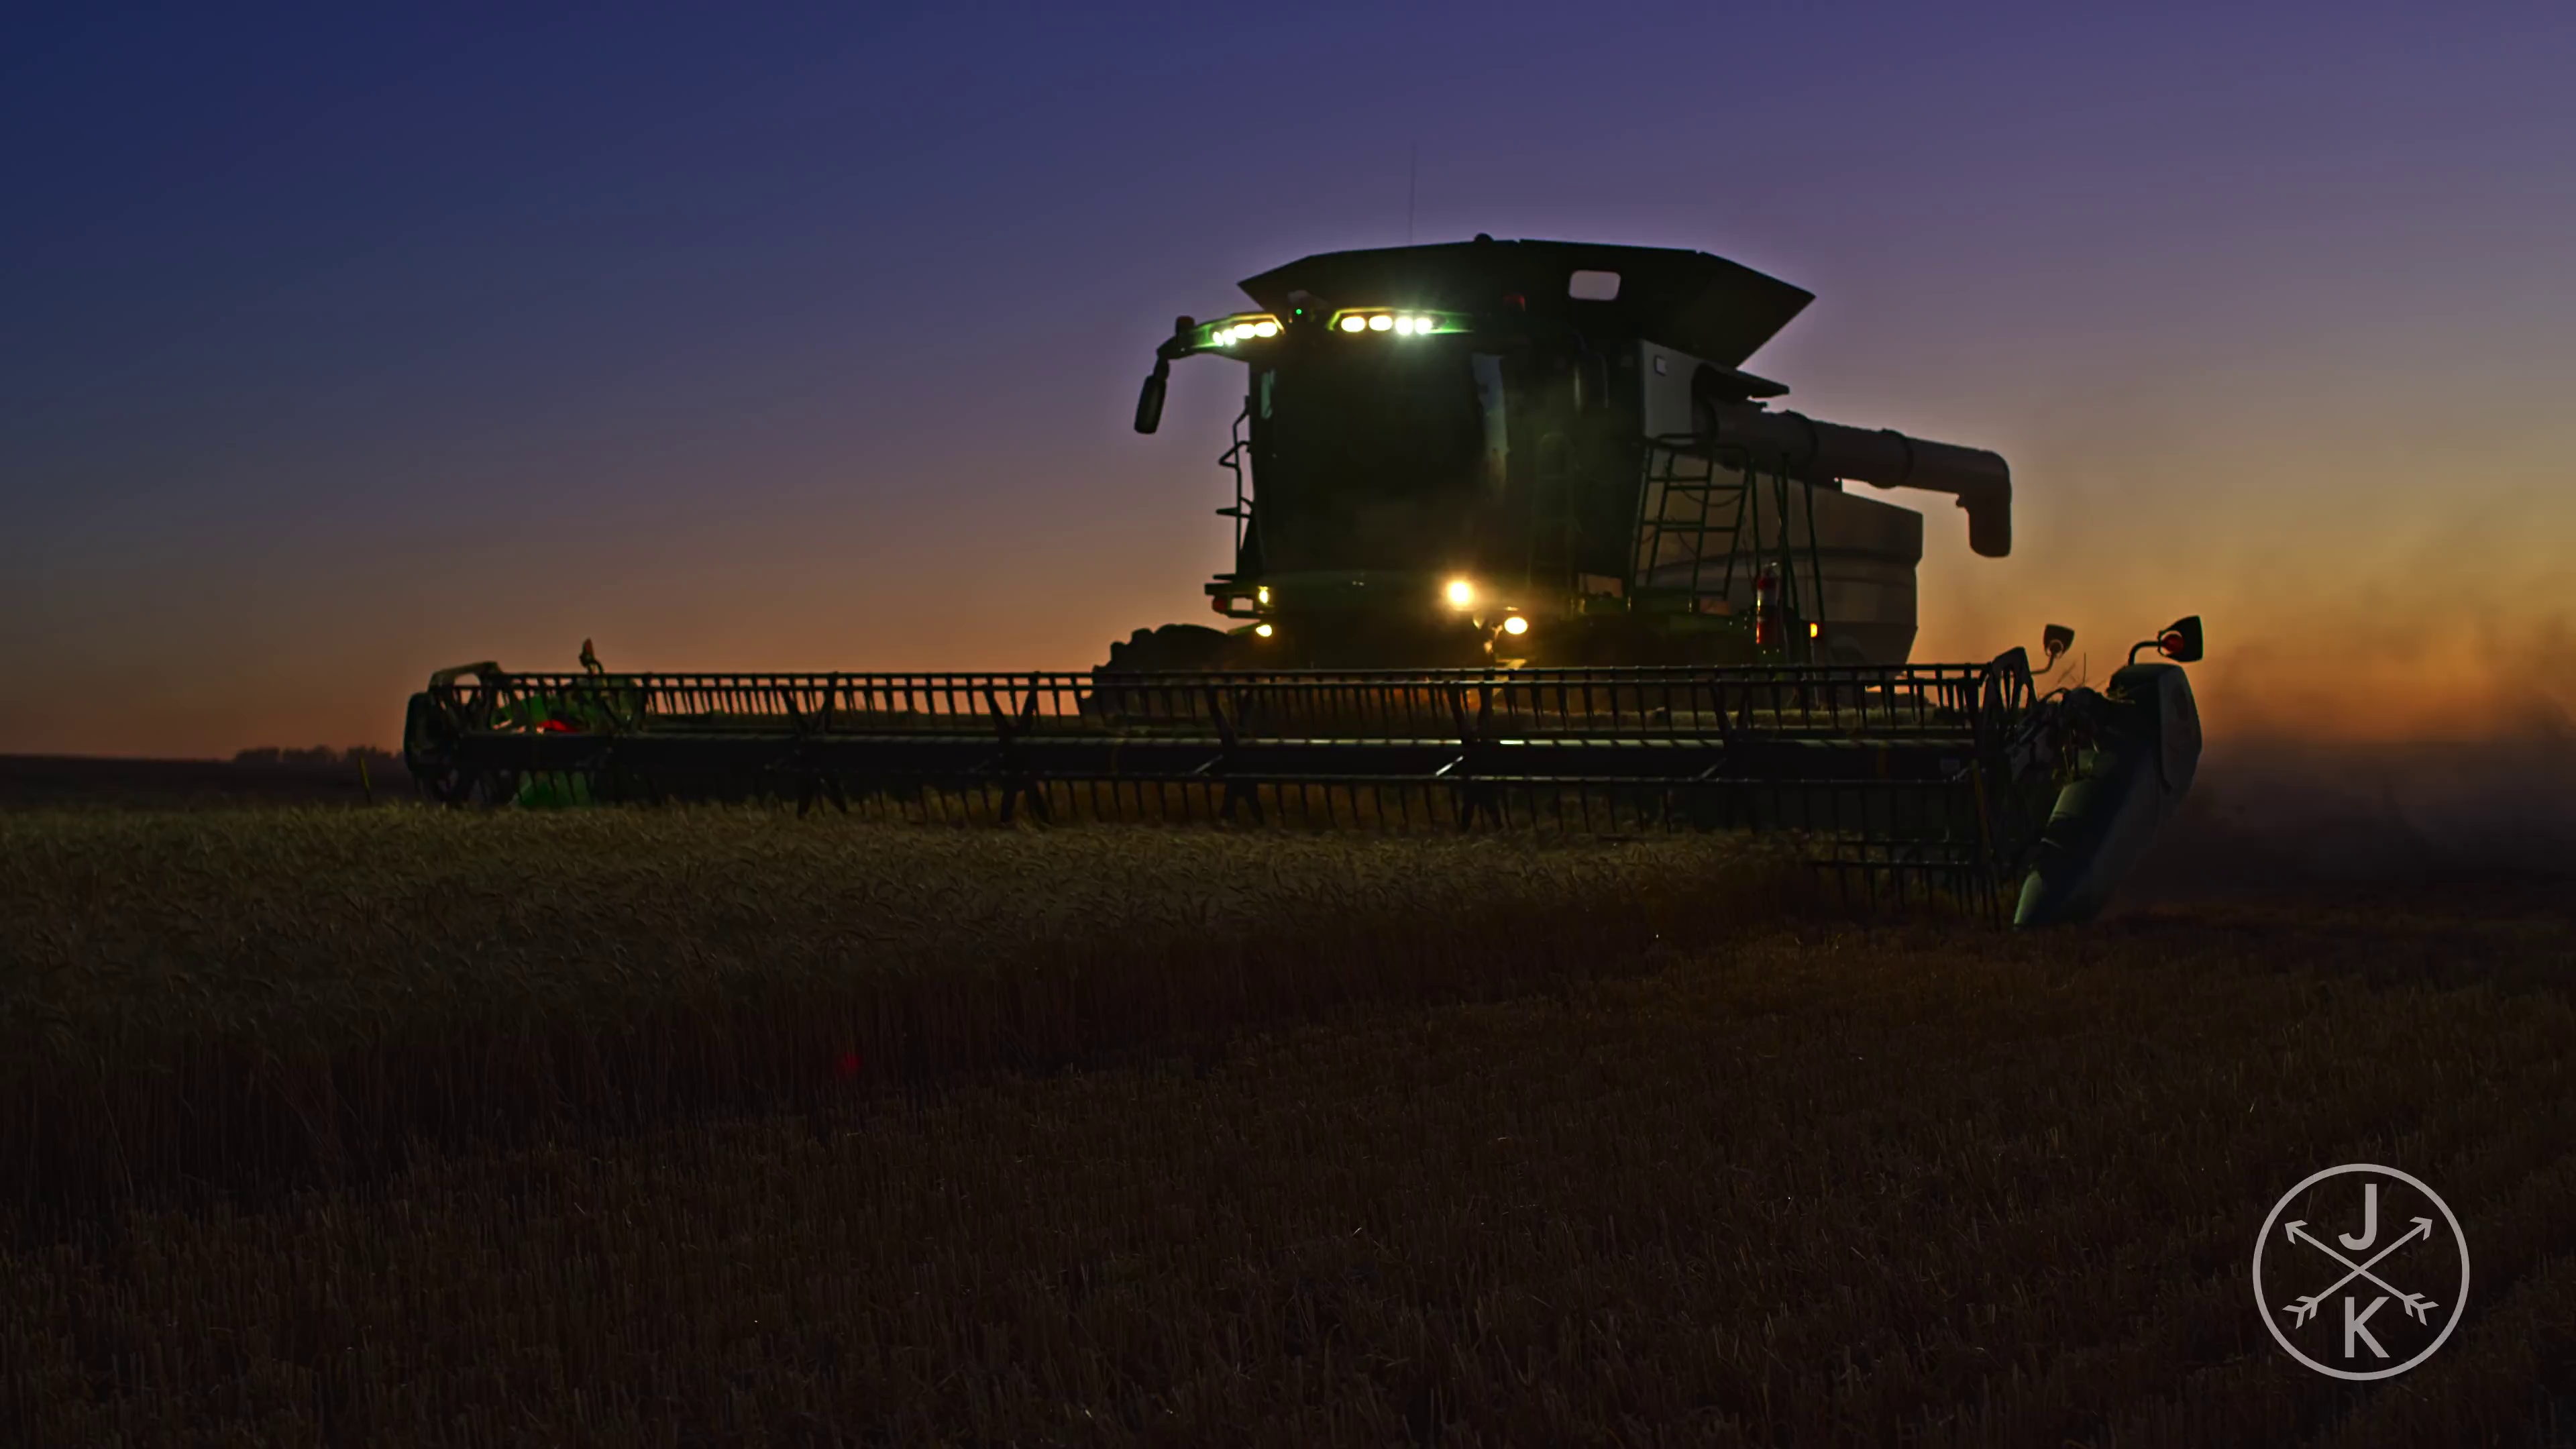}
        \caption{Video 5}
    \end{subfigure}
    % Video 6
    \begin{subfigure}[b]{0.3\textwidth}
        \centering
        \includegraphics[width=\textwidth]{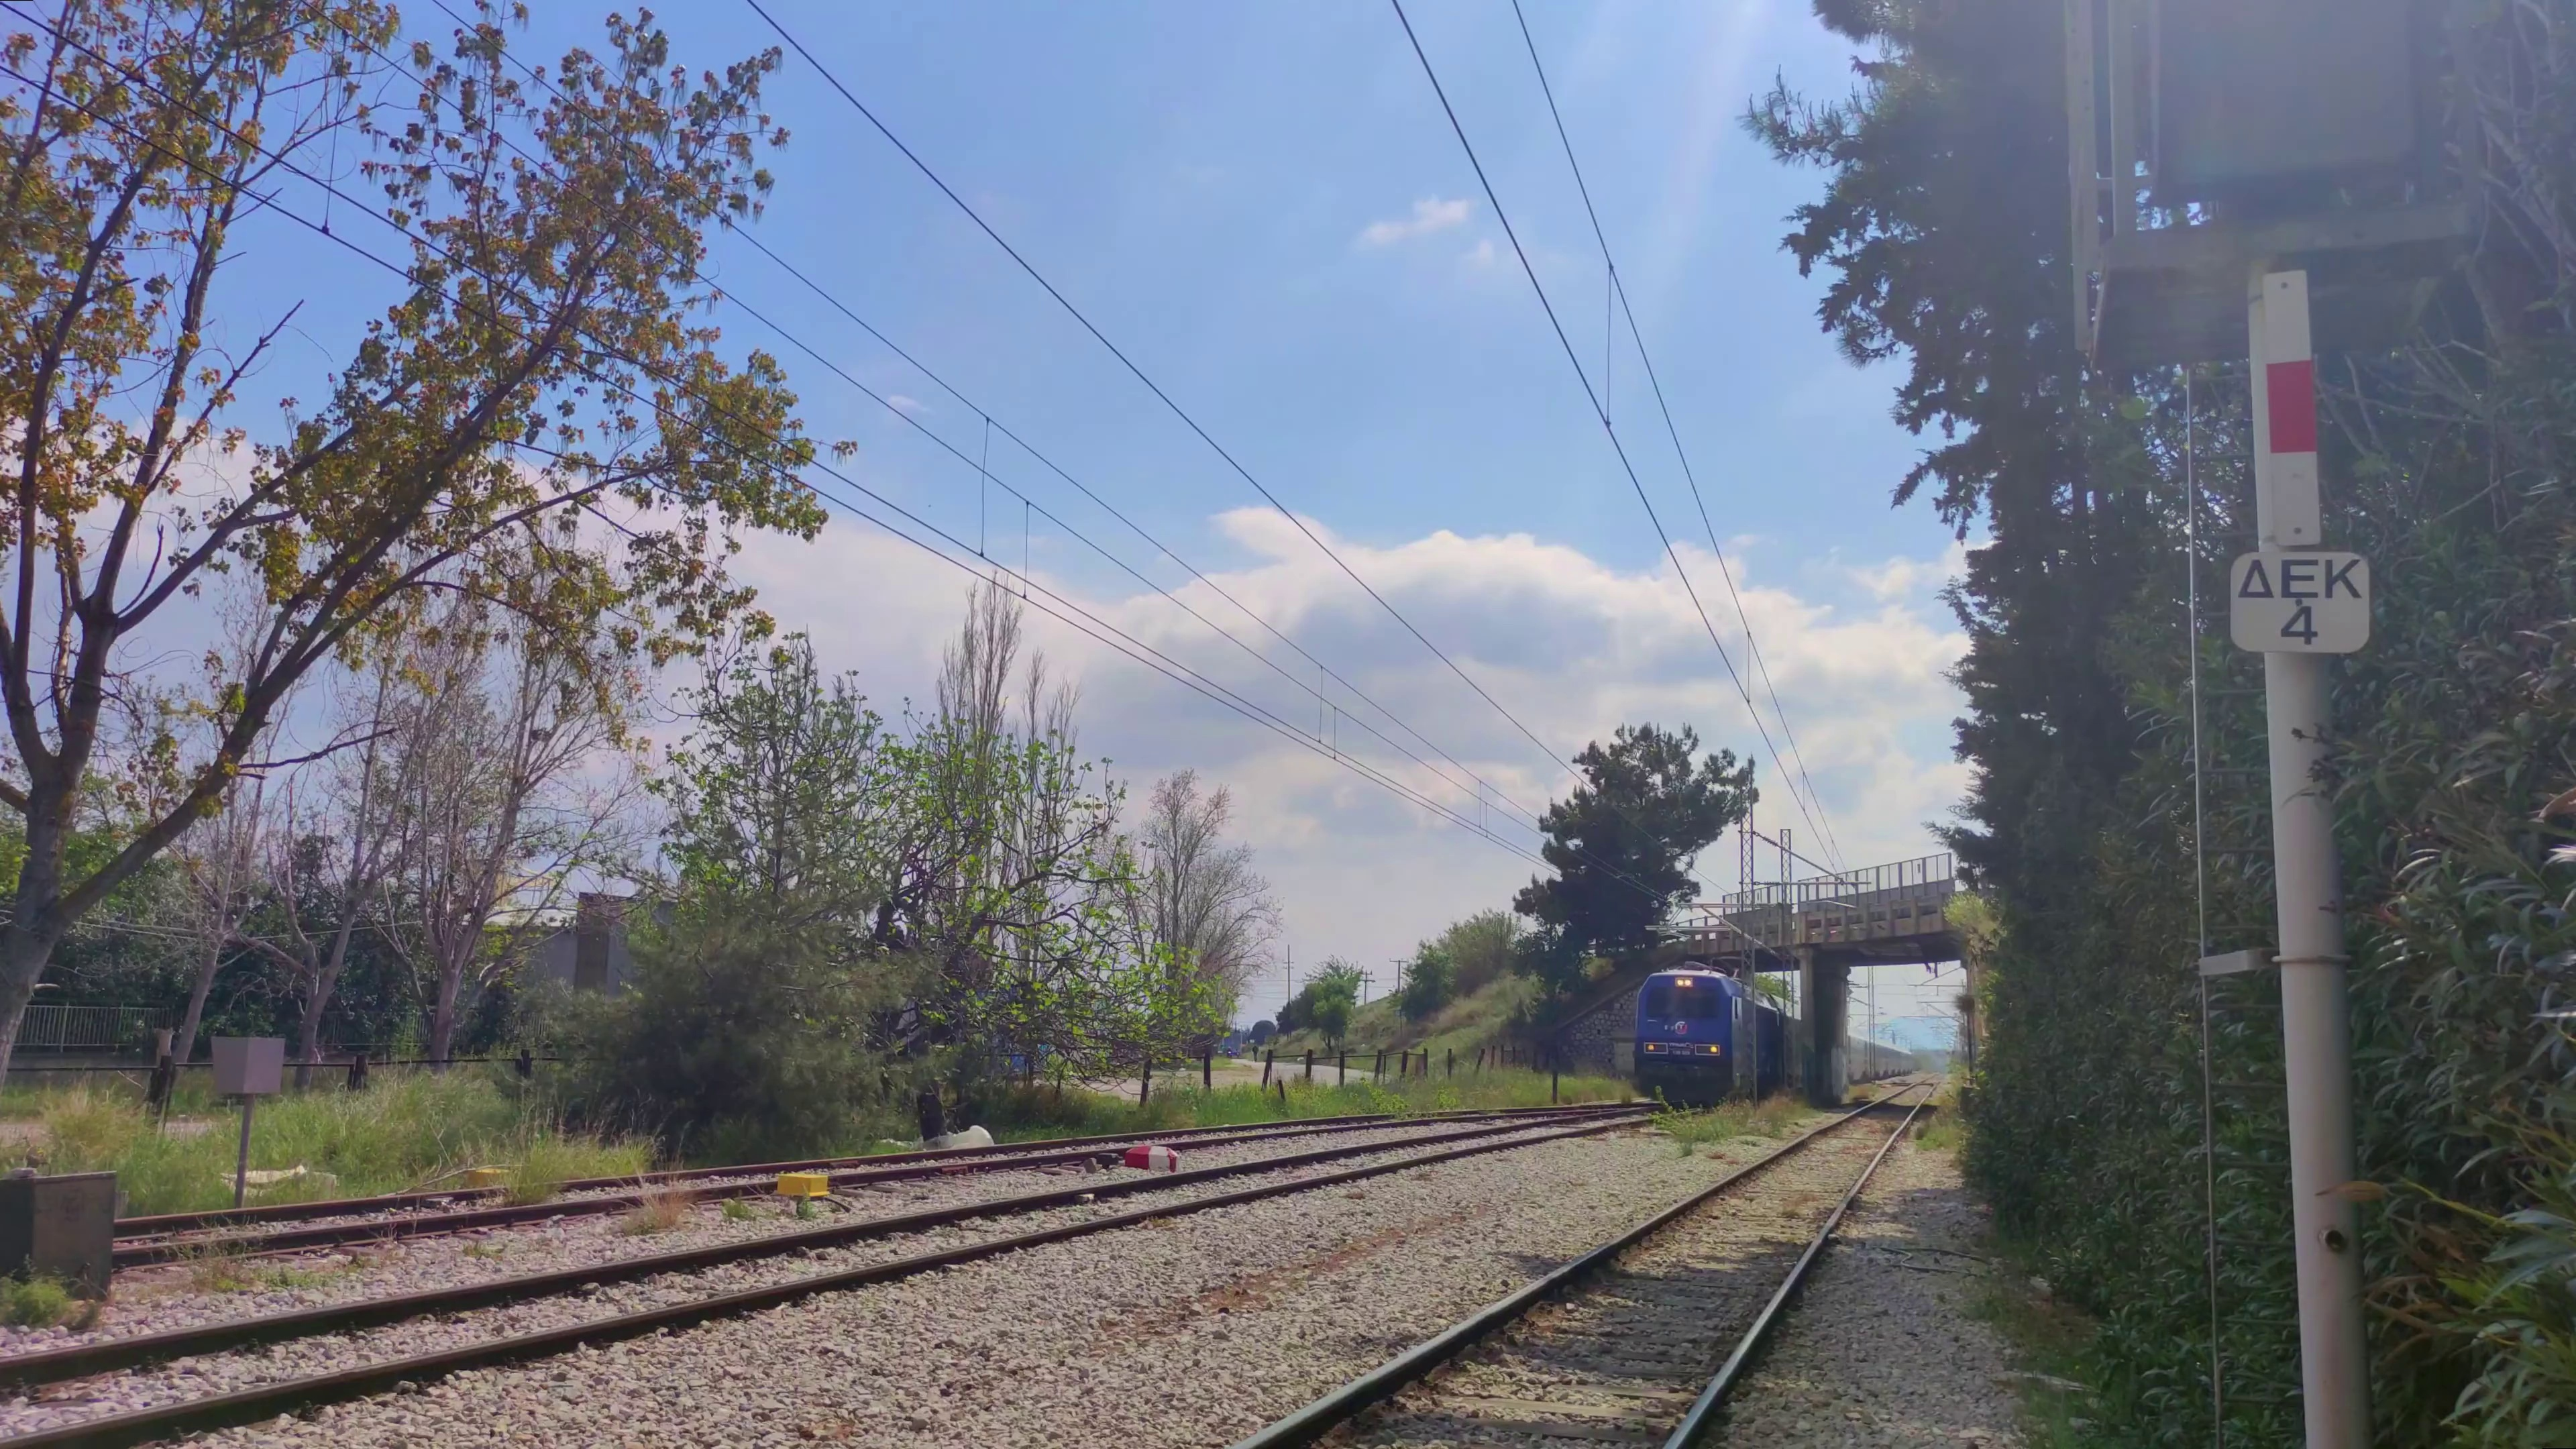}
        \caption{Video 6}
    \end{subfigure}
    
    \vspace{0.5cm}
    
    % Video 7
    \begin{subfigure}[b]{0.3\textwidth}
        \centering
        \includegraphics[width=\textwidth]{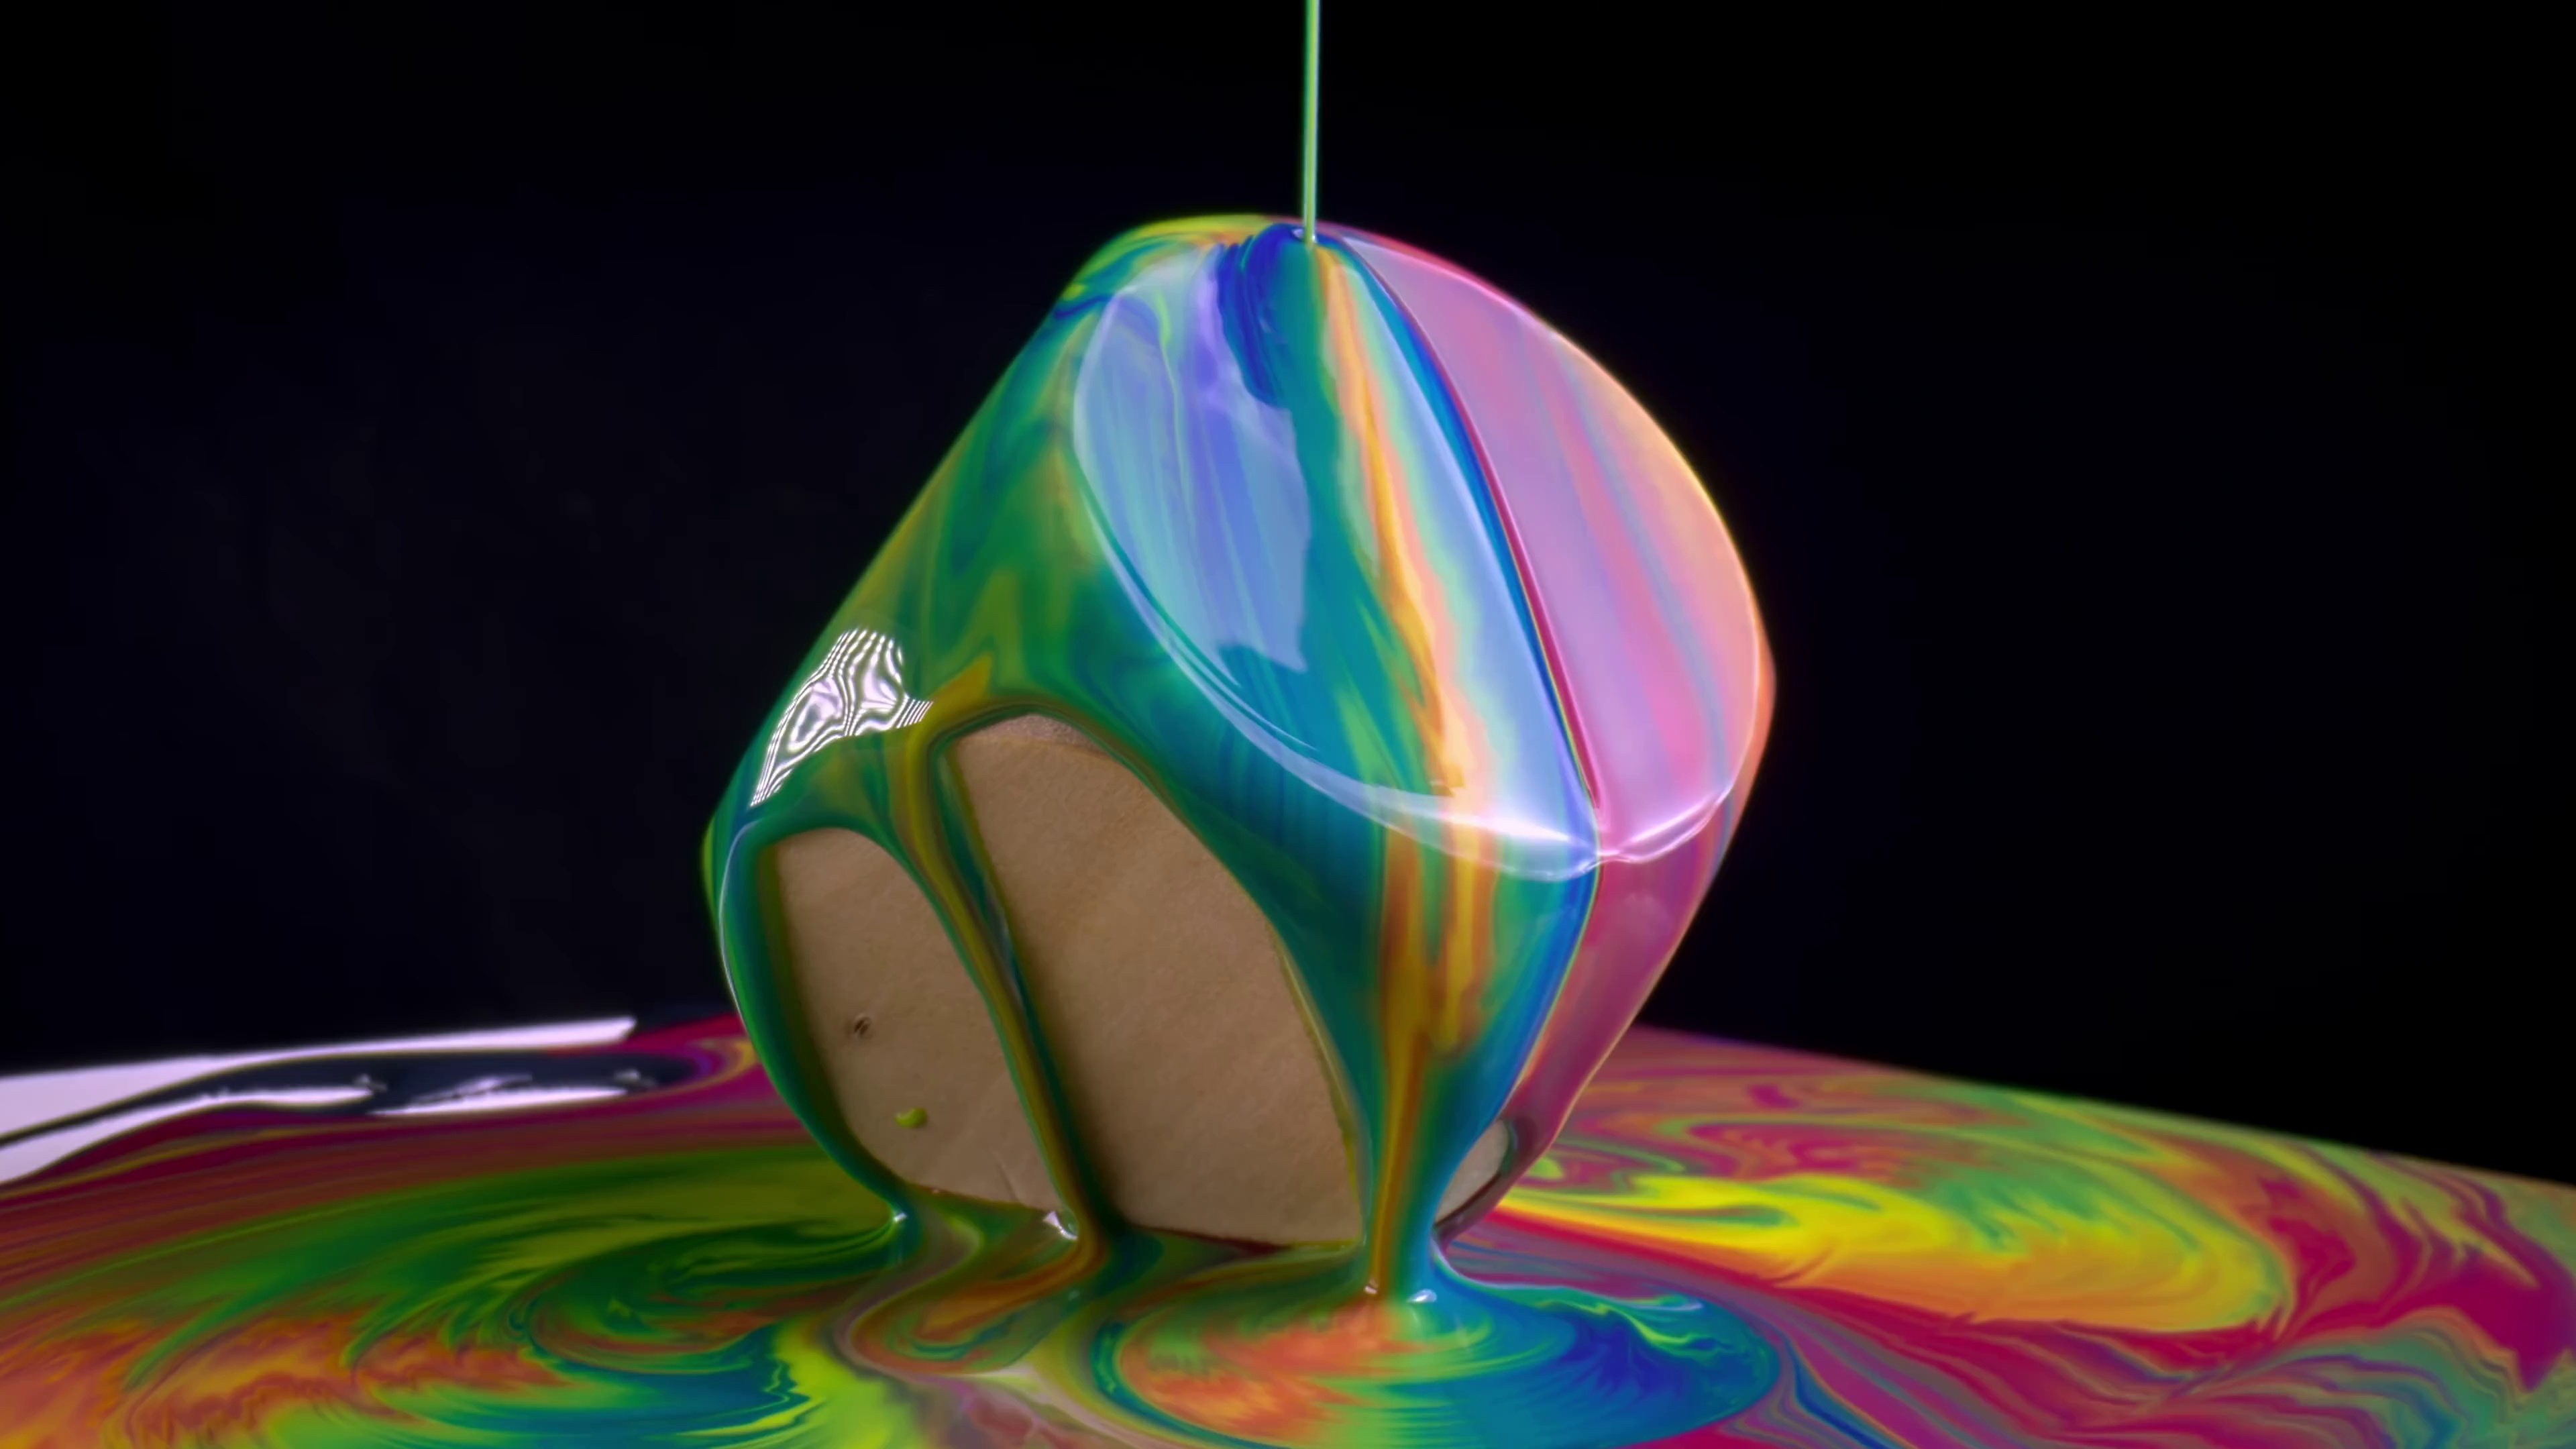}
        \caption{Video 7}
    \end{subfigure}
    % Video 8
    \begin{subfigure}[b]{0.3\textwidth}
        \centering
        \includegraphics[width=\textwidth]{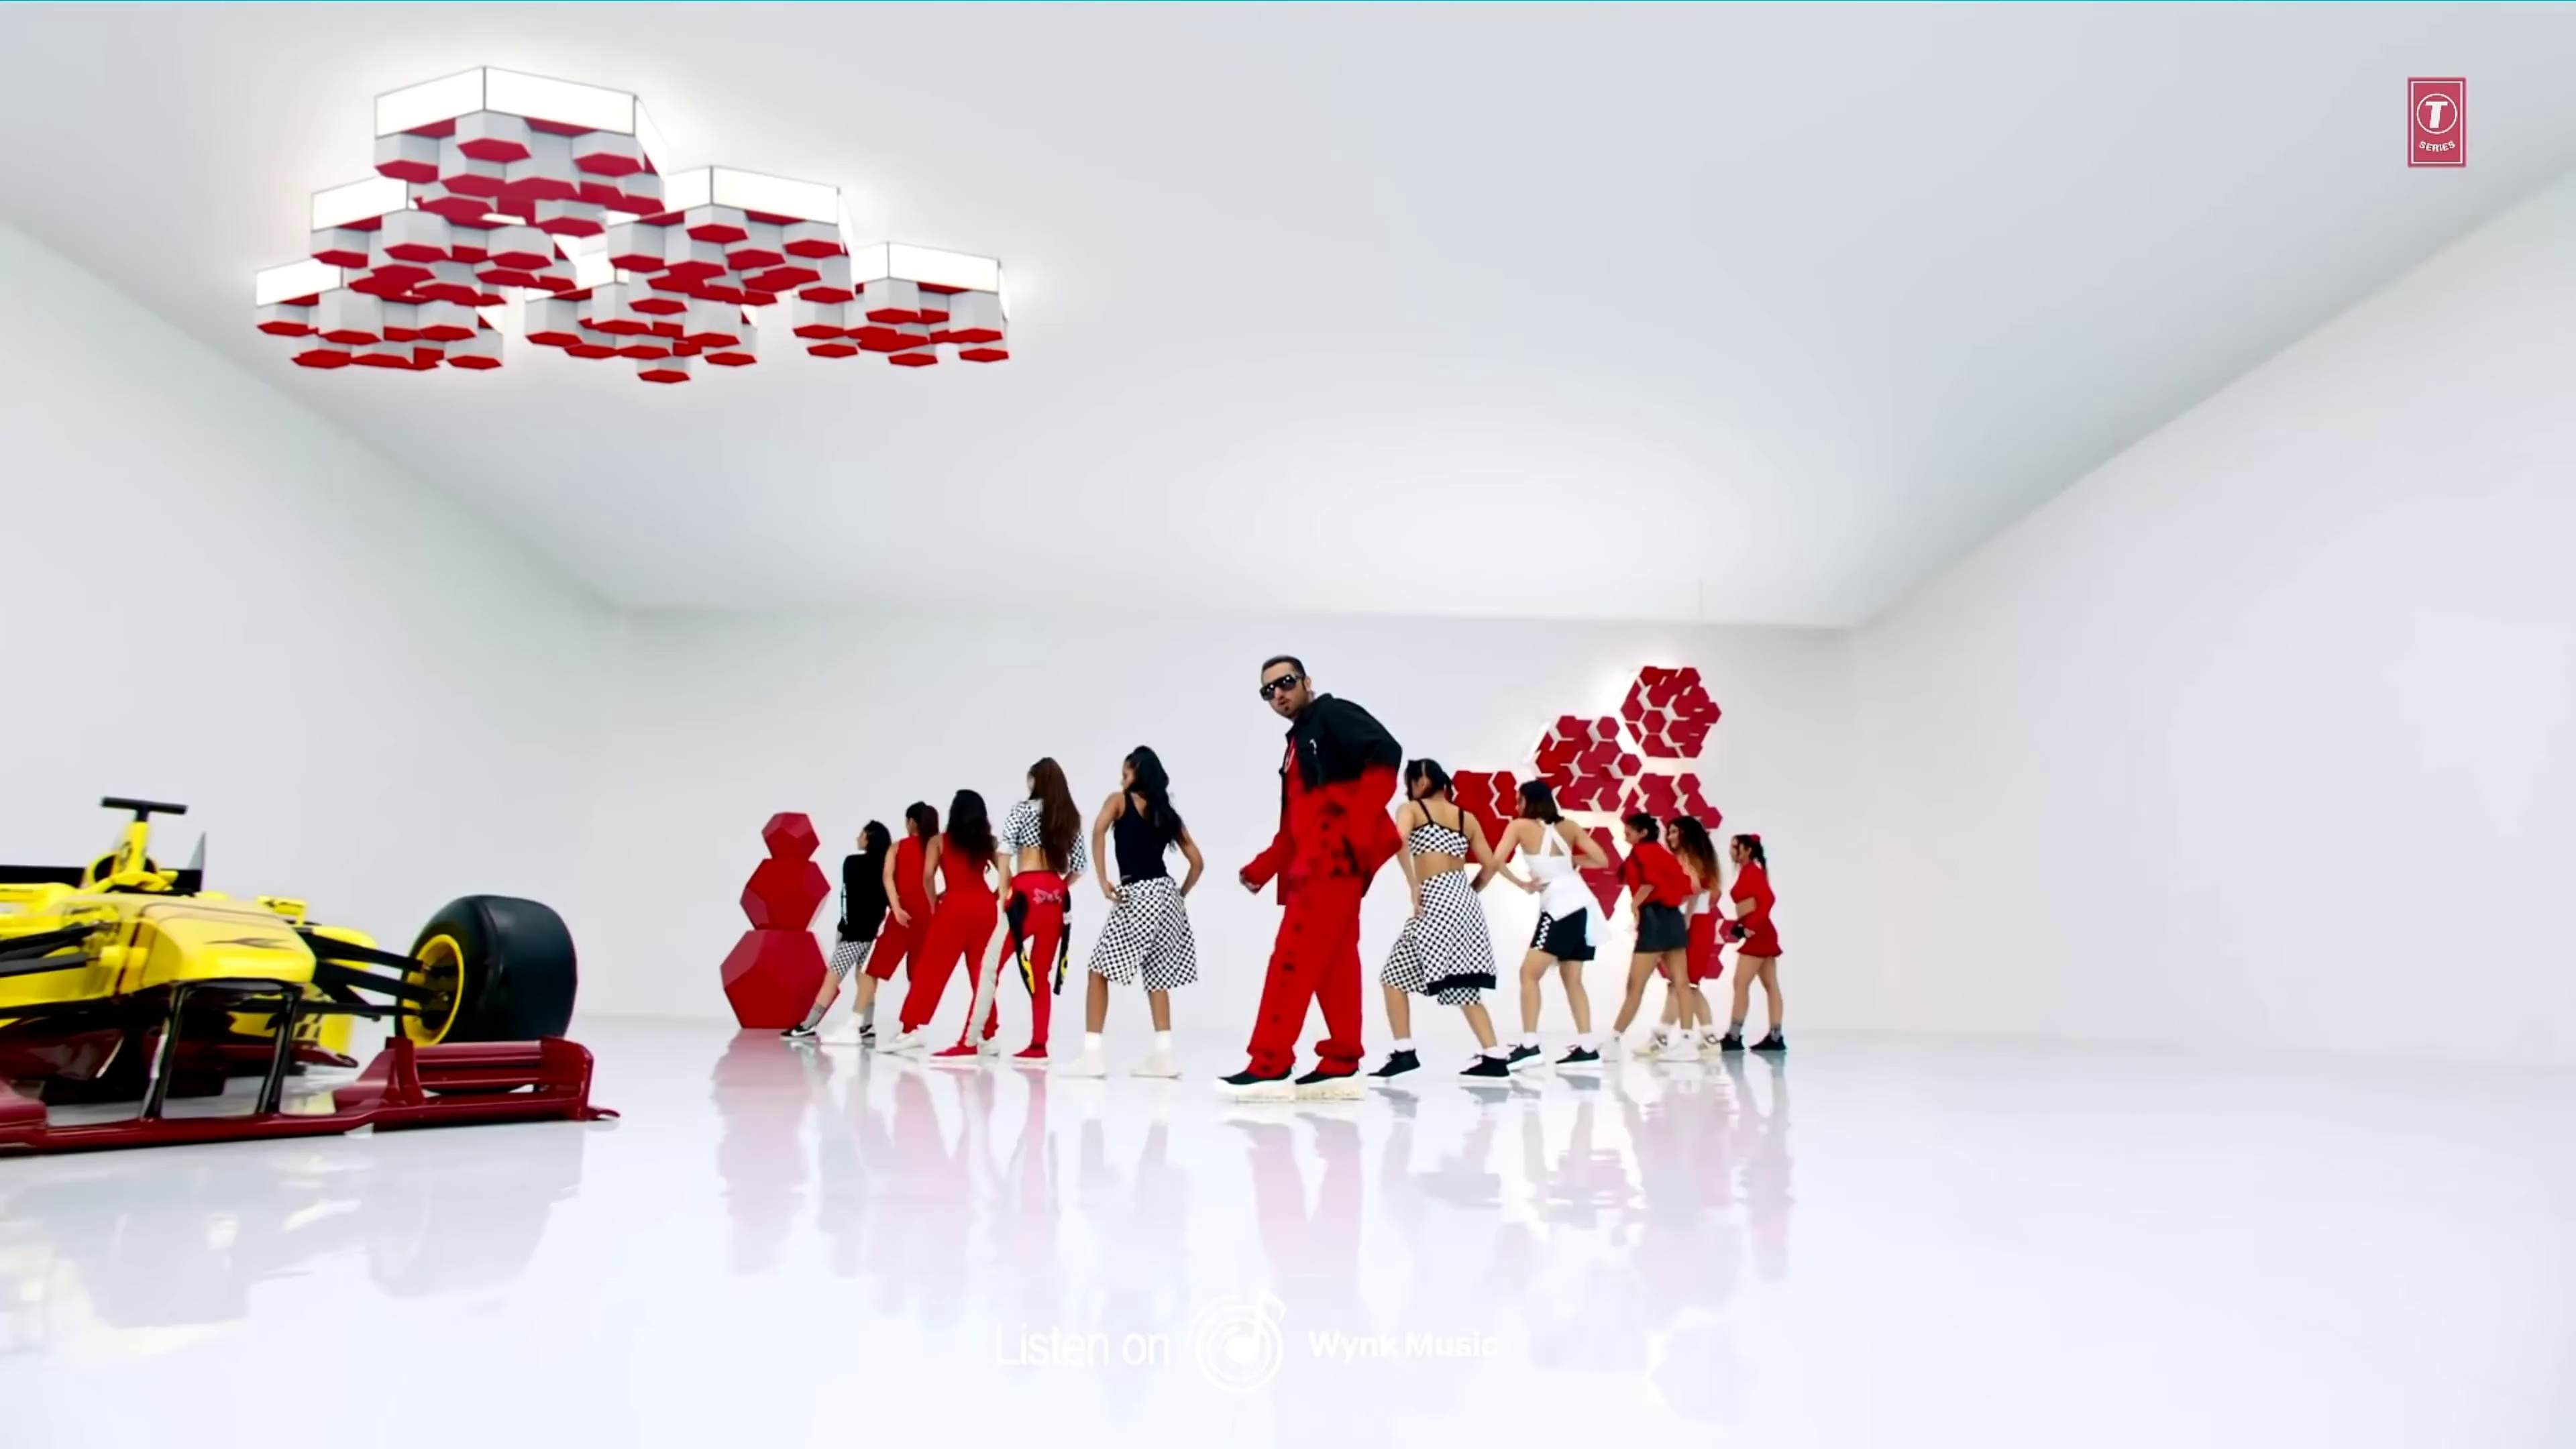}
        \caption{Video 8}
    \end{subfigure}
    % Video 9
    \begin{subfigure}[b]{0.3\textwidth}
        \centering
        \includegraphics[width=\textwidth]{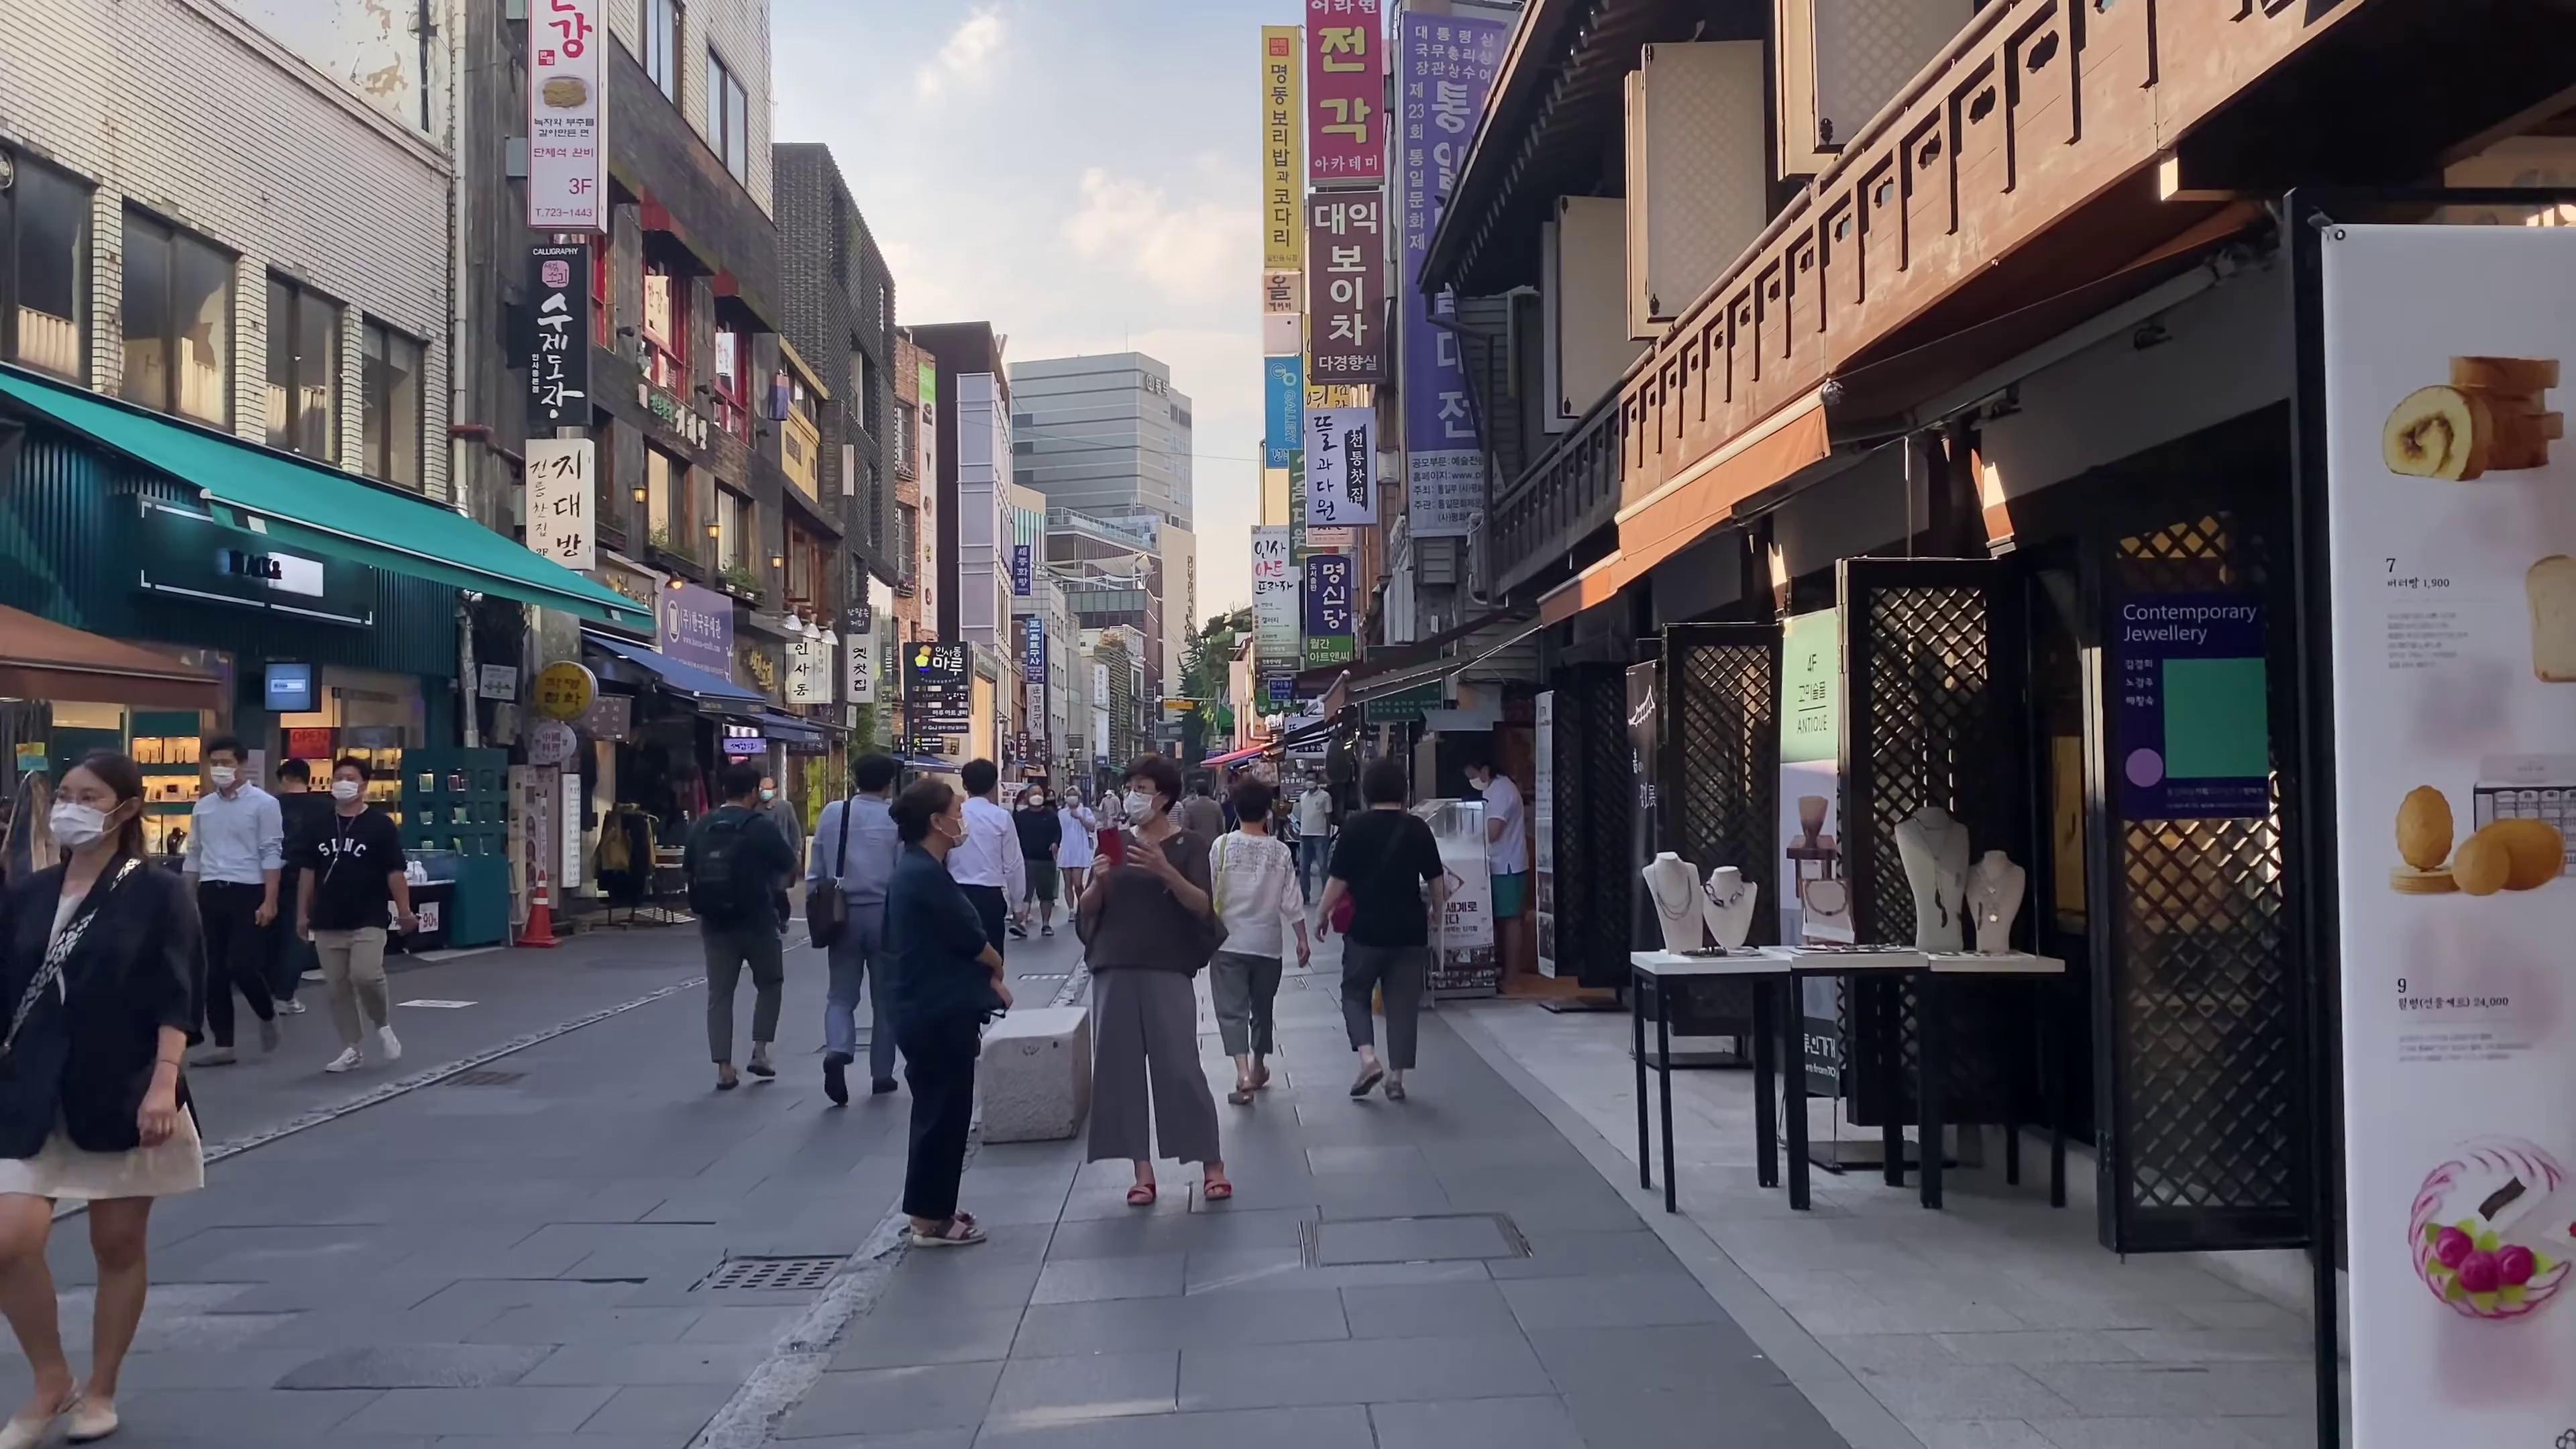}
        \caption{Video 9}
    \end{subfigure}

    \vspace{0.5cm}
    
    % Video 10
    \begin{subfigure}[b]{0.3\textwidth}
        \centering
        \includegraphics[width=\textwidth]{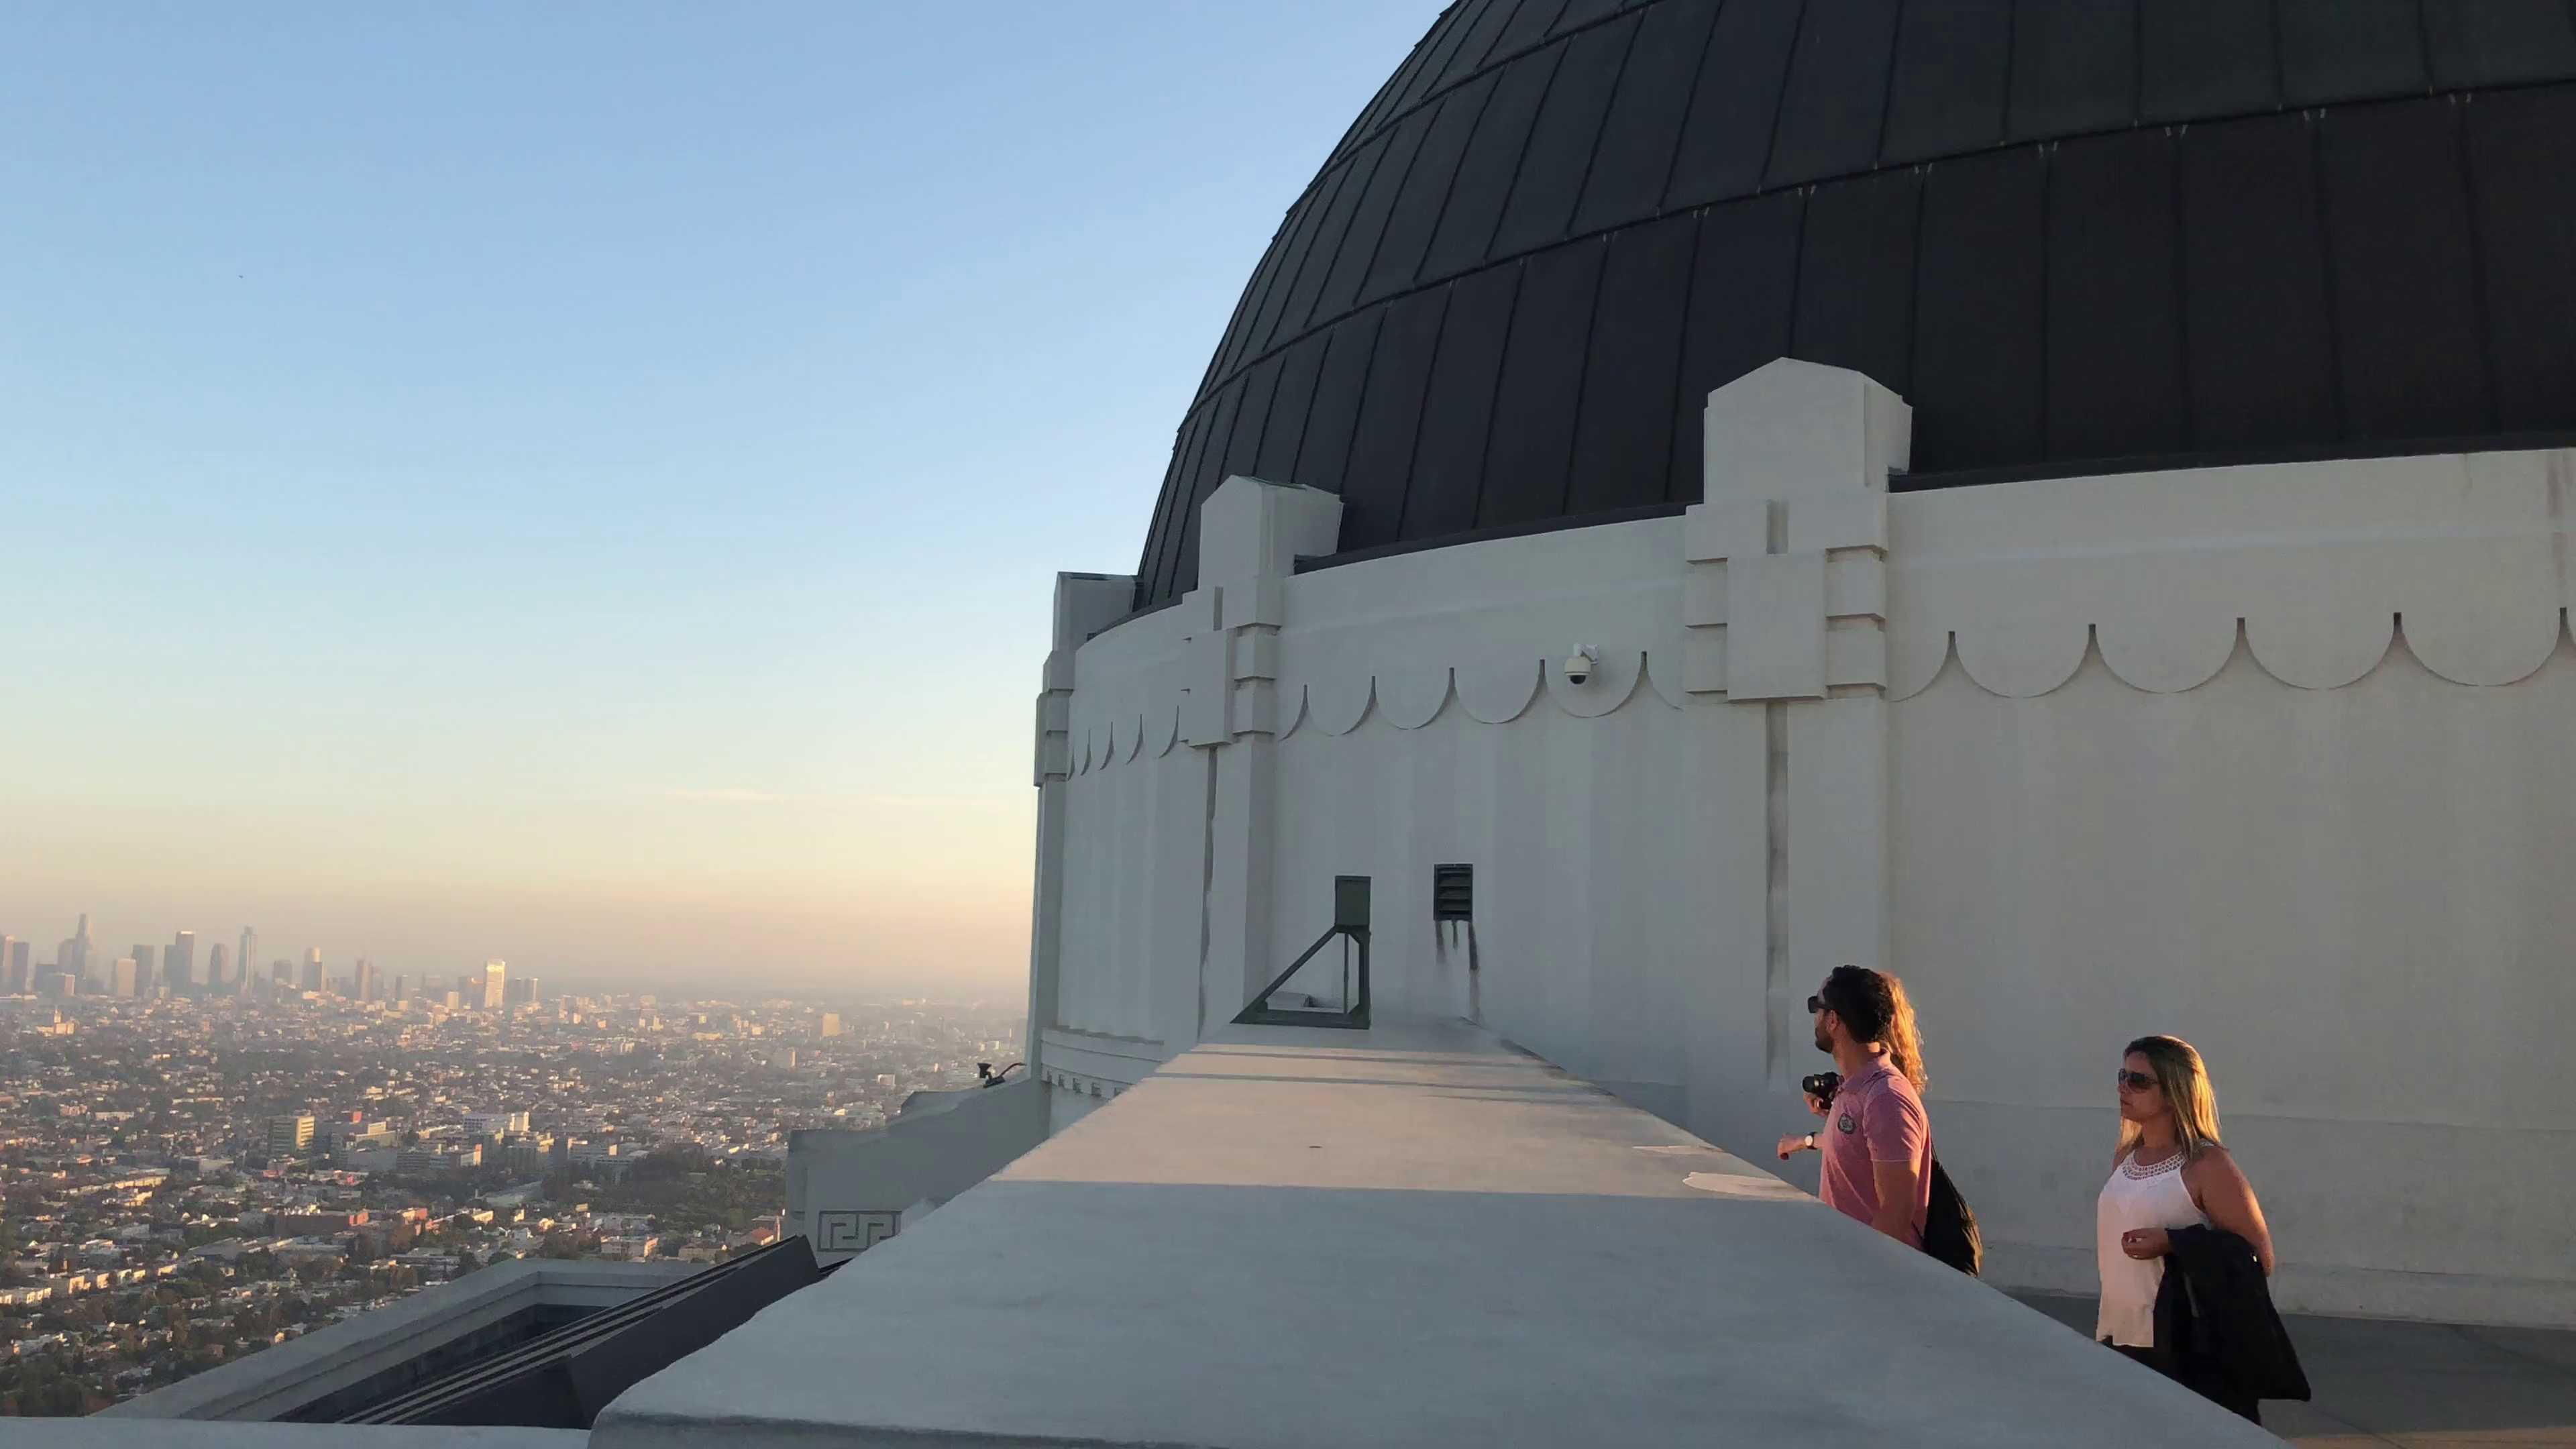}
        \caption{Video 10}
    \end{subfigure}

    \caption{\textbf{Examples of video frames from Video 1 to Video 10 used in the evaluation.}}
    \label{fig:video_examples}
\end{figure*}

\subsection{Training and Evaluation Details}
We extract distortion-related features from 20 randomly cropped patches, each with a resolution of \(384 \times 384\). The same patch positions are used across all frames within each video. During training, a single patch selected randomly from these 20 is processed through the diffusion feature extractor to capture the distortion-related features. In contrast, for inference, all 20 patches are processed to extract these features, which are then input into the downstream VQA network. The final video quality score is calculated by averaging the output scores from these 20 patches. The diffusion feature extractor comprises 1,699 million parameters, with only 363 million trainable parameters attributed to the Controller module. The VQA model itself contains an additional 95.29 million parameters. In terms of computational efficiency, the inference time for the diffusion feature extractor is 1.03 seconds per frame, while the VQA model processes each input in 0.807 seconds on a single Nvidia V100 GPU. Regarding computational complexity, the diffusion feature extractor requires 130.63 GFLOPs, whereas the VQA model demands 92.23 GFLOPs.

Some results presented in Tables 1 through 5 of the main paper are sourced from~\cite{wu2022disentangling,wu2023towards,lu2024kvq, liu2024scaling,mi2024clif,wu2023q}. Moreover, in Figure 7 of the main paper, we showcase t-SNE results highlighting semantic and distortion representations from ViT-L/16 and the diffusion feature extractor. To complement these results, \figref{fig:distortion_examples} and \figref{fig:video_examples} provide representative examples.

\subsection{Evaluation Metrics}
In our evaluation, we employ two metrics to assess the performance of our model: Spearman's Rank-Order Correlation Coefficient (SRCC) and Pearson's Linear Correlation Coefficient (PLCC).

PLCC evaluates the degree of linear correlation between the predicted and ground truth quality scores. It measures how closely the predictions align with the true values on a linear scale, making it sensitive to numerical differences. 

SRCC, on the other hand, assesses the monotonic relationship between two datasets, focusing on the rank order of the data rather than their actual values. This makes SRCC robust to outliers and skewed distributions. Both metrics produce values ranging from $-1$ to $1$, where a score of $1$ signifies perfect correlation, $-1$ indicates perfect inverse correlation, and $0$ reflects no correlation. Higher absolute values for these metrics indicate better model performance, with positive values demonstrating strong agreement with the ground truth.

For PLCC, let $s_i$ and $\hat{s}_i$ denote the ground truth and predicted quality scores for the $i$-th image, respectively. Let $\mu_{s_i}$ and $\mu_{\hat{s}_i}$ represent their respective means, and $N$ the total number of test images. PLCC is defined as:
\begin{equation}
    \operatorname{PLCC} =\frac{\sum^{N}_{i=1}(s_i-\mu_{s_i})(\hat{s}_i-\mu_{\hat{s}_i})}{\sqrt{\sum^{N}_{i=1}(s_i-\mu_{s_i})^{2}}\sqrt{\sum^{N}_{i=1}(\hat{s}_i-\mu_{\hat{s}_i})^{2}}}.
\end{equation}

For SRCC, let $d_i$ represent the rank difference between the ground truth and predicted scores for the $i$-th test image. SRCC is calculated as:
\begin{equation}
    \operatorname{SRCC} =1-\frac{6\sum^{N}_{i=1}d^2_i}{N(N^2-1)}.
\end{equation}

Both metrics provide complementary insights into the model's performance, with higher values indicating greater accuracy and consistency with human judgments.
